# Supplementary material for: Inherent-State Melting and the Onset of Glassy Dynamics in Two-Dimensional Supercooled Liquids
Source: arXiv:2204.07528 ancillary file (2022-04-15)
Supplement: Supplementary file 1 [file SM_OnsetTemperature.pdf]

# Supplemental Material

## Inherent-State Melting and the Onset of Glassy Dynamics in Two-Dimensional Supercooled Liquids

Dimitrios Fraggedakis<sup>1,†</sup>,      Muhammad R. Hasyim<sup>1,‡</sup>      Kranthi K. Mandadapu<sup>1,2,\*</sup>

<sup>1</sup>Department of Chemical & Biomolecular Engineering, University of California, Berkeley, CA, USA 94720

<sup>2</sup>Chemical Sciences Division, Lawrence Berkeley National Laboratory, Berkeley, CA, USA 94720

### Contents

|                                                                                        |           |
|----------------------------------------------------------------------------------------|-----------|
| <b>Preface</b>                                                                         | <b>ii</b> |
| <b>1 Statistical Mechanics of Excitations in Supercooled Liquids</b>                   | <b>1</b>  |
| 1.1 Isoconfigurational Ensemble of Inherent-State Jumps . . . . .                      | 1         |
| 1.2 Building a Grand Canonical Ensemble of Excitations . . . . .                       | 4         |
| 1.3 Application to Non-Interacting Excitations . . . . .                               | 10        |
| <b>2 Elasticity Theory of Defects in Two Dimensions</b>                                | <b>11</b> |
| 2.1 Incompatibility Strain Fields and Stress Functions . . . . .                       | 11        |
| 2.2 Elastic Defects as Geometric ‘Charges’ . . . . .                                   | 13        |
| 2.3 Variational Principles and Boundary Conditions . . . . .                           | 19        |
| 2.4 Conservation Laws for Geometric Charges . . . . .                                  | 20        |
| 2.5 Airy Stress Function Fundamental Solutions . . . . .                               | 22        |
| <b>3 Energy–Entropy Arguments and Interaction Energies</b>                             | <b>23</b> |
| 3.1 Free Energy Arguments for Geometric Charges . . . . .                              | 23        |
| 3.2 Interaction Energy for a System of Geometric Dipoles . . . . .                     | 27        |
| 3.3 Mapping Bound-Dipole Pairs to Pure-Shear Excitations . . . . .                     | 30        |
| 3.4 Grand Canonical Partition Function for Geometric Dipoles . . . . .                 | 32        |
| <b>4 Elastic Constants and Fluctuation Formulas</b>                                    | <b>33</b> |
| 4.1 The Binding-Unbinding Transition as an Inherent-State Melting Transition . . . . . | 34        |
| 4.2 Strain Formula for a System of Dipoles . . . . .                                   | 37        |
| <b>5 Renormalization Group (RG) Analysis of Geometric Dipoles</b>                      | <b>39</b> |
| 5.1 The Idea of RG and Fugacity Expansion . . . . .                                    | 39        |
| 5.2 Deriving the RG Equations . . . . .                                                | 50        |
| 5.3 Analysis of the RG Equations . . . . .                                             | 58        |
| 5.4 Atomistic Models of Glass Formers and RG Calculations of Elastic Moduli . . . . .  | 63        |
| 5.5 Mean-Squared Displacement and Density–Density Correlations . . . . .               | 65        |
| <b>References</b>                                                                      | <b>72</b> |

---

<sup>†</sup> dimfraged@gmail.com    <sup>‡</sup> muhammad\_hasyim@berkeley.edu    <sup>\*</sup> kranthi@berkeley.edu

## Preface

This Supplemental Material (SM) is an accompaniment to the main text, detailing all derivation steps for the theory of onset temperature  $T_o$  proposed in this work. The SM is written in a self-contained manner, and as such, there are sections containing review material. Here, we provide a brief overview of each section to allow readers to decide which section may be skipped or not:

- In Section 1, we establish the thermodynamic framework for studying excitations in the supercooled liquid. This section contains new material detailing the derivation of a grand canonical partition function  $\Xi_{\text{exc}}$  for excitations, Eq. (1.51), from the concept of an isoconfigurational ensemble [1] of inherent-state jumps, i.e., hopping events between energy-minimizing configurations of the potential energy landscape. For an ideal gas of excitations, the framework predicts a concentration of excitations, Eq. (1.56), consistent with dynamical facilitation (DF) theory [2].
- In Section 2, we overview the basics of linear elasticity under the presence of defects in two dimensions. In particular, we review the work of Moshe and co-workers [3, 4] where elastic defects are modeled as geometric ‘charges’ (monopoles, Eq. (2.30), dipoles, Eq. (2.41), quadrupoles, Eq. (2.48)), in analogy to electrostatics. This review also includes discussions on admissible boundary conditions, Eqs. (2.59) and (2.60), via variational principles, conservation laws applicable to the geometric charges, and Green’s function solutions for monopoles, dipoles and quadrupoles, Eqs. (2.74), (2.77) and (2.79), respectively.
- In Section 3, we determine which type of geometric charges can be used as the fundamental units of excitations. We use energy-entropy arguments similar to the ones used by Kosterlitz & Thouless [5, 6] to establish a binding-unbinding transition for geometric dipoles that may be associated with the onset temperature  $T_o$ . Taking dipoles as the excitations, we derive their interaction energy, Eq. (3.28) to prepare a more careful analysis of this transition. This section also contains new material where we map bound-dipole pairs to localized pure-shear excitations, which were originally proposed in Ref. [7] to connect dynamical excitations from DF theory to inherent structure and elasticity. We end this section by applying the grand canonical partition function  $\Xi_{\text{exc}}$  in Eq. (1.51) to a many-dipole system, Eq. (3.60).
- In Section 4, we explain how the binding-unbinding transition can be understood as an excitation-mediated inherent-state melting transition, in analogy to dislocation-mediated melting found in the Kosterlitz-Thouless-Halperin-Nelson-Young (KTHNY) theory [5, 6, 8–11]. To study the binding-unbinding transition as a melting transition, we derive the formulas for the elastic moduli, Eqs. (4.18)–(4.20), that accounts for both harmonic and excitation-induced strain fluctuations. The transition is then determined by the point at which the elastic moduli vanish. In addition, we derive a formula for the strain due to dipolar excitations, Eq. (4.27).
- In Section 5, we apply the renormalization group (RG) procedure to compute the elastic moduli in Eqs. (4.18)–(4.20) following closely the analysis in the KTHNY theory with minor differences. Expert readers who are familiar with the RG in the KTHNY theory may skip the majority of this section. However, Section 5.4 provides new material where we show the results of the RG calculations on the atomistic models of glass formers used in this work. In addition, we show in Section 5.5 how an effective Gaussian field theory of elastic fluctuations, based on the RG analysis, describes the response of a supercooled liquid at short intermediate timescales. The results are consistent with recent observations on the Mermin-Wagner fluctuations found in simulations and experiments of two-dimensional glass formers [12–16].

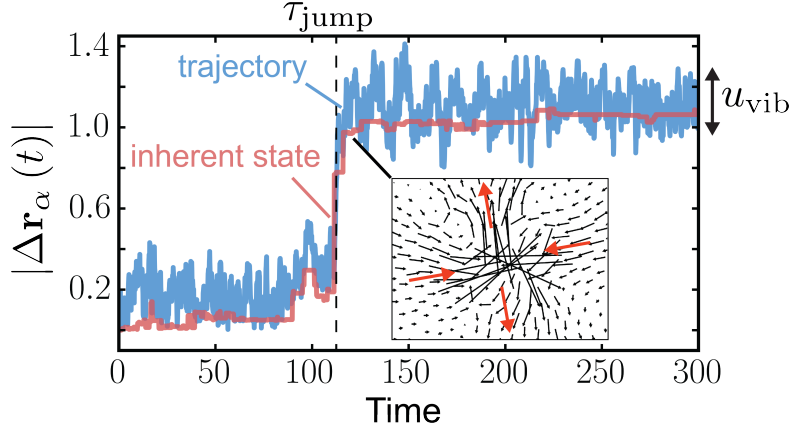

Figure S.1: The trajectory of a single particle at  $T = 0.137 < T_o$  for Poly-(12,0) compared with its inherent-state (IS) trajectory, at the intermediate timescales indicated by Eq. (1.2), with an inset showing a sample of the pure-shear excitation.

## 1 Statistical Mechanics of Excitations in Supercooled Liquids

In this section, we derive the partition function corresponding to a thermodynamic ensemble of excitations in supercooled liquids. In Section 1.1, the isoconfigurational ensemble is introduced to study inherent-state jumps at intermediate timescales. In Section 1.2, the partition function for an ensemble of excitations is derived from the partition function of the isoconfigurational ensemble. We then apply the framework to a system of non-interacting excitations in Section 1.3, demonstrating the Arrhenius law for the concentration of excitations and the role of entropy in driving inherent-state jumps.

### 1.1 Isoconfigurational Ensemble of Inherent-State Jumps

We begin by considering the supercooled liquid as a system of  $N$ -many particles in  $d$ -dimensions, whose configuration at time  $t$  is denoted as  $\{\mathbf{r}^\alpha(t)\}_{\alpha=1}^N \equiv \{\mathbf{r}^\alpha(t)\}$ , where  $\mathbf{r}^\alpha$  is the position of the  $\alpha$ -th particle. The corresponding inherent-state configuration  $\{\mathbf{R}^\alpha(t)\}_{\alpha=1}^N \equiv \{\mathbf{R}^\alpha(t)\}$  is obtained by locally minimizing the potential energy  $U(\{\mathbf{r}^\alpha\})$  starting from  $\{\mathbf{r}^\alpha(t)\}$ , i.e.,

$$-\left. \frac{\partial U(\{\mathbf{r}^\alpha\})}{\partial \mathbf{r}^\alpha} \right|_{\{\mathbf{R}^\alpha\}} \equiv \mathbf{F}^\alpha(\{\mathbf{R}^\alpha\}) = 0 \quad (1.1)$$

and  $\mathbf{F}^\alpha(\{\mathbf{r}^\alpha\})$  is the total force acting on the  $\alpha$ -th particle. As seen from Fig. S.1, the inherent-state trajectory coarse grains the vibrational motion of the particle and captures how the particle jumps from one initial position to the next. Since excitation events correspond to inherent-state jumps [7], we can study the statistical mechanics of excitations by considering motion within the following intermediate timescales:

$$\tau_{\text{vib}}(T) \ll t \sim \langle \tau_{\text{jump}}(T) \rangle \ll \tau_{\text{eq}}(T), \quad (1.2)$$

where  $\tau_{\text{vib}}(T)$  is the characteristic timescale for vibrational motion,  $\langle \tau_{\text{jump}}(T) \rangle$  is the average time needed for the system to jump from any initial inherent state to all possible nearest-neighboring inherent states, and  $\tau_{\text{eq}}(T)$  is the equilibrium relaxation time. Figure S.1 shows, in particular, how these intermediate timescales correlate with the initiation of the first hopping event.

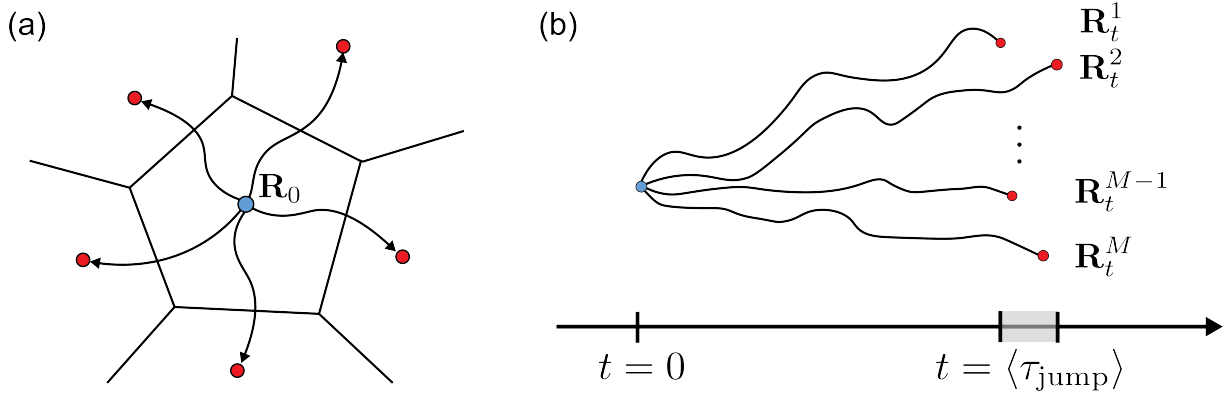

Figure S.2: (a) Illustration of inherent-state jumps in configuration space, that are obtained via the isoconfigurational ensemble. (b) An illustration of trajectories initiated by the isoconfigurational ensemble. The final configurations at  $t = \tau_{\text{jump}}$  form the set of all possible nearest neighboring inherent states in the limit of  $M \rightarrow \infty$ .

We can also observe in Fig. S.1 that there are fluctuations in  $\{\mathbf{R}^\alpha(t)\}$  that generate displacements smaller than the average vibrational displacement  $u_{\text{vib}}(T)$  defined as

$$u_{\text{vib}}(T) = \sqrt{\left\langle \frac{1}{Nd} \sum_{\alpha=1}^N |\mathbf{r}^\alpha - \mathbf{R}^\alpha|^2 \right\rangle}, \quad (1.3)$$

where  $\langle \dots \rangle$  is the equilibrium ensemble average. This motivates a criterion of what we define as an inherent-state jump: it is an event where the particle with the largest displacement has moved more than  $u_{\text{vib}}(T)$  in magnitude, or equivalently

$$\max_{1 \leq \alpha \leq N} \{|\Delta \mathbf{R}^\alpha(t)|\} \geq u_{\text{vib}}(T), \quad (1.4)$$

where  $\Delta \mathbf{R}^\alpha(t) = \mathbf{R}^\alpha(t) - \mathbf{R}_0^\alpha$ . For a given trajectory of the system, we can define  $\tau_{\text{jump}}(T)$  as the minimum time needed to satisfy the inequality in Eq. (1.4), i.e.,

$$\tau_{\text{jump}}(T) = \arg \min_{t \in [0, +\infty)} \left\{ \max_{1 \leq \alpha \leq N} \{|\Delta \mathbf{R}^\alpha(t)|\} \geq u_{\text{vib}}(T) \right\}. \quad (1.5)$$

The statistics of inherent-state jumps can be studied by initiating multiple trajectories from the same initial configuration  $\{\mathbf{r}_0^\alpha\}$ . If the system is driven by deterministic Newtonian dynamics, then one equilibrium trajectory can be realized by drawing a random set of initial momenta  $\{\mathbf{p}_0^\alpha\}$  from the Maxwell-Boltzmann distribution. The corresponding inherent-state trajectory then yields a stochastic realization of one inherent-state jump. Repeating this process  $M$ -many times, we can collect the configurations observed at time  $t = \tau_{\text{jump}}(T)$  into a set denoted as

$$\mathcal{S}_M(\{\mathbf{R}_0^\alpha\}) = \left\{ \{\mathbf{R}_m^\alpha(\tau_{\text{jump}}^m)\} \right\}_{m=1}^M, \quad (1.6)$$

where  $\tau_{\text{jump}}^m(T)$  is the jump time associated with the  $m$ -th trajectory,  $\{\mathbf{R}_m^\alpha(t)\}$  is the inherent state from the  $m$ -th trajectory at time  $t$ , and  $\{\mathbf{R}_0^\alpha\}$  is the initial inherent state corresponding to  $\{\mathbf{r}_0^\alpha\}$ . As illustrated in Fig. S.2, the set  $\mathcal{S}_M(\{\mathbf{R}_0^\alpha\})$  forms the isoconfigurational ensemble [1] of nearest-neighboring inherent states that can be reached via excitation events from  $\{\mathbf{R}_0^\alpha\}$ . Given

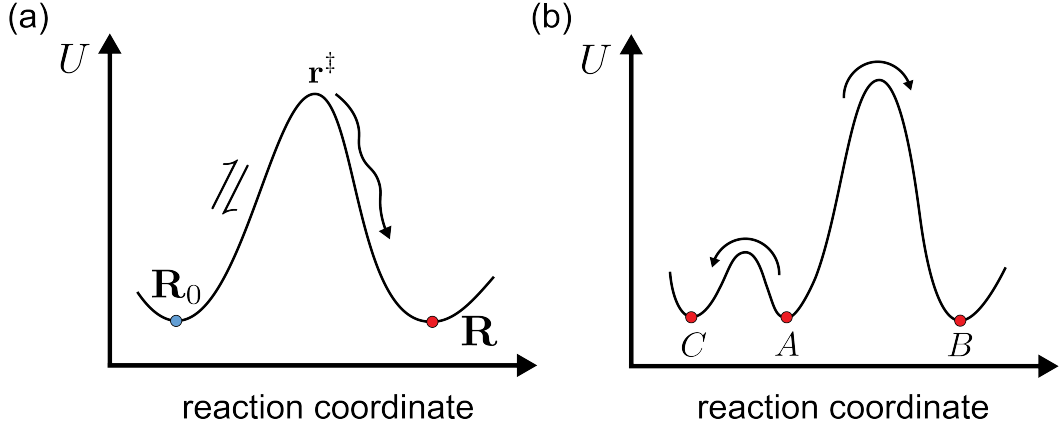

Figure S.3: (a) An illustration of TST as applied to one inherent-state jump. (b) An illustration of how the height of energy barriers determine the jump probabilities between two different inherent states with equal potential energies.

an observable  $A(\{\mathbf{R}^\alpha\}; \{\mathbf{R}_0^\alpha\})$  that depends on both the current and initial configurations, we can compute the isoconfigurational empirical average  $A_{\text{iso}}(M; \{\mathbf{R}_0^\alpha\})$  as

$$A_{\text{iso}}(\{\mathbf{R}_0^\alpha\}; M) = \frac{1}{M} \sum_{\{\mathbf{R}^\alpha\} \in \mathcal{S}_M(\{\mathbf{R}_0^\alpha\})} A(\{\mathbf{R}^\alpha\}; \{\mathbf{R}_0^\alpha\}). \quad (1.7)$$

These observables include elastic fields induced by the inherent-state jumps, such as stress and strain, as well as the number of excitations. The isoconfigurational ensemble average is then obtained by taking the following limit:

$$A_{\text{iso}}(\{\mathbf{R}_0^\alpha\}) = \lim_{M \rightarrow \infty} A_{\text{iso}}(\{\mathbf{R}_0^\alpha\}; M) := \sum_{\{\mathbf{R}^\alpha\} \in \mathcal{B}(\{\mathbf{R}_0^\alpha\})} A(\{\mathbf{R}^\alpha\}; \{\mathbf{R}_0^\alpha\}) p_{\text{iso}}(\{\mathbf{R}^\alpha\}; \{\mathbf{R}_0^\alpha\}), \quad (1.8)$$

where  $\mathcal{B}(\{\mathbf{R}_0^\alpha\})$  is the set of all possible nearest-neighboring inherent states defined as

$$\mathcal{B}(\{\mathbf{R}_0^\alpha\}) = \lim_{M \rightarrow \infty} \mathcal{S}_M(\{\mathbf{R}_0^\alpha\}) \quad (1.9)$$

and  $p_{\text{iso}}(\{\mathbf{R}^\alpha\}; \{\mathbf{R}_0^\alpha\})$  is the probability of observing a jump towards an inherent state  $\{\mathbf{R}^\alpha\} \in \mathcal{B}(\{\mathbf{R}_0^\alpha\})$  given that the system starts at  $\{\mathbf{R}_0^\alpha\}$ .

The form of  $p_{\text{iso}}(\{\mathbf{R}^\alpha\}; \{\mathbf{R}_0^\alpha\})$  is obtained from transition-state theory (TST) [17, 18]. As illustrated in Fig. S.3(a), TST assumes that every jump proceeds by establishing an equilibrium between the ‘reactant’ state  $\{\mathbf{R}_0^\alpha\}$  and transition state  $\{\mathbf{R}^\alpha\}^\ddagger$ , and then the ‘product’ state  $\{\mathbf{R}^\alpha\}$  is reached by crossing the transition state exactly once. This implies that  $p_{\text{iso}}(\{\mathbf{R}^\alpha\}; \{\mathbf{R}_0^\alpha\})$  is set by the probability to reach the transition state  $p^\ddagger(\{\mathbf{R}^\alpha\}^\ddagger; \{\mathbf{R}_0^\alpha\})$ . In other words,

$$p_{\text{iso}}(\{\mathbf{R}^\alpha\}; \{\mathbf{R}_0^\alpha\}) = p^\ddagger(\{\mathbf{R}^\alpha\}^\ddagger; \{\mathbf{R}_0^\alpha\}) \sim e^{-\beta \Delta U(\{\mathbf{R}^\alpha\}^\ddagger; \{\mathbf{R}_0^\alpha\})}, \quad (1.10)$$

where  $\Delta U(\{\mathbf{R}^\alpha\}^\ddagger; \{\mathbf{R}_0^\alpha\}) = U(\{\mathbf{R}^\alpha\}^\ddagger) - U(\{\mathbf{R}_0^\alpha\})$  is the transition-state energy barrier. The normalization factor  $Q_{\text{iso}}(\{\mathbf{R}_0^\alpha\})$  of Eq. (1.10) over all possible  $\{\mathbf{R}^\alpha\} \in \mathcal{B}(\{\mathbf{R}_0^\alpha\})$  is the partition function associated with the isoconfigurational ensemble and is written as

$$Q_{\text{iso}}(\{\mathbf{R}_0^\alpha\}) = \sum_{\{\mathbf{R}^\alpha\} \in \mathcal{B}(\{\mathbf{R}_0^\alpha\})} e^{-\beta \Delta U(\{\mathbf{R}^\alpha\}^\ddagger; \{\mathbf{R}_0^\alpha\})}, \quad (1.11)$$

and Eq. (1.8) becomes

$$A_{\text{iso}}(\{\mathbf{R}_0^\alpha\}) = \frac{1}{Q_{\text{iso}}(\{\mathbf{R}_0^\alpha\})} \sum_{\{\mathbf{R}^\alpha\} \in \mathcal{B}(\{\mathbf{R}_0^\alpha\})} A(\{\mathbf{R}^\alpha\}; \{\mathbf{R}_0^\alpha\}) e^{-\beta \Delta U(\{\mathbf{R}^\alpha\}^\ddagger)}. \quad (1.12)$$

Since the partition function in Eq. (1.11) depends only on potential-energy differences, Eq. (1.11) provides us a thermodynamic framework to study the inherent-state jumps. In particular, we can define the free energy of the isoconfigurational ensemble as

$$F_{\text{iso}}(\{\mathbf{R}_0^\alpha\}) := -k_B T \ln Q_{\text{iso}}(\{\mathbf{R}_0^\alpha\}). \quad (1.13)$$

This free energy is related to the free-energy difference between all possible transition states and the reactant state. To see this, we can re-express Eq. (1.11) as

$$Q_{\text{iso}}(\{\mathbf{R}_0^\alpha\}) = \sum_{\{\mathbf{R}^\alpha\} \in \mathcal{B}(\{\mathbf{R}_0^\alpha\})} e^{-\beta(U(\{\mathbf{R}^\alpha\}^\ddagger) - U(\{\mathbf{R}_0^\alpha\}))} = \left( \sum_{\{\mathbf{R}^\alpha\} \in \mathcal{B}(\{\mathbf{R}_0^\alpha\})} e^{-\beta U(\{\mathbf{R}^\alpha\}^\ddagger)} \right) e^{\beta U(\{\mathbf{R}_0^\alpha\})} \quad (1.14)$$

and defining  $F^\ddagger(\{\mathbf{R}_0^\alpha\}) = -k_B T \ln \left( \sum_{\{\mathbf{R}^\alpha\} \in \mathcal{B}(\{\mathbf{R}_0^\alpha\})} e^{-\beta U(\{\mathbf{R}^\alpha\}^\ddagger)} \right)$  as the free-energy of the collection of transition states, so that Eq. (1.13) can be written as

$$F_{\text{iso}}(\{\mathbf{R}_0^\alpha\}) = F^\ddagger(\{\mathbf{R}_0^\alpha\}) - U(\{\mathbf{R}_0^\alpha\}). \quad (1.15)$$

The thermodynamic interpretation of Eq. (1.15) is that it describes the driving force for the initial inherent state to create excitations.

There are three consequences following the usage of TST to construct the isoconfigurational partition function:

1. As illustrated in Fig. S.3(b), two neighboring inherent states may have the same potential energies, but drastically different  $p_{\text{iso}}$  values due to the differences in energy barriers. This emphasizes the fact that we are not modeling their long-time equilibrium statistics, but their statistics at short intermediate timescales.
2. The transmission coefficient [17, 18] is ignored due to the no-recrossing assumption. Thus, the computation of  $Q_{\text{iso}}(\{\mathbf{R}_0^\alpha\})$  is independent of the dynamical properties of the liquid and relies solely on its static properties through the potential energy.
3. Because TST assumes equilibrium between the reactant and transition states, the isoconfigurational ensemble is effectively a thermodynamic ensemble of transition states. Since localized excitations are associated with the transition states [7], we can use  $Q_{\text{iso}}(\{\mathbf{R}_0^\alpha\})$  as a basis for constructing the partition function of a system of excitations. This is done in the next section, Section 1.2.

## 1.2 Building a Grand Canonical Ensemble of Excitations

Excitations enter into the picture when we discuss how the sum in  $Q_{\text{iso}}(\{\mathbf{R}_0^\alpha\})$  (Eq. (1.11)) is computed. To see this, we may use the fact that all inherent-state jumps between  $\{\mathbf{R}^\alpha\} \in \mathcal{B}(\{\mathbf{R}_0^\alpha\})$  and  $\{\mathbf{R}_0^\alpha\}$  can be classified in terms of the number of excitations  $N_{\text{exc}}(\{\mathbf{R}^\alpha\}; \{\mathbf{R}_0^\alpha\})$  detected in them. Let the subset of  $\mathcal{B}$  containing inherent states with exactly  $N_{\text{exc}}$ -many excitations be denoted as

$$\mathcal{B}_{N_{\text{exc}}}(\{\mathbf{R}_0^\alpha\}) = \{\{\mathbf{R}^\alpha\} \in \mathcal{B} \mid N_{\text{exc}}(\{\mathbf{R}^\alpha\}; \{\mathbf{R}_0^\alpha\}) = N_{\text{exc}}\}. \quad (1.16)$$

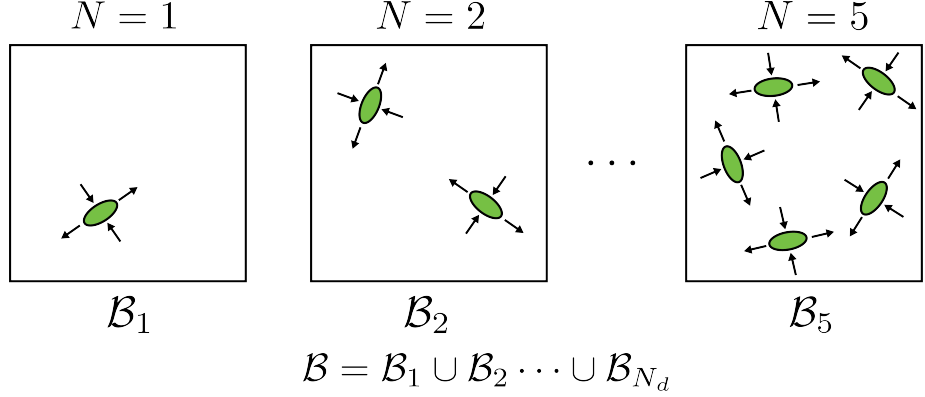

Figure S.4: An illustration of the subsets of the set of all possible nearest-neighbor inherent states  $\mathcal{B}$ , organized in terms of the number of detectable excitations. Here, we assume that the excitations correspond to T1 transitions inducing localized pure-shear events in the medium [7].

An illustration for configurations belonging to each subset  $\mathcal{B}_{N_{\text{exc}}}(\{\mathbf{R}_0^\alpha\})$  is given in Fig. S.4. We can use Eq. (1.16) to write the set of all nearest-neighbor inherent states  $\mathcal{B}(\{\mathbf{R}_0^\alpha\})$  as

$$\mathcal{B}(\{\mathbf{R}_0^\alpha\}) = \mathcal{B}_1(\{\mathbf{R}_0^\alpha\}) \cup \mathcal{B}_2(\{\mathbf{R}_0^\alpha\}) \cup \dots \cup \mathcal{B}_{N_d}(\{\mathbf{R}_0^\alpha\}) = \bigcup_{N_{\text{exc}}=1}^{N_d} \mathcal{B}_{N_{\text{exc}}}(\{\mathbf{R}_0^\alpha\}), \quad (1.17)$$

where  $N_d$  is the maximum number of excitations, which should scale as  $N_d \sim N$  to reach a thermodynamic limit. Using Eq. (1.17), Eq. (1.11) can be re-written as

$$Q_{\text{iso}}(\{\mathbf{R}_0^\alpha\}) = \sum_{N_{\text{exc}}=1}^{N_d} \left[ \sum_{\{\mathbf{R}^\alpha\} \in \mathcal{B}_{N_{\text{exc}}}(\{\mathbf{R}_0^\alpha\})} e^{-\beta \Delta U(\{\mathbf{R}^\alpha\}^\dagger; \{\mathbf{R}_0^\alpha\})} \right]. \quad (1.18)$$

Equation (1.18) turns the sum over all nearest-neighbor inherent states to a sum over a fluctuating number of excitations.

To bring Eq. (1.18) closer to being a grand canonical partition function for excitations, two additional approximations are needed:

1. Approximate the sum  $\sum_{\{\mathbf{R}^\alpha\} \in \mathcal{B}_{N_{\text{exc}}}(\{\mathbf{R}_0^\alpha\})}$  as an integral over excitation degrees of freedom (DOFs). There are two kinds of DOFs: the translational DOF modeled by a  $d$ -dimensional position vector  $\mathbf{q}^\mu$  and the internal DOFs modeled as a  $d_{\text{int}}$ -dimensional vector  $\mathbf{s}^\mu$ , e.g.,  $d_{\text{int}} = 1$  for a scalar orientation angle  $\psi^\mu$ . Assuming that the excitations are identical, the sum over neighboring inherent states in Eq. (1.11) can be approximated as

$$\sum_{\{\mathbf{R}^\alpha\} \in \mathcal{B}_{N_{\text{exc}}}(\{\mathbf{R}_0^\alpha\})} \approx \frac{1}{(a_{\text{exc}})^{N_{\text{exc}}d} N_{\text{exc}}!} \int \prod_{\mu=1}^{N_{\text{exc}}} d^d \mathbf{q}^\mu d^{d_{\text{int}}} \mathbf{s}^\mu, \quad (1.19)$$

where  $a_{\text{exc}}$  is the characteristic size of the excitations.

2. Approximate the potential energy using the elastic strain energy. To write this approximation, let  $\epsilon_{ij}^\dagger(\mathbf{x}) = \frac{1}{2} [u_{i,j}^\dagger(\mathbf{x}) + u_{j,i}^\dagger(\mathbf{x})]$  be the strain field of the transition state. According to Ref. [7], the elastic strain energy can be written as

$$\Delta U(\{\mathbf{R}^\alpha\}^\dagger; \{\mathbf{R}_0^\alpha\}) \approx \Delta U[\epsilon_{ij}^\dagger; \{\mathbf{R}_0^\alpha\}] = \frac{1}{2} \int d^d \mathbf{x} \epsilon_{ij}^\dagger(\mathbf{x}) C_{ijkl}(\{\mathbf{R}_0^\alpha\}) \epsilon_{kl}^\dagger(\mathbf{x}), \quad (1.20)$$

where  $C_{ijkl}(\{\mathbf{R}_0^\alpha\})$  is the stiffness tensor that includes both affine and non-affine parts [7, 19, 20]. Given that every excitation induces its own strain field, we can approximate  $\epsilon_{ij}^\dagger(\mathbf{x})$  as a linear combination of excitation strain fields, i.e.,

$$\epsilon_{ij}^\dagger(\mathbf{x}) \approx \sum_{\mu=1}^{N_{\text{exc}}} \epsilon_{ij}^\mu(\mathbf{x} - \mathbf{q}^\mu; \mathbf{s}^\mu), \quad (1.21)$$

where  $\epsilon_{ij}^\mu$  is the strain due to the  $\mu$ -th excitation. Substituting Eq. (1.21) into Eq. (1.20) yields a new potential energy  $\Delta U[\epsilon_{ij}^\dagger; \{\mathbf{R}_0^\alpha\}] \approx \Delta U(\{(\mathbf{q}^\mu, \mathbf{s}^\mu)\}; \{\mathbf{R}_0^\alpha\})$  comprised of a sum of two parts:

$$\Delta U(\{(\mathbf{q}^\mu, \mathbf{s}^\mu)\}; \{\mathbf{R}_0^\alpha\}) = \sum_{\langle \mu, \gamma \rangle} v(\mathbf{q}^\mu, \mathbf{q}^\gamma, \mathbf{s}^\mu, \mathbf{s}^\gamma; \{\mathbf{R}_0^\alpha\}) + \sum_{\mu=1}^{N_{\text{exc}}} E_c(\mathbf{q}^\mu, \mathbf{s}^\mu; \{\mathbf{R}_0^\alpha\}), \quad (1.22)$$

$$v(\mathbf{q}^\mu, \mathbf{q}^\gamma, \mathbf{s}^\mu, \mathbf{s}^\gamma; \{\mathbf{R}_0^\alpha\}) = \int d^d \mathbf{x} \epsilon_{ij}^\mu(\mathbf{x} - \mathbf{q}^\mu; \mathbf{s}^\mu) C_{ijkl}(\{\mathbf{R}_0^\alpha\}) \epsilon_{kl}^\gamma(\mathbf{x} - \mathbf{q}^\gamma; \mathbf{s}^\gamma), \quad (1.23)$$

$$E_c(\mathbf{q}^\mu, \mathbf{s}^\mu; \{\mathbf{R}_0^\alpha\}) = \frac{1}{2} \int d^d \mathbf{x} \epsilon_{ij}^\mu(\mathbf{x} - \mathbf{q}^\mu; \mathbf{s}^\mu) C_{ijkl}(\{\mathbf{R}_0^\alpha\}) \epsilon_{kl}^\mu(\mathbf{x} - \mathbf{q}^\mu; \mathbf{s}^\mu), \quad (1.24)$$

where  $\sum_{\langle \mu, \gamma \rangle} = \frac{1}{2} \sum_{\mu} \sum_{\gamma \neq \mu}$  is a pair-wise sum,  $v(\mathbf{q}^\mu, \mathbf{q}^\gamma, \mathbf{s}^\mu, \mathbf{s}^\gamma; \{\mathbf{R}_0^\alpha\})$  is the pair potential governing the elastic interaction between the  $\mu$ -th and  $\gamma$ -th excitation, and  $E_c(\mathbf{q}^\mu, \mathbf{s}^\mu; \{\mathbf{R}_0^\alpha\})$  is the self-energy of the  $\mu$ -th excitation, i.e., the elastic energetic cost to create a single excitation.

Substituting Eqs. (1.19) and (1.22)–(1.24) into Eq. (1.18), we obtain

$$Q_{\text{iso}}(\{\mathbf{R}_0^\alpha\}) \approx \sum_{N_{\text{exc}}=1}^{N_d} \frac{1}{(a_{\text{exc}})^{N_{\text{exc}}d} N_{\text{exc}}!} \int \prod_{\mu=1}^{N_{\text{exc}}} d^d \mathbf{q}^\mu d^{d_{\text{int}}} \mathbf{s}^\mu e^{-\beta \Delta U(\{(\mathbf{q}^\mu, \mathbf{s}^\mu)\}; \{\mathbf{R}_0^\alpha\})}. \quad (1.25)$$

Equation (1.25) is only valid for one initial inherent state. However, we are also interested in computing ensemble averages over all possible initial inherent states. At thermal equilibrium, they are sampled from a Boltzmann probability [7, 21]

$$p_{\text{IS}}(\{\mathbf{R}^\alpha\}) = \frac{1}{Q_{\text{IS}}} e^{-\beta U(\{\mathbf{R}^\alpha\})}, \quad Q_{\text{IS}} = \sum_{\{\mathbf{R}^\alpha\} \in \mathcal{C}} e^{-\beta U(\{\mathbf{R}^\alpha\})}, \quad (1.26)$$

where  $Q_{\text{IS}}$  the inherent-state partition function and  $\mathcal{C}$  is the set of all possible inherent states. Given a collection of equilibrated inherent-state configurations  $\{\{\mathbf{R}_k^\alpha\}\}_{k=1}^K$ , we can further average the isoconfigurational empirical average in Eq. (1.7) for an observable  $A$  to yield

$$A(K, M) = \frac{1}{K} \sum_{k=1}^K A_{\text{iso}}(\{\mathbf{R}_k^\alpha\}; M) = \frac{1}{K} \sum_{k=1}^K \left[ \frac{1}{M} \sum_{\{\mathbf{R}^\alpha\} \in \mathcal{S}_M(\{\mathbf{R}_k^\alpha\})} A(\{\mathbf{R}^\alpha\}; \{\mathbf{R}_k^\alpha\}) \right], \quad (1.27)$$

where  $A(K, M)$  is the empirical average over  $K$ -many initial inherent states and  $M$ -many trajectories per initial inherent state. Using the most general form of the isoconfigurational ensemble average (Eq. (1.8)), the final ensemble average of an observable is obtained by taking the following limit:

$$\langle A \rangle = \lim_{\substack{K \rightarrow \infty \\ M \rightarrow \infty}} A(K, M) = \left\langle \sum_{\{\mathbf{R}^\alpha\} \in \mathcal{B}(\{\mathbf{R}_0^\alpha\})} A(\{\mathbf{R}^\alpha\}; \{\mathbf{R}_0^\alpha\}) p_{\text{iso}}(\{\mathbf{R}^\alpha\}; \{\mathbf{R}_0^\alpha\}) \right\rangle_{\text{IS}} \quad (1.28)$$

$$= \left\langle \frac{1}{Q_{\text{iso}}(\{\mathbf{R}_0^\alpha\})} \sum_{\{\mathbf{R}^\alpha\} \in \mathcal{B}(\{\mathbf{R}_0^\alpha\})} A(\{\mathbf{R}^\alpha\}; \{\mathbf{R}_0^\alpha\}) e^{-\beta \Delta U(\{\mathbf{R}^\alpha\}^\dagger; \{\mathbf{R}_0^\alpha\})} \right\rangle_{\text{IS}}. \quad (1.29)$$

The computation of Eq. (1.29) involves an ensemble average of the inverse of the isoconfigurational partition function,  $Q_{\text{iso}}(\{\mathbf{R}_0^\alpha\})$ , over all possible initial inherent states. To simplify the computation, let us write  $Q_{\text{iso}}(\{\mathbf{R}_0^\alpha\})$  as a sum of its mean, denoted as  $\langle Q_{\text{iso}}(\{\mathbf{R}_0^\alpha\}) \rangle_{\text{IS}} = \bar{Q}_{\text{iso}}$ , and fluctuation. This yields

$$Q_{\text{iso}}(\{\mathbf{R}_0^\alpha\}) = \bar{Q}_{\text{iso}} + \delta Q_{\text{iso}}(\{\mathbf{R}_0^\alpha\}). \quad (1.30)$$

The inverse of  $Q_{\text{iso}}(\{\mathbf{R}_0^\alpha\})$  entering Eq. (1.29) can be expanded in a Taylor series for small fluctuations:

$$\frac{1}{Q_{\text{iso}}(\{\mathbf{R}_0^\alpha\})} = \frac{1}{\bar{Q}_{\text{iso}}} \left( 1 - \frac{\delta Q_{\text{iso}}(\{\mathbf{R}_0^\alpha\})}{\bar{Q}_{\text{iso}}} + \dots \right). \quad (1.31)$$

Let  $\delta Q_{\text{iso}}(\{\mathbf{R}_0^\alpha\})/\bar{Q}_{\text{iso}} = \delta \tilde{Q}_{\text{iso}}(\{\mathbf{R}_0^\alpha\})$ . Substituting Eq. (1.31) into Eq. (1.29) yields

$$\langle A \rangle = \frac{1}{\bar{Q}_{\text{iso}}} \left\langle \sum_{\{\mathbf{R}^\alpha\} \in \mathcal{B}(\{\mathbf{R}_0^\alpha\})} A(\{\mathbf{R}^\alpha\}; \{\mathbf{R}_0^\alpha\}) e^{-\beta \Delta U(\{\mathbf{R}^\alpha\}^\dagger; \{\mathbf{R}_0^\alpha\})} \right\rangle_{\text{IS}} + \mathcal{O}(\delta \tilde{Q}_{\text{iso}}(\{\mathbf{R}_0^\alpha\})). \quad (1.32)$$

We can show that  $\delta \tilde{Q}_{\text{iso}}(\{\mathbf{R}_0^\alpha\})$  vanishes in the thermodynamic limit by analyzing the excitation representation of  $Q_{\text{iso}}(\{\mathbf{R}_0^\alpha\})$  (Eq. (1.25)). In this representation,  $\{\mathbf{R}_0^\alpha\}$  enters into the partition function only through the elastic moduli, which can be written as a sum of its mean  $\langle C_{ijkl}(\{\mathbf{R}_0^\alpha\}) \rangle_{\text{IS}} = C_{ijkl}^{\text{IS}}$  and fluctuation:

$$C_{ijkl}(\{\mathbf{R}_0^\alpha\}) = C_{ijkl}^{\text{IS}} + \delta C_{ijkl}(\{\mathbf{R}_0^\alpha\}). \quad (1.33)$$

As shown in Fig. S.5 the variance of these fluctuations decay as  $\mathcal{O}(1/N)$  because the elastic modulus is an intensive thermodynamic property of the system [22]. For large system sizes, this implies that

$$C_{ijkl}(\{\mathbf{R}_0^\alpha\}) \approx C_{ijkl}^{\text{IS}}; \quad \Delta U(\{(\mathbf{q}^\mu, \mathbf{s}^\mu)\}; \{\mathbf{R}_0^\alpha\}) \approx \Delta \bar{U}(\{(\mathbf{q}^\mu, \mathbf{s}^\mu)\}), \quad (1.34)$$

where  $\Delta \bar{U}(\{(\mathbf{q}^\mu, \mathbf{s}^\mu)\})$  is the inherent-state averaged potential energy of the excitations. Given the approximations in Eq. (1.34), we can now prove that  $\delta \tilde{Q}_{\text{iso}}(\{\mathbf{R}_0^\alpha\})$  vanishes in the thermodynamic limit by first Taylor expanding the Boltzmann factor

$$e^{-\beta \Delta U(\{(\mathbf{q}^\mu, \mathbf{s}^\mu)\}; \{\mathbf{R}_0^\alpha\})} \approx e^{-\beta \Delta \bar{U}(\{(\mathbf{q}^\mu, \mathbf{s}^\mu)\})} (1 - \delta U), \quad (1.35)$$

where  $\delta U = \delta(\Delta U(\{(\mathbf{q}^\mu, \mathbf{s}^\mu)\}; \{\mathbf{R}_0^\alpha\}))$  is the fluctuation of the potential energy induced by the elastic moduli.

Substituting Eq. (1.35) into Eq. (1.30), we obtain the following inherent-state averaged isoconfigurational partition function

$$\bar{Q}_{\text{iso}} = \sum_{N_{\text{exc}}=1}^{N_d} \frac{1}{(a_{\text{exc}})^{N_{\text{exc}}d} N_{\text{exc}}!} \int \prod_{\mu=1}^{N_{\text{exc}}} d^d \mathbf{q}^\mu d^{d_{\text{int}}} \mathbf{s}^\mu e^{-\beta \Delta \bar{U}(\{(\mathbf{q}^\mu, \mathbf{s}^\mu)\})} = \sum_{N_{\text{exc}}=1}^{N_d} \bar{Q}_{\text{iso}, N_{\text{exc}}}, \quad (1.36)$$

where  $\bar{Q}_{\text{iso}, N_{\text{exc}}}$  is the inherent-state averaged isoconfigurational partition function, conditioned upon having a fixed number of excitations,

$$\bar{Q}_{\text{iso}, N_{\text{exc}}} = \frac{1}{(a_{\text{exc}})^{N_{\text{exc}}d} N_{\text{exc}}!} \int \prod_{\mu=1}^{N_{\text{exc}}} d^d \mathbf{q}^\mu d^{d_{\text{int}}} \mathbf{s}^\mu e^{-\beta \Delta \bar{U}(\{(\mathbf{q}^\mu, \mathbf{s}^\mu)\})}. \quad (1.37)$$

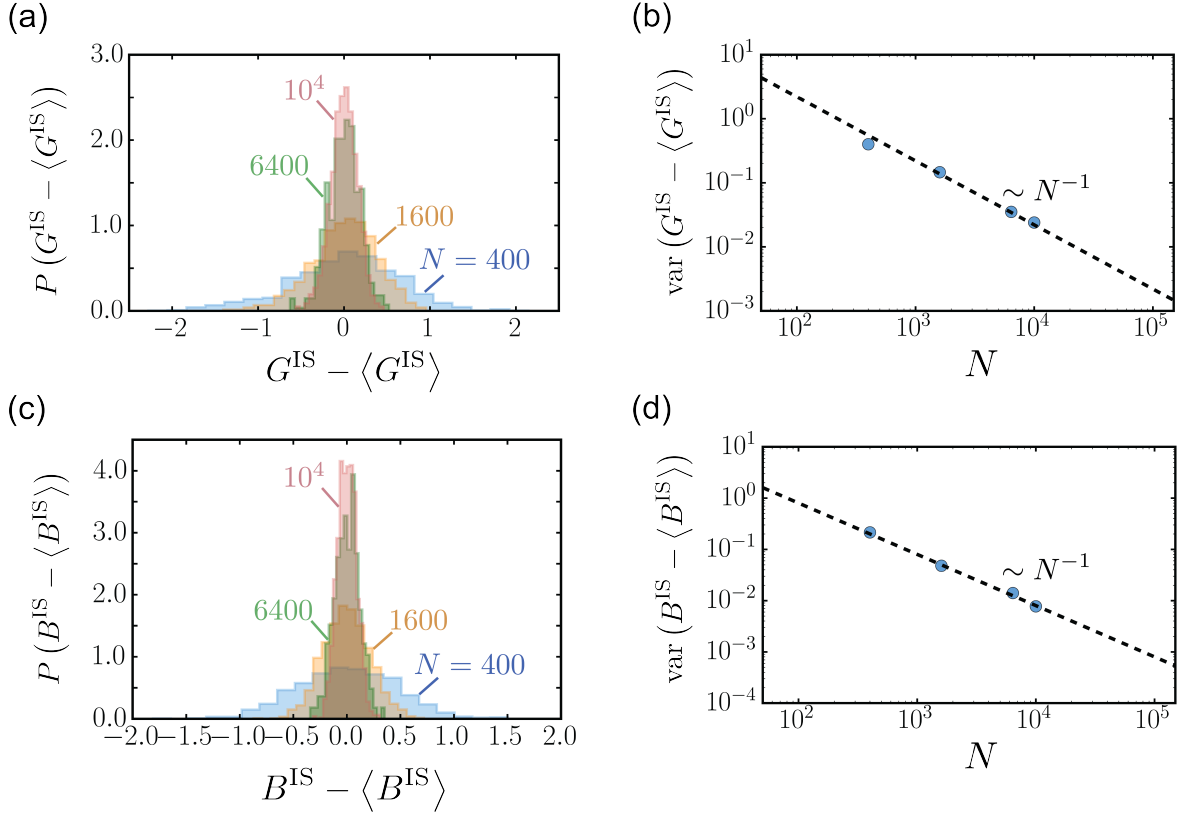

Figure S.5: The distribution and variance of shear modulus (a,b) and bulk modulus (c,d) at different system sizes and  $T = 0.095$ . The  $\mathcal{O}(1/N)$  scaling of the variance implies that every sample converges towards their mean in the thermodynamic limit.

Additionally, the fluctuations around  $\bar{Q}_{\text{iso}}$  can be written as

$$\delta Q_{\text{iso}}(\{\mathbf{R}_0^\alpha\}) \approx - \sum_{N_{\text{exc}}=1}^{N_d} \frac{1}{(a_{\text{exc}})^{N_{\text{exc}}d} N_{\text{exc}}!} \int \prod_{\mu=1}^{N_{\text{exc}}} d^d \mathbf{q}^\mu d^{d_{\text{int}}} \mathbf{s}^\mu \delta U e^{-\beta \Delta \bar{U}(\{\mathbf{q}^\mu, \mathbf{s}^\mu\})} \approx 0, \quad (1.38)$$

where the second equality in Eq. (1.38) is obtained by using Eq. (1.34), and thereby demonstrating the vanishing of  $\delta Q_{\text{iso}}(\{\mathbf{R}_0^\alpha\})$  for large system sizes. Finally, we can use the new set of approximations to simplify the computation of ensemble averages in Eq. (1.32). As a concrete example, we may take the number of excitations  $N_{\text{exc}}(\{\mathbf{R}^\alpha\}, \{\mathbf{R}_0^\alpha\})$  as the chosen observable. Using Eqs. (1.25), (1.32), (1.34) and (1.38), we find that

$$\langle N_{\text{exc}} \rangle \approx \frac{1}{\bar{Q}_{\text{iso}}} \left\langle \sum_{N_{\text{exc}}=1}^{N_d} \frac{1}{(a_{\text{exc}})^{N_{\text{exc}}d} N_{\text{exc}}!} \int \prod_{\mu=1}^{N_{\text{exc}}} d^d \mathbf{q}^\mu d^{d_{\text{int}}} \mathbf{s}^\mu N_{\text{exc}}(\{\mathbf{R}^\alpha\}, \{\mathbf{R}_0^\alpha\}) e^{-\beta \Delta U(\{\mathbf{q}^\mu, \mathbf{s}^\mu\}; \{\mathbf{R}_0^\alpha\})} \right\rangle_{\text{IS}} \quad (1.39)$$

$$= \frac{1}{\bar{Q}_{\text{iso}}} \sum_{N_{\text{exc}}=1}^{N_d} \frac{N_{\text{exc}}}{(a_{\text{exc}})^{N_{\text{exc}}d} N_{\text{exc}}!} \int \prod_{\mu=1}^{N_{\text{exc}}} d^d \mathbf{q}^\mu d^{d_{\text{int}}} \mathbf{s}^\mu e^{-\beta \Delta \bar{U}(\{\mathbf{q}^\mu, \mathbf{s}^\mu\})}, \quad (1.40)$$

where Eq. (1.40) is obtained by applying Eq. (1.35) to Eq. (1.39).

To proceed further, note that Eq. (1.40) is similar to averages in a grand canonical ensemble for a classical many-body system [23]. In such an ensemble, the fugacity plays the role of an auxiliary

variable that we can use to compute the average number of particles via derivatives of the grand canonical partition function [23]. In the isoconfigurational ensemble, an analogous auxiliary variable may be found by writing the inherent-state averaged potential energy  $\Delta\bar{U}$  more explicitly as a sum of pair potentials  $\bar{v}^{\mu\gamma}$  and self-energy  $\bar{E}_c$ :

$$\Delta\bar{U}(\{\mathbf{q}^\mu, \mathbf{s}^\mu\}) = \sum_{\langle\mu,\gamma\rangle} \bar{v}^{\mu\gamma} + \bar{E}_c N_{\text{exc}}, \quad (1.41)$$

$$\bar{v}^{\mu\gamma} = \int d^d \mathbf{x} \, \epsilon_{ij}^\mu(\mathbf{x} - \mathbf{q}^\mu; \mathbf{s}^\mu) C_{ijkl}^{\text{IS}} \epsilon_{kl}^\gamma(\mathbf{x} - \mathbf{q}^\gamma; \mathbf{s}^\gamma), \quad (1.42)$$

$$\bar{E}_c = \frac{1}{2N_{\text{exc}}} \sum_{\mu=1}^{N_{\text{exc}}} \int d^d \mathbf{x} \, \epsilon_{ij}^\mu(\mathbf{x} - \mathbf{q}^\mu; \mathbf{s}^\mu) C_{ijkl}^{\text{IS}} \epsilon_{kl}^\mu(\mathbf{x} - \mathbf{q}^\mu; \mathbf{s}^\mu), \quad (1.43)$$

where  $\sum_{\langle\mu,\gamma\rangle} = \frac{1}{2} \sum_{\mu=1}^{N_{\text{exc}}} \sum_{\gamma \neq \mu}^{N_{\text{exc}}}$  is the pair-wise sum over excitations. Suppose that the self-energy  $\bar{E}_c$  is constant with respect to the excitation coordinates and internal degrees of freedoms. Substituting Eqs. (1.41)–(1.43) into Eq. (1.40) yields

$$\langle N_{\text{exc}} \rangle = \frac{1}{\bar{Q}_{\text{iso}}} \sum_{N_{\text{exc}}=1}^{N_d} \frac{N_{\text{exc}}}{(a_{\text{exc}})^{N_{\text{exc}}d} N_{\text{exc}}!} \int \prod_{\mu=1}^{N_{\text{exc}}} d^d \mathbf{q}^\mu d^{d_{\text{int}}} \mathbf{s}^\mu e^{-\beta \sum_{\langle\mu,\gamma\rangle} \bar{v}^{\mu\gamma}} e^{-\beta \bar{E}_c N_{\text{exc}}} \quad (1.44)$$

$$= \frac{1}{\bar{Q}_{\text{iso}}} \sum_{N_{\text{exc}}=1}^{N_d} \frac{N_{\text{exc}} y^{N_{\text{exc}}}}{(a_{\text{exc}})^{N_{\text{exc}}d} N_{\text{exc}}!} \int \prod_{\mu=1}^{N_{\text{exc}}} d^d \mathbf{q}^\mu d^{d_{\text{int}}} \mathbf{s}^\mu e^{-\beta \sum_{\langle\mu,\gamma\rangle} \bar{v}^{\mu\gamma}}, \quad (1.45)$$

where the variable  $y$  is defined as the Boltzmann factor of the self-energy. Thus,

$$y = e^{-\beta \bar{E}_c} \quad (1.46)$$

and it plays the role of fugacity in this isoconfigurational ensemble.

Given the fugacity variable Eq. (1.46), we can employ a trick of taking derivatives of  $\bar{Q}_{\text{iso}}$  to compute Eq. (1.45). In particular, using the fact that

$$N_{\text{exc}} y^{N_{\text{exc}}} = y \frac{d}{dy} y^{N_{\text{exc}}} = \frac{d}{d \ln y} y^{N_{\text{exc}}}, \quad (1.47)$$

we can write Eq. (1.45) as follows:

$$\langle N_{\text{exc}} \rangle = \frac{1}{\bar{Q}_{\text{iso}}} \frac{d}{d \ln y} \sum_{N_{\text{exc}}=1}^{N_d} \frac{y^{N_{\text{exc}}}}{(a_{\text{exc}})^{N_{\text{exc}}d} N_{\text{exc}}!} \int \prod_{\mu=1}^{N_{\text{exc}}} d^d \mathbf{q}^\mu d^{d_{\text{int}}} \mathbf{s}^\mu e^{-\beta \sum_{\langle\mu,\gamma\rangle} \bar{v}^{\mu\gamma}} \quad (1.48)$$

$$= \frac{1}{\bar{Q}_{\text{iso}}} \frac{d \bar{Q}_{\text{iso}}}{d \ln y} = -k_B T \frac{d \ln \bar{Q}_{\text{iso}}}{d E_c}. \quad (1.49)$$

This result, where ensemble averages are computed via derivatives of the partition function, also generalizes to other observables. For example, the potential energy and heat capacities can be computed by taking derivatives of  $\bar{Q}_{\text{iso}}$  with respect to temperature. Thus, we may conclude that  $\bar{Q}_{\text{iso}}$  (Eq. (1.36)) forms the basis of studying the thermodynamics of the inherent-state jumps or, equivalently, excitations in supercooled liquids.

Note that subsequent analyses in this work involve comparing states in the isoconfigurational ensemble with an empty state where no excitations are present. For such studies, it is useful to

add the Boltzmann factor of the empty state, which is  $e^{-\beta\Delta\bar{U}} = e^0 = 1$ , to  $\bar{Q}_{\text{iso}}$  (Eq. (1.36)). This addition provides us with a grand canonical partition function for a many-excitation system

$$\bar{\Xi}_{\text{exc}} = \bar{Q}_{\text{iso}} + 1, \quad (1.50)$$

which can be written more explicitly as

$$\bar{\Xi}_{\text{exc}} = \sum_{N_{\text{exc}}=0}^{N_d} Z_{N_{\text{exc}}} y^{N_{\text{exc}}}, \quad Z_{N_{\text{exc}}} = \frac{1}{(a_{\text{exc}})^{N_{\text{exc}}d} N_{\text{exc}}!} \int \prod_{\mu=1}^{N_{\text{exc}}} d^d \mathbf{q}^\mu d^{d_{\text{int}}} \mathbf{s}^\mu e^{-\beta \mathcal{H}(\{\mathbf{q}^\mu, \mathbf{s}^\mu\})}, \quad (1.51)$$

$$y = e^{-\beta \bar{E}_c}, \quad \mathcal{H}(\{\mathbf{q}^\mu, \mathbf{s}^\mu\}) = \sum_{\langle \mu, \gamma \rangle} \bar{v}^{\mu\gamma}, \quad (1.52)$$

where  $\bar{v}^{\mu\gamma}$  and  $\bar{E}_c$  are given in Eq. (1.42) and Eq. (1.43), respectively,  $\mathcal{H}$  and  $Z_{N_{\text{exc}}}$  are the effective Hamiltonian and canonical partition function of the excitations, when their number is fixed to  $N_{\text{exc}}$ .

### 1.3 Application to Non-Interacting Excitations

We can apply the framework developed in Section 1.2 to an ideal gas of excitations ( $\bar{v}^{\mu\gamma} = 0$ ). Such system models uncorrelated inherent-state jumps, which is the statistics we expect at very short times and low temperatures [24]. In the thermodynamic limit, the isoconfigurational partition function becomes

$$\bar{Q}_{\text{iso}} = \sum_{N_{\text{exc}}=1}^{\infty} \frac{y^{N_{\text{exc}}}}{(a_{\text{exc}})^{N_{\text{exc}}d} N_{\text{exc}}!} \int \prod_{\mu=1}^{N_{\text{exc}}} d^d \mathbf{q}^\mu d^{d_{\text{int}}} \mathbf{s}^\mu = \sum_{N_{\text{exc}}=1}^{N_d} \frac{(yVS/(a_{\text{exc}})^d)^{N_{\text{exc}}}}{N_{\text{exc}}!} \quad (1.53)$$

$$= \exp\left(yVS/(a_{\text{exc}})^d\right) - 1 \approx \exp\left(yVS/(a_{\text{exc}})^d\right), \quad (1.54)$$

where  $V$  is the volume,  $S = \int d^{d_{\text{int}}} \mathbf{s}$ , and the second equality in Eq. (1.54) is obtained by assuming large  $V$ . Substituting Eq. (1.54) into Eq. (1.49) we obtain

$$\langle N_{\text{exc}} \rangle = y \frac{d}{dy} \left( yVS/(a_{\text{exc}})^d \right) = \frac{yVS}{(a_{\text{exc}})^d} = \frac{VS}{(a_{\text{exc}})^d} e^{-\beta \bar{E}_c}. \quad (1.55)$$

Defining the concentration of excitations as  $c_{\text{eq}} := \frac{\langle N_{\text{exc}} \rangle}{V}$ , we find that

$$c_{\text{eq}}(T) = \frac{S}{(a_{\text{exc}})^d} e^{-\beta \bar{E}_c}, \quad (1.56)$$

which is the expected Arrhenius formula for non-interacting excitations.

The Arrhenius formula  $c_{\text{eq}}(T)$  we obtained from an ideal gas of excitations is consistent with previous works related to dynamical facilitation (DF) theory [2]. First, Eq. (1.56) matches with the concentration assumed in the kinetically constrained spin-lattice models [25, 26]. These models provide a coarse-grained description of supercooled liquid dynamics in terms of excitations relaxing nearby excitations in a hierarchical manner, and thus were used in DF theory to guide predictions on super-Arrhenius relaxation behavior. Using the East model [27, 28] as an example, the dimensionless concentration of excitations can be written as

$$\tilde{c}_{\text{eq}}(T) = \frac{e^{-\beta \bar{E}_c}}{1 + e^{-\beta \bar{E}_c}} \rightarrow e^{-\beta \bar{E}_c} \quad \text{as } T \rightarrow 0. \quad (1.57)$$

Equation (1.57) can be obtained from Eq. (1.56) by assuming that excitations have no internal DOFs ( $S = 1$ ) and  $a_{\text{exc}} = \sigma_{\text{d}}$ , where  $\sigma_{\text{d}}$  is the particle diameter. In this case, the dimensionless concentration of excitations from Eq. (1.56) is  $\tilde{c}_{\text{eq}}(T) := c_{\text{eq}}(\sigma_{\text{d}})^d = e^{-\beta \bar{E}_{\text{c}}}$ , which agrees with Eq. (1.57). Second, Eq. (1.56) is also consistent with the rate of particle-hopping events  $c_{\sigma}(T)$ , which is computed by analyzing coarse-grained particle trajectories [24]. In the perspective of DF theory, the rate quantity  $c_{\sigma}(T)$  is a proxy for  $c_{\text{eq}}(T)$  from molecular simulations, and it has been empirically observed to follow an Arrhenius law [7, 24], i.e.,

$$c_{\sigma}(T) \sim e^{-J_{\sigma}(\beta - \beta_0)} \quad \text{for } T \leq T_0, \quad (1.58)$$

where  $J_{\sigma}$  is the apparent energy barrier and  $\beta_0 = 1/k_{\text{B}}T_0$ . This result was previously interpreted as due to the uncorrelated nature of the first few hopping events at deeply supercooled conditions, consistent with the non-interacting nature of the excitations. This work provides a justification for using the Arrhenius form for the concentration of excitations in the DF theory.

Using Eq. (1.54), we also find that the free energy is

$$\bar{F}_{\text{iso}}(T) = -k_{\text{B}}T \ln \bar{Q}_{\text{iso}} = -k_{\text{B}}T y V S / (a_{\text{exc}})^d = -k_{\text{B}}T \langle N_{\text{exc}} \rangle < 0. \quad (1.59)$$

Note that  $\bar{F}_{\text{iso}}(T)$  represents the average free-energy difference between the nearby transition states and the initial reactant state (see Eq. (1.15)). Thus, we may conclude from Eq. (1.59) that a supercooled liquid whose excitations are non-interacting is always thermodynamically driven to jump from its initial inherent state. This driving force is also entropic since it increases as the size of both translational (through  $V$ ) and internal DOFs (through  $S$ ) increases. When interactions are included, we may predict opposite driving forces where excitations are no longer thermodynamically favorable. The framework to model these excitations via linear elasticity theory is the focus of Section 2.

## 2 Elasticity Theory of Defects in Two Dimensions

In this section, we review the elasticity theory of defects in two dimensions (2D), with emphasis on its application to model excitations in supercooled liquids. In Section 2.1, we introduce stress functions and incompatibility strains as tools for modeling elastic defects in 2D. In Section 2.2, we introduce the Volterra construction [29]; a macroscopic approach for introducing defects in a continuum solid. We also demonstrate how a Volterra construction can correspond to a localized source of strain incompatibility, whose mathematical form resembles a source of localized point ‘charges’ like the one from electrostatics [3, 4].

After discussing boundary conditions in Section 2.3, the alternative ‘electrostatics’ framework is used in Section 2.4 to derive conservation laws analogous to electroneutrality conditions in charged systems. These laws are important for applications in statistical mechanics as they constrain the allowable distribution of defects depending on the chosen boundary conditions. Finally, we end with a derivation of the stress-function solutions for different classes of defects in Section 2.5. These solutions are useful for discussing the thermodynamics and interaction of such defects in Section 3.1.

### 2.1 Incompatibility Strain Fields and Stress Functions

We are interested in describing the response of a linear elastic medium when defects are present. The nature of defects can be of any kind (e.g. point defects, disclinations, dislocations, Eshelby’s inclusions, etc.) leading to qualitatively different displacement fields  $u_i^{\text{d}}(\mathbf{x})$  that exhibit spatial

discontinuities. In response to such discontinuities, the solid medium deforms elastically and induces an elastic displacement field  $u_i^e(\mathbf{x})$ . This results in a total displacement field  $u_i(\mathbf{x})$  that is continuous, which can be written as

$$u_i(\mathbf{x}) = u_i^e(\mathbf{x}) + u_i^d(\mathbf{x}) . \quad (2.1)$$

The equivalent form of Eq. (2.1) in terms of strains is

$$\epsilon_{ij} = \epsilon_{ij}^e + \epsilon_{ij}^d . \quad (2.2)$$

The continuity of  $u_i(\mathbf{x})$  leads to the additional constraint of compatibility on the corresponding strain  $\epsilon_{ij}$ , which is expressed in two dimensions (2D) as

$$\varepsilon_{ik}\varepsilon_{jl}\epsilon_{ij,kl} = 0 , \quad (2.3)$$

where  $\varepsilon_{ij}$  is the 2D Levi-Civita symbol with  $\varepsilon_{11} = \varepsilon_{22} = 0$  and  $\varepsilon_{12} = -\varepsilon_{21} = 1$ . Equation (2.3) can be derived from the fact that the following second-order partial derivatives of the strain tensor

$$\epsilon_{11,22} = u_{1,122} , \quad \epsilon_{22,11} = u_{2,211} , \quad \epsilon_{12,12} = \frac{1}{2} (u_{1,212} + u_{2,112}) \quad (2.4)$$

are not independent of each other. In fact, from the continuity of  $u_i(\mathbf{x})$  and its derivatives, we must have that

$$\epsilon_{11,22} + \epsilon_{22,11} - 2\epsilon_{12,12} = u_{1,122} + u_{2,211} - u_{1,212} - u_{2,112} = 0 . \quad (2.5)$$

The left part of Eq. (2.5) is precisely Eq. (2.3) in terms of its Cartesian components. By substituting the decomposition in Eq. (2.2) into Eq. (2.3), we find

$$\varepsilon_{ik}\varepsilon_{jl}\epsilon_{ij,kl}^e = -\varepsilon_{ik}\varepsilon_{jl}\epsilon_{ij,kl}^d . \quad (2.6)$$

The form of Eq. (2.6) implies that elastic strain fields  $\epsilon_{ij}^e$  will develop as a consequence of introducing defects in the elastic medium via  $\epsilon_{ij}^d$ .

The quantity  $-\varepsilon_{ik}\varepsilon_{jl}\epsilon_{ij,kl}^d$  is often referred to as the incompatibility source  $\eta(\mathbf{x})$  [30], i.e.,

$$\eta(\mathbf{x}) := -\varepsilon_{ik}\varepsilon_{jl}\epsilon_{ij,kl}^d , \quad \varepsilon_{ik}\varepsilon_{jl}\epsilon_{ij,kl}^e = \eta(\mathbf{x}) . \quad (2.7)$$

The source  $\eta(\mathbf{x})$  is non-zero when defects are introduced since the defect strain  $\epsilon_{ij}^d$  violates the compatibility condition, hence the name ‘incompatibility’. Equation (2.7) can also be written in terms of the elastic stress field  $T_{ij}^e$ . For linear elastic solids, the stress is related to the elastic strain  $\epsilon_{ij}^e$  through the following relation:

$$T_{ij}^e = C_{ijkl}\epsilon_{kl}^e , \quad (2.8)$$

where  $C_{ijkl}$  is the stiffness tensor. Alternatively, we can also invert Eq. (2.8) to write the following linear relation:

$$\epsilon_{ij}^e = S_{ijkl}T_{kl}^e , \quad (2.9)$$

where  $S_{ijkl}$  is the compliance tensor. By substituting Eq. (2.9) into the compatibility condition in Eq. (2.7) we arrive at

$$S_{ijmn}\varepsilon_{ik}\varepsilon_{jl}T_{mn,kl}^e = \eta(\mathbf{x}) . \quad (2.10)$$

In addition to the linear constitutive law, the 2D nature of the solid allows us to express the elastic stress field  $T_{ij}^e$  in terms of the Airy stress function  $\chi(\mathbf{x})$  as

$$T_{ij}^e = \varepsilon_{ik}\varepsilon_{jl}\chi_{,kl} = \chi_{,kk}\delta_{ij} - \chi_{,ij} , \quad (2.11)$$

where the second equality is obtained via the identity  $\varepsilon_{ik}\varepsilon_{jl} = \delta_{ij}\delta_{kl} - \delta_{il}\delta_{kj}$ . Note that Eq. (2.11) satisfies identically the force balance in domains where no defects are present, i.e.,  $T_{ij,j}^e = \varepsilon_{ik}\varepsilon_{jl}\chi_{,klj} = 0$ . Combining Eq. (2.9) with Eq. (2.11), we can also express  $\epsilon_{ij}^e$  as a function of  $\chi(\mathbf{x})$ , leading to

$$\epsilon_{ij}^e = S_{ijkl}\varepsilon_{km}\varepsilon_{ln}\chi_{,mn} = S_{ijkk}\chi_{,mm} - S_{ijkl}\chi_{,kl}. \quad (2.12)$$

Furthermore, by substituting Eq. (2.11) into the compatibility condition in Eq. (2.10) we arrive at

$$S_{ijkl}\chi_{,ijkl} = \eta(\mathbf{x}). \quad (2.13)$$

Equation (2.13) constitutes the final equation for modeling the elastic field of defects via the solution for the stress function  $\chi(\mathbf{x})$ .

For an isotropic linear elastic solid, the stiffness tensor can be written as

$$C_{ijkl} = \lambda\delta_{ij}\delta_{kl} + G(\delta_{ik}\delta_{jl} + \delta_{il}\delta_{jk}) = 2G\frac{\nu}{1-\nu}\delta_{ij}\delta_{kl} + G(\delta_{ik}\delta_{jl} + \delta_{il}\delta_{jk}), \quad (2.14)$$

where  $G$  and  $\lambda$  are the shear modulus and the first Lamé parameter, respectively. The compliance tensor is

$$S_{ijkl} = \frac{1}{4G}(\delta_{ik}\delta_{jl} + \delta_{il}\delta_{jk}) - \frac{\lambda}{4G(\lambda + G)}\delta_{ij}\delta_{kl} = \frac{1}{4G}(\delta_{ik}\delta_{jl} + \delta_{il}\delta_{jk}) - \frac{1}{2G}\frac{\nu}{1+\nu}\delta_{ij}\delta_{kl}, \quad (2.15)$$

where  $\nu = \frac{\lambda}{\lambda+2G}$  is the 2D Poisson's ratio. Note that a superscript 'IS' needs to be introduced in all elastic moduli if the isotropic solid corresponds to inherent states of supercooled liquids [7], which we omit for brevity. Substituting Eq. (2.15) in Eq. (2.12), we obtain the strain-stress-function relation for isotropic solids

$$\epsilon_{ij}^e = \frac{1}{Y}(\chi_{,kk}\delta_{ij} - (1+\nu)\chi_{,ij}), \quad (2.16)$$

where  $Y = 2G(1+\nu)$  is the Young's modulus, while substituting Eq. (2.15) in Eq. (2.13) gives us the equation for determining the Airy stress function in isotropic solids,

$$\frac{1}{Y}\nabla^4\chi = \eta(\mathbf{x}). \quad (2.17)$$

For all subsequent analyses, we rely heavily on Eqs. (2.16) and (2.17) as a basis for modeling defects and their energetics.

## 2.2 Elastic Defects as Geometric 'Charges'

As discussed in Section 2.1, defects are sources of discontinuities in the elastic fields. In the context of crystalline solids, the discontinuities can be identified directly from imperfections in the geometry of the perfect lattice. However, we are interested in defects in amorphous solids, e.g., inherent states of supercooled liquids, where discontinuities are generated via thermally-activated bond-breaking events. For such solids, there exists a macroscopic approach known as the Volterra construction [29], which is a series of cuts, insertions/removals, and gluing steps that replicate an internal distribution of stress and strain due to defects.

This section demonstrates the Volterra construction for three classes of defects: disclinations, dislocations, and point defects. In addition, we explain a framework developed by Moshe and co-workers [3, 4] where each class of defects from the Volterra construction corresponds to a particular localized source of incompatibility  $\eta(\mathbf{x})$ . This new framework allows us to model all possible classes of defects via analogies to electrostatics [3, 4]. In particular, a disclination, dislocation, and point

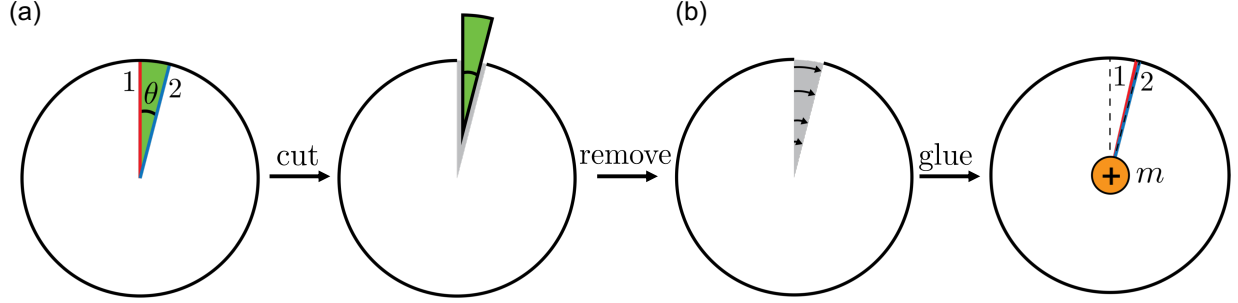

Figure S.6: (a) The Volterra construction that yields a disclination in a solid, i.e., localized source of rotational displacement and strain. (b) Disclination as a (positive) monopole source in the incompatibility  $\eta(\mathbf{x})$ . Note that a negative source may be introduced by introducing a wedge with an angle larger than the original cut [29].

defect can be thought of as a ‘geometric’ monopole, dipole, and quadrupole source in  $\eta(\mathbf{x})$ , respectively. The electrostatics framework is completely independent of the Volterra construction, which is macroscopic in nature, and is generalizable to many-defect systems. Thus, the electrostatics framework is more useful in microscopic applications such as the statistical mechanics of excitations in supercooled liquids.

**Disclinations as Monopoles:** To begin, suppose that we have a circular solid shown in Fig. S.6, where the center of mass is located at  $\mathbf{x} = \mathbf{q}$ . We introduce the disclination as a Volterra construction that cuts a wedge of angle  $m$  (Fig. S.6(a)) in the material, and glues the two open sides together via an elastic deformation (Fig. S.6(b)). This process yields a discontinuity in the angular part of the elastic displacement  $u_\theta^e$ . In particular, the jump in  $u_\theta^e$  at side ‘2’ with respect to side ‘1’ is

$$[[u_\theta^e]] = m\Delta r, \quad (2.18)$$

where  $\Delta r = |\mathbf{x} - \mathbf{q}|$ . Note that Eq. (2.18) also implies a discontinuity in the rotation tensor  $w_{ij}^e$ , which is computed from the anti-symmetric part of the displacement gradient, i.e.,

$$w_{ij}^e := \frac{1}{2} (u_{i,j}^e - u_{j,i}^e) = \frac{1}{2} \begin{bmatrix} 0 & u_{1,2}^e - u_{2,1}^e \\ u_{2,1}^e - u_{1,2}^e & 0 \end{bmatrix}. \quad (2.19)$$

From Eq. (2.19), we see that  $w_{ij}^e$  depends only on one function

$$\theta^e = \frac{1}{2} (u_{1,2}^e - u_{2,1}^e) = \frac{1}{2} \varepsilon_{ij} u_{i,j}^e, \quad (2.20)$$

which is known as the local rotation [31]. Thus, the rotation tensor  $w_{ij}^e$  can be written in index notation as

$$w_{ij}^e = \theta^e \varepsilon_{ij}. \quad (2.21)$$

Given the elastic displacement  $u_i^e(\mathbf{x})$  and local rotation field  $\theta^e(\mathbf{x})$ , we can detect discontinuities in the material by computing a contour integral that goes counter clockwise around a circle  $\Gamma(r)$  of radius  $r$  centered at  $\mathbf{x} = \mathbf{q}$ . The contour integral of local rotation picks up the wedge angle  $m$  while the displacement integral picks up Eq. (2.18), i.e.,

$$\oint_{\Gamma(r)} d\theta^e = m, \quad (2.22)$$

$$\oint_{\Gamma(r)} du_i^e = m_i r, \quad (2.23)$$

where the vector  $m_i$  can be written in polar-coordinate basis as  $\mathbf{m} = m\hat{\mathbf{e}}_\theta$ . Equations (2.22) and (2.23) constitute sufficient conditions for a disclination to exist at the center of the material.

The contour integrals in Eqs. (2.22) and (2.23) can also be used to derive the equivalent incompatibility source  $\eta(\mathbf{x})$  that reproduces the elastic fields from the Volterra construction via Eq. (2.17). To see this, we apply Green's theorem to Eq. (2.22) and find that

$$\oint_{\Gamma(r)} d\theta^e = \oint_{\Gamma(r)} \theta_{,k}^e d\mathcal{C}_k = \int_{S(r)} d^2\mathbf{x} \varepsilon_{lk} \theta_{,kl}^e = m. \quad (2.24)$$

where  $d\mathcal{C}_k$  is a line element that follows the circle and  $S(r)$  denotes a circular domain of radius  $r$ . Equation (2.24) can also be expressed in differential form by localizing the contour integral through the limit of  $r \rightarrow 0$ . Since Eq. (2.22) never vanishes for any value of  $r$ , this limit yields

$$\varepsilon_{lk} \theta_{,kl}^e = m \delta(\mathbf{x} - \mathbf{q}). \quad (2.25)$$

Green's theorem can also be applied to Eq. (2.23), where we find that

$$\oint_{\Gamma(r)} du_i^e = \oint_{\Gamma(r)} u_{i,j}^e d\mathcal{C}_j = \int_{S(r)} d^2\mathbf{x} \varepsilon_{kj} u_{i,jk}^e = m_i r. \quad (2.26)$$

Unlike the local rotation, the discontinuity in displacement vanishes as  $r \rightarrow 0$ , and thus localizing the contour yields

$$\varepsilon_{jk} u_{i,jk}^e = 0. \quad (2.27)$$

Note that if the elastic strain  $\epsilon_{ij}^e$  is expressed as the displacement gradient minus its anti-symmetric part, i.e.,

$$\epsilon_{ij}^e = u_{i,j}^e - w_{ij}^e = u_{i,j}^e - \theta^e \varepsilon_{ij}, \quad (2.28)$$

then the incompatibility condition in Eq. (2.6) can be re-expressed in terms of a linear combination of Eqs. (2.25) and (2.27). This yields,

$$\eta(\mathbf{x}) = \varepsilon_{ik} \varepsilon_{jl} (u_{i,jkl}^e - \theta_{,kl}^e \varepsilon_{ij}) \quad (2.29)$$

$$= \varepsilon_{ik} \theta_{,ki}^e = m \delta(\mathbf{x} - \mathbf{q}). \quad (2.30)$$

Applying the stress-function formalism of the compatibility condition in Eq. (2.17), we then find that

$$\frac{1}{Y} \nabla^4 \chi = m \delta(\mathbf{x} - \mathbf{q}). \quad (2.31)$$

By interpreting the stress function  $\chi(\mathbf{x})$  and Eq. (2.31) as the analogous electrostatic potential and Poisson's equation, respectively, the work in Ref. [3] proposes that a disclination may be interpreted as embedding a monopole of charge  $m$  into the solid (Fig. S.6(b)). The charge  $m$  then has the geometric meaning of the amount of local rotation experienced at the discontinuity.

**Dislocations as Dipoles:** The next Volterra construction involves performing a similar cut as a disclination, but yields a displacement discontinuity without a rotational discontinuity. In two dimensions, this can be done in two ways. The first construction yields a Mode I dislocation, and it involves cutting a thin rectangular slice with width  $b$  as shown in Fig. S.7(a), and gluing the

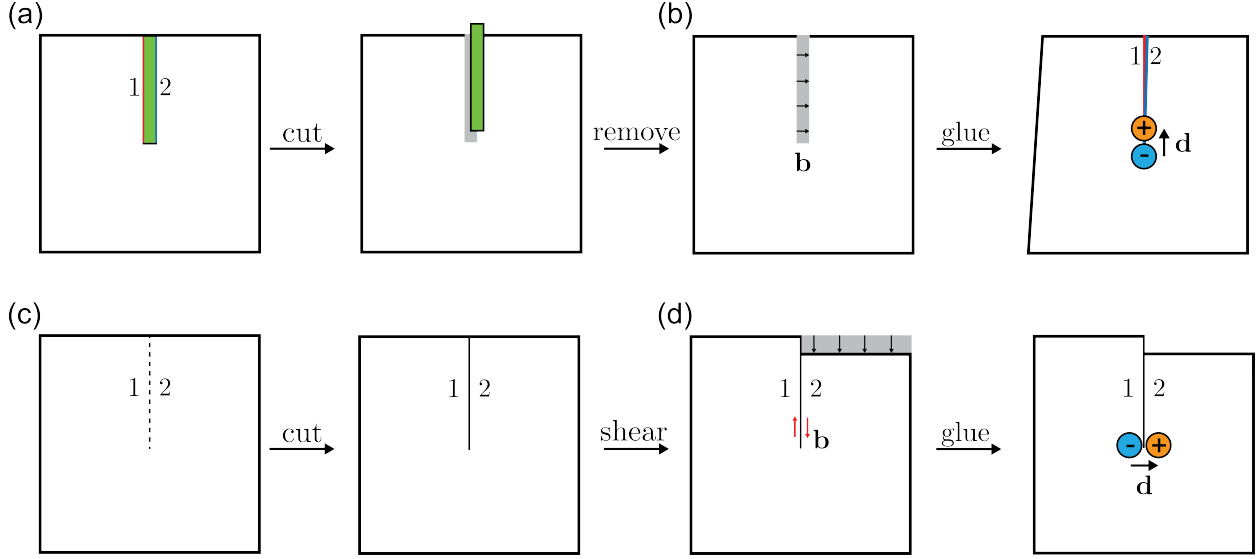

Figure S.7: (a) The Volterra construction that yields a Mode I dislocation. (b) Mode I dislocation as a dipole source in the incompatibility  $\eta(\mathbf{x})$ . (c) The Volterra construction that yields a Mode II dislocation. (d) Mode II dislocation as a dipole source. Both dislocations provide a localized source of translational displacement, distinguished only by the relative orientation of their cut with respect to the dipole-moment (or Burgers) vector.

two open sides together as in Fig. S.7(b). Along the thin cut, we produce a discontinuity in the displacement field without inducing any local rotation ( $\theta^e = 0$ ). The jump in  $u_\theta^e$  along the cut is

$$\llbracket u_\theta^e \rrbracket = b \text{ for Mode I dislocation.} \quad (2.32)$$

The second construction yields a Mode II dislocation, which is created by performing an infinitesimally small cut, and shearing the material instead as in Fig. S.7(c). Along the cut, we produce a displacement discontinuity that is perpendicular to the one made by a Mode I dislocation. In particular, the jump is now on the radial component, i.e.,

$$\llbracket u_r^e \rrbracket = b \text{ for Mode II dislocation.} \quad (2.33)$$

Unlike a disclination, the displacement jump in both dislocations is constant everywhere along the cut, all the way to the origin. But similar to a disclination, contour integrals of the local rotation and displacements can be used to state the sufficient conditions needed for a dislocation to exist at the center of the material. These integrals can be written as

$$\oint_{\Gamma(r)} d\theta^e = 0, \quad (2.34)$$

$$\oint_{\Gamma(r)} du_i^e = b_i, \quad (2.35)$$

where  $b_i$  is the so-called Burgers vector and may be written in polar basis as  $\mathbf{b} = b\hat{\mathbf{e}}_\theta$  (for Mode I) and  $\mathbf{b} = b\hat{\mathbf{e}}_r$  (for Mode II). Applying the steps used for disclinations, we can reduce the contour integrals into their local forms so that

$$\varepsilon_{lk}\theta_{,kl}^e = 0, \quad (2.36)$$

$$\varepsilon_{jk}u_{i,jk}^e = b_i\delta(\mathbf{x} - \mathbf{q}). \quad (2.37)$$

Substituting Eqs. (2.36) and (2.37) into Eq. (2.29), we find the following form for the incompatibility source:

$$\eta(\mathbf{x}) = \varepsilon_{ik}\varepsilon_{jkl}u_{i,jkl}^e = -\varepsilon_{il}b_i\delta(\mathbf{x} - \mathbf{q})_{,l} . \quad (2.38)$$

Switching the indices in Levi-Civita symbol, we then find in the stress-function form that

$$\frac{1}{Y}\nabla^4\chi = \varepsilon_{li}b_i\delta(\mathbf{x} - \mathbf{q})_{,l} . \quad (2.39)$$

Following the electrostatics analogy, one may also construct the localized source of  $\eta(\mathbf{x})$  in Eq. (2.38) directly from the monopoles/disclinations by putting two monopoles with opposite charges closely as in Fig. S.7(b). Let their separation distance be denoted as  $\mathbf{a}^m$ . The incompatibility source of two opposite monopoles can be written as

$$\eta(\mathbf{x}) = m\delta\left(\mathbf{x} - \left(\mathbf{q} + \frac{\mathbf{a}^m}{2}\right)\right) - m\delta\left(\mathbf{x} - \left(\mathbf{q} - \frac{\mathbf{a}^m}{2}\right)\right) \quad (2.40)$$

$$= -m a_l^m \delta(\mathbf{x} - \mathbf{q})_{,l} + \mathcal{O}\left(|\mathbf{a}^m|^2\right) . \quad (2.41)$$

Defining  $d_l = m a_l^m$  as the dipole moment vector, we may compare Eq. (2.41) with Eq. (2.38) and find that the Burgers vector is related to the dipole moment as

$$b_k = \varepsilon_{kl}d_l . \quad (2.42)$$

Since the 2D Levi-Civita tensor is equivalent to a 90° rotation matrix, Eq. (2.42) implies that the dipole moment is perpendicular to the Burgers vector, and the inner product  $b_i d_i = 0$ . Different modes of dipoles, e.g, Mode I or Mode II, can then be constructed based on the orientation angle of the cut with respect to the dipole-moment or Burgers vector.

**Point Defects as Quadrupoles:** The last Volterra construction involves an ellipsoidal cut at the center (Fig. S.8(a)), followed by putting the ellipsoid back into the material in a different orientation via an application of a uniform strain  $\epsilon_{ij}^c$  called an eigenstrain [32] (Fig. S.8(b)). This reduces the ellipsoidal cut to a single point, producing the so-called point defect. Unlike the previous defects, the elastic field outside of the defect core is always continuous, since the discontinuity is isolated at the center. In other words, the following contour integrals are identically zero,

$$\oint_{\Gamma(r)} d\theta^e = 0 , \quad (2.43)$$

$$\oint_{\Gamma(r)} du_i^e = 0 . \quad (2.44)$$

One way to define a point defect is by directly going into its defect strain  $\epsilon_{ij}^d$ . In particular, one may set the defect strain as

$$\epsilon_{ij}^d = \tilde{\epsilon}_{ij}^c \delta(\mathbf{x} - \mathbf{q}) , \quad (2.45)$$

where  $\tilde{\epsilon}_{ij}^c$  is proportional to the eigenstrain  $\epsilon_{ij}^c$  but with units length-squared instead. Using the definition of incompatibility (Eq. (2.6)), we find that

$$\eta(\mathbf{x}) = \left(-\varepsilon_{ik}\varepsilon_{jkl}\tilde{\epsilon}_{ij}^c\right)\delta(\mathbf{x} - \mathbf{q})_{,kl} . \quad (2.46)$$

An equivalent source of incompatibility can also be obtained by forming a quadrupole, i.e., a bound-dipole pair as shown in Fig. S.8(b). Its incompatibility source can be mapped to the one

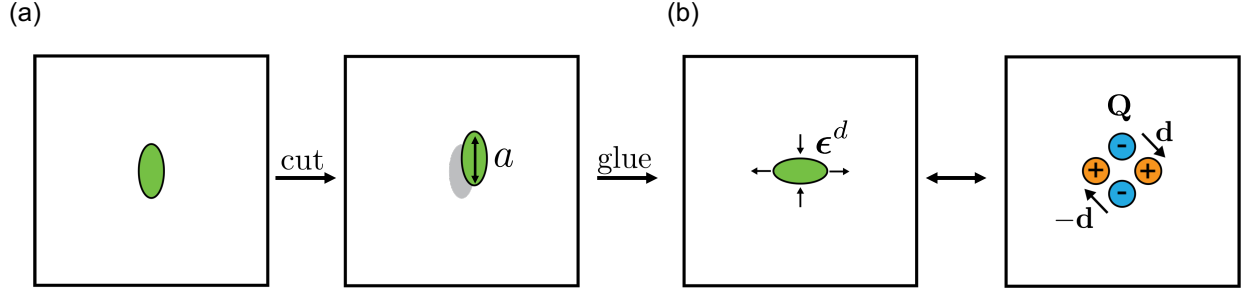

Figure S.8: (a) The Volterra construction that yields a point defect in a solid, i.e., localized source of defect strain. (b) Point defect as a quadrupole source in the incompatibility  $\eta(\mathbf{x})$ .

defined in Eq. (2.46). To this end, let  $\mathbf{a}^{\text{dpl}}$  be the pair-distance vector connecting the center of mass of one dipole to the next one. Following the same strategy as the dipole-dislocation correspondence, we can Taylor expand the monopole sources up to second order and obtain the following incompatibility source:

$$\eta(\mathbf{x}) = \left( d_k a_l^{\text{dpl}} \right)_{\text{sym}} \delta(\mathbf{x} - \mathbf{q})_{,kl} + \mathcal{O}(|\mathbf{a}^{\text{dpl}}|^2) + \mathcal{O}(|\mathbf{a}^{\text{m}}|^2) + \mathcal{O}(\mathbf{a}^{\text{dpl}} \cdot \mathbf{a}^{\text{m}}), \quad (2.47)$$

where  $(d_i a_j^{\text{dpl}})_{\text{sym}}$  is the symmetric part of the dyadic product between the dipole-moment vector  $\mathbf{d}$  and the pair-distance vector  $\mathbf{a}_{\text{dpl}}$ . More generally, a quadrupole incompatibility source is specified by a quadrupole tensor  $Q_{ij}$  so that

$$\eta(\mathbf{x}) = Q_{kl} \delta(\mathbf{x} - \mathbf{q})_{,kl}, \quad (2.48)$$

where the quadrupole tensor for a pair of dipoles like in Fig. S.8(b) is

$$Q_{kl} = \left( d_i a_j^{\text{dpl}} \right)_{\text{sym}} = \frac{1}{2} \left( d_i a_j^{\text{dpl}} + d_j a_i^{\text{dpl}} \right). \quad (2.49)$$

Given the more general source in Eq. (2.48), we can compare it with Eq. (2.46) to obtain

$$\tilde{\epsilon}_{ij}^c = -\varepsilon_{ik} \varepsilon_{jl} Q_{kl}. \quad (2.50)$$

Note that the trace  $\tilde{\epsilon}_{ii}^c = -\varepsilon_{ik} \varepsilon_{il} Q_{kl} = -Q_{kk}$ . If  $\mathbf{Q}$  is traceless, then the corresponding eigenstrain is also traceless, i.e., the defect strain is of pure-shear type. Thus, quadrupoles can also be used to model localized pure-shear excitations, which were previously modeled in previous work [7] via the force-dipole formalism [32].

**Application to the Inherent States:** We now have two ways to model elastic defects, which are the Volterra construction and the framework of geometric charges. For all subsequent analyses, we use the latter framework because it is generalizable to model defects of any kind without resorting to macroscopic cutting/welding procedures. In addition, we shall see in Section 2.4 how the geometric-charges framework allows us to derive conservation laws that restrict the allowable defect configurations. Such constraints are important when studying the statistical mechanics of excitations in supercooled liquids. In the next section (Section 2.3), we derive the admissible boundary conditions via variational calculus that will supplement the analysis in Section 2.4

### 2.3 Variational Principles and Boundary Conditions

To prepare our discussions on the energetics of geometric charges in an elastic medium, we need to derive the total strain energy in terms of the stress function  $\chi(\mathbf{x})$ , as well as the appropriate boundary conditions in terms of  $\chi(\mathbf{x})$ . The total energy of a linear elastic medium is defined as

$$\Delta U = \frac{1}{2} \int d^2\mathbf{x} T_{ij}^e \epsilon_{ij}^e = G \int d^2\mathbf{x} \left( \epsilon_{ij}^e \epsilon_{ij}^e + \frac{\nu}{1-\nu} \epsilon_{kk}^e \epsilon_{ll}^e \right), \quad (2.51)$$

where we used Eq. (2.8) for an isotropic linear elastic medium. Substituting the strain-stress-function relation Eq. (2.16) in Eq. (2.51), we obtain

$$\Delta U = \frac{1}{2Y} \int d^2\mathbf{x} [(1+\nu) \chi_{,ij} \chi_{,ij} - \nu \chi_{,kk} \chi_{,ll}]. \quad (2.52)$$

From Eq. (2.52), we can deduce the appropriate boundary conditions for the stress functions via variational calculus [33]. First, we consider the variation of  $\Delta U$  by introducing a variation in the stress function  $\delta\chi$ . Up to linear order  $\delta\chi$ , we find that

$$\delta(\Delta U) = \frac{1}{Y} \int d^2\mathbf{x} [(1+\nu) \chi_{,ij} (\delta\chi)_{,ij} - \nu \chi_{,kk} (\delta\chi)_{,ll}]. \quad (2.53)$$

After integrating by parts and using divergence theorem, we then arrive at

$$\begin{aligned} \delta(\Delta U) &= \frac{(1+\nu)}{Y} \int d\mathcal{C} n_j \chi_{,ij} (\delta\chi)_{,i} - \frac{(1+\nu)}{Y} \int d^2\mathbf{x} \chi_{,ijj} (\delta\chi)_{,i} \\ &\quad - \frac{\nu}{Y} \int d\mathcal{C} n_l \chi_{,kk} (\delta\chi)_{,l} + \frac{\nu}{Y} \int d^2\mathbf{x} \chi_{,kkl} (\delta\chi)_{,l} \end{aligned} \quad (2.54)$$

$$= \frac{(1+\nu)}{Y} \int d\mathcal{C} n_j \chi_{,ij} (\delta\chi)_{,i} - \frac{\nu}{Y} \int d\mathcal{C} n_l \chi_{,kk} (\delta\chi)_{,l} - \frac{1}{Y} \int d^2\mathbf{x} \chi_{,ijj} (\delta\chi)_{,i}, \quad (2.55)$$

where  $n_l$  is the normal vector of the system's boundary. As a last step, we again integrate by parts on the last term of Eq. (2.55) leading to

$$\begin{aligned} \delta(\Delta U) &= \frac{(1+\nu)}{Y} \int d\mathcal{C} n_j \chi_{,ij} (\delta\chi)_{,i} - \frac{\nu}{Y} \int d\mathcal{C} n_l \chi_{,kk} (\delta\chi)_{,l} \\ &\quad - \frac{1}{Y} \int d\mathcal{C} n_i \chi_{,ijj} (\delta\chi) + \frac{1}{Y} \int d^2\mathbf{x} \chi_{,ijjj} (\delta\chi). \end{aligned} \quad (2.56)$$

Through Eq. (2.56), we can set the total variation in energy to be zero by setting the following partial differential equation to be zero in the interior of the system,

$$\frac{1}{Y} \chi_{,iijj} = 0, \quad (2.57)$$

which is equivalent to Eq. (2.17) in index notation when no defects are present, and setting the following set of equations to be zero at the boundaries,

$$\frac{1}{Y} (-n_j \chi_{,ii j}) (\delta\chi) = 0, \quad (2.58a)$$

$$\frac{1}{Y} [-\nu \chi_{,kk} n_j + (1+\nu) n_j \chi_{,ij}] (\delta\chi)_{,j} = 0. \quad (2.58b)$$

In the language of variational calculus, we can choose the so-called essential boundary conditions by setting the variation  $\delta\chi = 0$  to satisfy Eq. (2.58a) and its gradient  $\delta\chi_{,k} = 0$  to satisfy Eq. (2.58b). The so-called natural boundary conditions are obtained when we set  $-n_j\chi_{,ij} = 0$  to satisfy Eq. (2.58a) and  $-\nu\chi_{,kk}n_j + (1+\nu)n_j\chi_{,ij} = 0$  to satisfy Eq. (2.58b). Note that if non-zero tractions are present on the boundaries, then a more general set of natural boundary conditions  $-\frac{1}{Y}n_j\chi_{,ij} = \bar{\alpha}$  and  $-\frac{1}{Y}(\nu\chi_{,kk}n_j + (1+\nu)n_j\chi_{,ij}) = \bar{\beta}$ , where  $\bar{\alpha}$  and  $\bar{\beta}$  are non-zero constants, may be found that still leave the total variation  $\delta(\Delta U) = 0$ .

The boundary conditions in Eqs. (2.58a) and (2.58b) can also be expressed in terms of stresses  $T_{ij}$  and hydrostatic pressure  $p = -T_{ii}/2 = -\chi_{,ii}/2$ . Given the definition of pressure, we find that Eq. (2.58a) becomes

$$\frac{1}{Y}(2p_{,j}n_j)(\delta\chi) = 0. \quad (2.59)$$

Thus, one of the natural boundary conditions is to set the gradient of the pressure along the normal to be zero ( $p_{,j}n_j = 0$ ). Using Eq. (2.11), Eq. (2.58b) is written as

$$\frac{1}{Y}(-2pn_i - (1+\nu)T_{ij}^e n_j)(\delta\chi)_{,i} = 0. \quad (2.60)$$

Eq. (2.60) relates the traction ( $T_{ij}^e n_j$ ) observed at the boundary of the system with the pressure. While we are free to choose any combination of natural and essential boundary conditions, the next section (Section 2.4) will show that the boundary conditions appropriate for studying a system of defects are related to the natural boundary conditions.

## 2.4 Conservation Laws for Geometric Charges

By modeling elastic defects via analogy with electrostatics, we also obtain conservation laws that are analogous to Gauss' law in electrostatics. Specializing to isotropic systems, we derive a charge conservation law from Eq. (2.17), which is written in index notation as

$$\eta(\mathbf{x}) = \frac{1}{Y}\chi_{,iijj}. \quad (2.61)$$

Integrating Eq. (2.61) over space, we find

$$\int d^2\mathbf{x} \eta(\mathbf{x}) = \frac{1}{Y} \int d^2\mathbf{x} \chi_{,iijj}. \quad (2.62)$$

Applying divergence theorem yields

$$\int d^2\mathbf{x} \eta(\mathbf{x}) = \frac{1}{Y} \int d\mathcal{C} n_j \chi_{,iij}. \quad (2.63)$$

The pressure in the medium is expressed in terms of the Airy stress function as  $p = -\chi_{,ii}/2$ , and thus

$$\int d^2\mathbf{x} \eta(\mathbf{x}) = -\frac{2}{Y} \int d\mathcal{C} n_j p_j. \quad (2.64)$$

**Charge Conservation:** Defining the total charge  $Q$  in the system as  $Q = \int d^2\mathbf{x} \eta(\mathbf{x})$  and considering the case of a population of monopoles with allowable charges  $m^\mu = \pm m$ , the left part of Eq. (2.64) becomes

$$Q = \int d^2\mathbf{x} \eta(\mathbf{x}) = \int d^2\mathbf{x} \sum_{\mu} m^\mu \delta(\mathbf{x} - \mathbf{q}^\mu) = \sum_{\mu} m^\mu.$$

For the case of  $Q = 0$ , we observe that the right part of Eq. (2.64) is zero. This condition can be satisfied either globally, where the integral of  $n_j p_j$  along the boundary vanishes, or when  $n_j p_j = 0$  identically. The latter result is the natural boundary conditions of Eq. (2.59) deduced through the variational approach described in Section 2.3.

**Dipole Conservation:** We can also obtain an additional conservation law by multiplying both sides of Eq. (2.61) with  $\mathbf{x}$  and integrating over volume, which yields

$$\int d^2\mathbf{x} x_k \eta(\mathbf{x}) = \frac{1}{Y} \int d^2\mathbf{x} x_k \chi_{,iijj}. \quad (2.65)$$

Applying integration by parts and divergence theorem, the right part of Eq. (2.65) becomes

$$\int d^2\mathbf{x} x_k \eta(\mathbf{x}) = \frac{1}{Y} \int d\mathcal{C} n_j x_k \chi_{,iij} - \frac{1}{Y} \int d^2\mathbf{x} \chi_{,iik} \quad (2.66)$$

$$= -\frac{2}{Y} \int d\mathcal{C} n_j x_k p_{,j} + \frac{2}{Y} \int d^2\mathbf{x} p_{,k}, \quad (2.67)$$

where the second equality is obtained by incorporating the definition of pressure as before. We can further use divergence theorem in the last term, which leads to

$$\int d^2\mathbf{x} x_k \eta(\mathbf{x}) = -\frac{2}{Y} \int d\mathcal{C} n_j x_k p_{,j} + \frac{2}{Y} \int d\mathcal{C} n_k p. \quad (2.68)$$

Defining the total dipole moment as  $P_k = \int d^2\mathbf{x} x_k \eta(\mathbf{x})$ , for a system of dipoles with  $\eta(\mathbf{x}) = \sum_\mu d_j^\mu \delta(\mathbf{x} - \mathbf{q}^\mu)_{,j}$  we find

$$P_k = \int d^2\mathbf{x} x_k \eta(\mathbf{x}) = \int d^2\mathbf{x} x_k \sum_\mu d_j^\mu \delta(\mathbf{x} - \mathbf{q}^\mu)_{,j} = \sum_\mu d_k^\mu,$$

where in the third equality we integrated by parts. By definition, a system of dipoles satisfy  $Q = 0$ , which according to Eq. (2.64) makes the first integral in Eq. (2.68) to vanish, and thus

$$P_k = \frac{2}{Y} \int d\mathcal{C} n_k p. \quad (2.69)$$

Additionally, when the total dipole moment  $P_k = 0$ , we may find that the pressure  $p = 0$  at the boundaries. When combined with the natural boundary condition implied in Eq. (2.60), zero pressure at the boundaries leads to traction-free boundary condition, i.e.,  $T_{ij}^e n_j = 0$ .

To summarize, charge  $Q$  and dipole-moment  $P_k$  neutrality imply the following natural boundary conditions:

$$p = 0, \quad (2.70a)$$

$$n_j p_{,j} = 0, \quad (2.70b)$$

$$T_{ij}^e n_j = 0. \quad (2.70c)$$

These boundary conditions are useful not only for analyzing finite-size systems but also when determining integration constants arising from the fundamental solutions of the Airy stress function, as we shall see in Section 2.5.

## 2.5 Airy Stress Function Fundamental Solutions

We now proceed to establishing the fundamental solution (Green's function)  $G(\mathbf{x} - \mathbf{x}')$  of the partial differential equation that arises in Eq. (2.17). Using the Green's function and the superposition principle, we can then express  $\chi$  for a general distribution of charges.

The fundamental solution that satisfies  $\frac{1}{Y}\nabla^4 G(\mathbf{x}) = \delta(\mathbf{x})$  is known to be (Problem 9.9 in [31] and Eq. (2.12) in [9])

$$G(\mathbf{x}) = \frac{Y}{8\pi} r^2 (\ln r + A) + B, \quad (2.71)$$

where  $A, B$  are undetermined integration constants. The general solution of the Airy stress function when a distribution of defects  $\eta(\mathbf{x})$  is present can then be written as

$$\chi(\mathbf{x}) = \int d^2\mathbf{x}' G(\mathbf{x} - \mathbf{x}') \eta(\mathbf{x}'). \quad (2.72)$$

We now specialize the solution to each class of defects introduced in Section 2.2: a single monopole with charge  $m^\mu$ , a single dipole with dipole moment  $\mathbf{d}^\mu$  and a single quadrupole with quadrupole tensor  $\mathbf{Q}^\mu$ .

**Monopole:** For a geometric monopole of strength  $m^\mu$  located at the origin, we apply Eq. (2.30) to Eq. (2.72) leading to

$$\chi(\mathbf{x}) = \int d^2\mathbf{x}' G(\mathbf{x} - \mathbf{x}') m^\mu \delta(\mathbf{x}') = \frac{Y m^\mu}{8\pi} r^2 (\ln r + A) + B. \quad (2.73)$$

To determine one of the integration constants, we may use the natural boundary conditions, in particular the vanishing pressure condition Eq. (2.70a). Let  $R$  be the system size for a material shaped as a circle. Equation (2.70a) is equivalent to setting the radial component of the stress  $T_{rr}$  to be zero at  $r = R$  [34]. This condition results in  $A = -\frac{1}{2} - \ln R$ , and Eq. (2.73) becomes

$$\chi(\mathbf{x}) = \frac{Y m^\mu}{8\pi} r^2 \left( \ln \frac{r}{R} - \frac{1}{2} \right) + B. \quad (2.74)$$

Since we are dealing with monopoles, charge conservation is also upheld, which implies the natural boundary condition  $p_{,j} n_j = 0$ . From variational calculus, we know that all-natural boundary conditions lead to one undetermined constant in the solution, and in the monopole case, this corresponds to the constant  $B$  in Eq. (2.74). This constant can only be fixed with extra conditions pertaining to the physical setup of the problem.

**Dipole:** In the case of a geometric dipole of strength  $d_c^\mu = \sqrt{d_i^\mu d_i^\mu}$  located at the origin,  $\eta(\mathbf{x})$  is given by Eq. (2.41), which results in

$$\chi(\mathbf{x}) = - \int d^2\mathbf{x}' G(\mathbf{x} - \mathbf{x}') d_k^\mu \delta(\mathbf{x}')_{,k} = \int d^2\mathbf{x} \frac{\partial G}{\partial x_k} d_k^\mu \delta(\mathbf{x}') = -\frac{Y}{4\pi} d_i^\mu x_i (\ln r + C), \quad (2.75)$$

where  $C \equiv A + \frac{1}{2}$  and in the second equality we performed integration by parts, discarding boundary terms as they vanish identically due to the delta function. Unlike the monopoles, the constant  $C$  cannot be determined via the natural boundary conditions. To see this, note that the pressure arising from a dipole can be written as

$$p(\mathbf{x}) = -\frac{\chi_{,kk}}{2} = \frac{Y d_c^\mu}{4\pi r} \cos(2\theta - 2\psi^\mu), \quad (2.76)$$

where  $\psi^\mu$  is the orientation angle of the dipole moment vector. Equation (2.76) is independent of  $C$  and also vanishes at  $r = R$  when  $R \rightarrow \infty$ . Thus, the constant  $C$  for a dipole needs to be determined via a different closure relation.

However, without loss of generality, we may re-define the  $C$  constant so as to introduce a logarithmic system-size dependence into the solution. This re-definition turns Eq. (2.75) into

$$\chi(\mathbf{x}) = -\frac{Y}{4\pi} d_i^\mu x_i \left( \ln \frac{r}{R} + C \right). \quad (2.77)$$

In this form, the lengthscale inside the logarithmic term is compatible with the monopole solution. For all subsequent analyses pertaining to the dipoles, we use Eq. (2.77) instead of Eq. (2.75).

**Quadrupole:** Finally, we are also interested in the Airy stress function generated by a geometric quadrupole  $\mathbf{Q}^\mu$  located at the origin. The source of incompatibility is Eq. (2.48), which leads to

$$\begin{aligned} \chi(\mathbf{x}) &= \int d^2\mathbf{x}' G(\mathbf{x} - \mathbf{x}') Q_{kl}^\mu \delta(\mathbf{x}')_{,kl} = \int d^2\mathbf{x}' \frac{\partial^2 G}{\partial x_k \partial x_l} Q_{kl}^\mu \delta(\mathbf{x}') \\ &= \frac{Y}{4\pi} \left[ Q_{ii}^\mu \left( \ln \frac{r}{R} + C \right) + \frac{x_i Q_{ij}^\mu x_j}{r^2} \right]. \end{aligned} \quad (2.78)$$

When  $\mathbf{Q}^\mu$  is a symmetric traceless tensor, the first term at the end result is identically zero. This yields,

$$\chi(\mathbf{x}) = \frac{Y x_i Q_{ij}^\mu x_j}{4\pi r^2} \quad \text{for } Q_{ii}^\mu = 0. \quad (2.79)$$

Equations (2.73), (2.77) and (2.79) are essential to understand the thermodynamics of these geometric charges, which is relevant in the context of statistical mechanics of excitations in supercooled liquids.

### 3 Energy–Entropy Arguments and Interaction Energies

In this section, we use the framework of geometric charges to model excitations in supercooled liquids, particularly those that are relevant for understanding the onset temperature  $T_o$  of glassy dynamics. To this end, we develop energy-entropy arguments for the geometric monopole, dipole, and quadrupoles in Section 3.1. Here, we deduce that dipoles yield a critical temperature  $T_c$  that may correspond to  $T_o$ . By choosing dipoles as the fundamental units of excitation, we derive their interaction energy in Section 3.2 and demonstrate their connection (at  $T \ll T_c$ ) to localized pure-shear excitations developed in previous work [7]. This motivates a mapping in Section 3.3 between the parameters of the geometric dipole, i.e., dipole magnitude  $d_c$  and constant  $C$  in Eq. (2.77), to the parameters defining localized pure-shear excitations.

#### 3.1 Free Energy Arguments for Geometric Charges

We are interested in understanding the conditions for which the formation of a single geometric monopole, dipole, and quadrupole is thermodynamically favored within an isotropic elastic solid. In the context of supercooled liquids, each class of defects constitutes a plausible candidate for excitations, with the solid corresponding to the initial inherent state. The goal is to screen these possible candidates and figure out which defect yields a critical transition temperature  $T_c$  that may be associated with the onset temperature  $T_o$ .

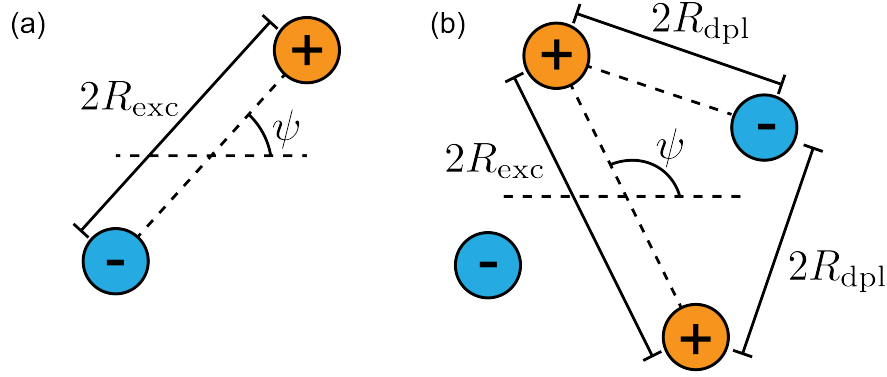

Figure S.9: Schematic of geometric (a) dipole and (b) quadrupole considered in the energy-entropy arguments. In (a), the diameter of excitation  $2R_{\text{exc}}$  corresponds to the length of the dipole. In (b), the size of excitation corresponds to the distance between two monopoles of equal charges. For the present geometric model of quadrupoles,  $2R_{\text{dpl}} = \sqrt{2}R_{\text{exc}}$ .

### Partition Function and Free Energy of Formation

To formulate the energy-entropy arguments, we need to evaluate the single-excitation partition function. Since the energetics only involve the self-energy  $\bar{E}_c$ , the appropriate partition function is  $\bar{Q}_{\text{iso}, N_{\text{exc}}}$  for  $N_{\text{exc}} = 1$  as given by Eq. (1.36) from Section 1.2. For a single excitation, we can write Eq. (1.36) as

$$\bar{Q}_{\text{iso},1} = \frac{1}{R_{\text{exc}}^2 1!} \int d^2 \mathbf{q} \int d^{d_{\text{int}}} \mathbf{s} e^{-\beta \bar{E}_c} = e^{-\beta \bar{E}_c} \left( \frac{R}{R_{\text{exc}}} \right)^2 \left( \int d^{d_{\text{int}}} \mathbf{s} \right), \quad (3.1)$$

where  $R_{\text{exc}}$  and  $R$  correspond to the radius of excitation and the size of the domain, respectively. The free energy of formation  $\Delta F_f$  is then related to  $\bar{Q}_{\text{iso},1}$  through  $\Delta F_f = -k_B T \ln \bar{Q}_{\text{iso},1}$ .

The self-energy  $\bar{E}_c$  is evaluated from the strain field due to a single excitation  $\epsilon_{ij}^\mu$  by substituting the stiffness tensor Eq. (2.14) into the self-energy formula in Eq. (1.24). This yields

$$\bar{E}_c = G^{\text{IS}} \int d^2 \mathbf{x} \left( \epsilon_{ij}^\mu \epsilon_{ij}^\mu + \frac{\nu^{\text{IS}}}{1 - \nu^{\text{IS}}} \epsilon_{kk}^\mu \epsilon_{ll}^\mu \right). \quad (3.2)$$

We can use the strain-stress-function relation in Eq. (2.16) to write Eq. (3.2) in terms of the stress function, i.e.,

$$\bar{E}_c = \frac{1}{2Y^{\text{IS}}} \int d^2 \mathbf{x} \left[ (1 + \nu^{\text{IS}}) \chi_{,ij}^\mu \chi_{,ij}^\mu - \nu^{\text{IS}} \chi_{,kk}^\mu \chi_{,ll}^\mu \right]. \quad (3.3)$$

The integration in Eq. (3.3) can be expressed in terms of polar coordinates as follows

$$\bar{E}_c = \frac{1}{2Y^{\text{IS}}} \int_0^{2\pi} d\theta \int_{R_{\text{exc}}}^R r dr \left[ (1 + \nu^{\text{IS}}) \chi_{,ij}^\mu \chi_{,ij}^\mu - \nu^{\text{IS}} \chi_{,kk}^\mu \chi_{,ll}^\mu \right]. \quad (3.4)$$

Using the stress-function solutions for monopoles, dipoles and quadrupoles, Eqs. (2.73), (2.77) and (2.79), respectively, we can evaluate  $\bar{E}_c$ , and therefore their respective free energy of formation.

**Monopole:** For a single monopole with charge  $m$  we substitute Eq. (2.73) in Eq. (3.4), and perform the integration to find

$$\bar{E}_c = \frac{m^2 Y^{\text{IS}}}{32\pi} \left[ 1 - \left( \frac{R_{\text{exc}}}{R} \right)^2 \left( 1 + 2(1 - \nu^{\text{IS}}) \ln \left( \frac{R_{\text{exc}}}{R} \right)^2 \right) \right] R^2 \simeq \frac{m^2 Y^{\text{IS}}}{32\pi} R^2, \quad (3.5)$$

where  $m$  is the magnitude of the monopole and the final equality is considered under the limit  $R_{\text{exc}}/R \rightarrow 0$ . The partition function  $\bar{Q}_{\text{iso},1}$  becomes

$$\bar{Q}_{\text{iso},1} = e^{-\beta \bar{E}_c} \left( \frac{R}{R_{\text{exc}}} \right)^2 \simeq \exp \left( -\frac{m^2 \beta Y^{\text{IS}}}{32\pi} R^2 \right) \left( \frac{R}{R_{\text{exc}}} \right)^2, \quad (3.6)$$

which leads to the following free energy of formation for the monopoles:

$$\Delta F_{\text{f}}^{\text{mnpl}} \simeq \frac{m^2 Y^{\text{IS}}}{32\pi} R^2 - 2k_{\text{B}} T \ln \left( \frac{R}{R_{\text{exc}}} \right). \quad (3.7)$$

From Eq. (3.7), we observe that

$$\lim_{R \rightarrow \infty} \Delta F_{\text{f}}^{\text{mnpl}} \simeq \lim_{R \rightarrow \infty} \frac{m^2 Y^{\text{IS}}}{32\pi} R^2 \rightarrow +\infty, \quad (3.8)$$

and thus geometric monopoles are not thermodynamically favored at any temperature.

**Dipole:** A single dipole consists of two monopoles located at  $\mathbf{x} = \pm \frac{\mathbf{a}_m}{2} = \pm R_{\text{exc}} [\cos \psi, \sin \psi]$  with  $\mathbf{d} = m\mathbf{a}^m$ , as shown in Fig. S.9(a). Using Eqs. (2.77) and (3.4), the self-energy is

$$\bar{E}_c = \frac{m^2 R_{\text{exc}}^2 Y^{\text{IS}}}{2\pi} \ln \left( \frac{R}{R_{\text{exc}}} \right) = \frac{d_c^2 Y^{\text{IS}}}{8\pi} \ln \left( \frac{R}{R_{\text{exc}}} \right), \quad (3.9)$$

where  $d_c = 2mR_{\text{exc}}$  is the magnitude of the dipole moment. Given that the internal degree of freedom is just the orientation angle  $\psi$ ,  $\int d^{\text{int}} \mathbf{s}^\mu = \int_0^{2\pi} d\psi = 2\pi$  and with Eq. (3.9), Eq. (3.1) becomes

$$\bar{Q}_{\text{iso},1} = 2\pi e^{-\beta \bar{E}_c} \left( \frac{R}{R_{\text{exc}}} \right)^2 = 2\pi \left( \frac{R}{R_{\text{exc}}} \right)^{2 - \frac{d_c^2 \beta Y^{\text{IS}}}{8\pi}}. \quad (3.10)$$

The free energy formation for a dipole becomes

$$\Delta F_{\text{f}}^{\text{dpl}} = -k_{\text{B}} T \ln(2\pi) + \left( \frac{d_c^2 Y^{\text{IS}}}{8\pi} - 2k_{\text{B}} T \right) \ln \left( \frac{R}{R_{\text{exc}}} \right). \quad (3.11)$$

From Eq. (3.11), we observe two limiting cases. For  $k_{\text{B}} T > \frac{d_c^2 Y^{\text{IS}}}{16\pi}$ , free energy of formation is negative and in the limit of large system size  $\Delta F_{\text{f}}^{\text{dpl}} \rightarrow -\infty$ . This implies that dipoles are entropically favored at high temperatures. For  $k_{\text{B}} T < \frac{d_c^2 Y^{\text{IS}}}{16\pi}$ , the limit  $R \rightarrow \infty$  leads to  $\Delta F_{\text{f}}^{\text{dpl}} \rightarrow \infty$ , indicating that dipoles do not form naturally in the medium.

**Quadrupole:** Here, we consider a quadrupole made of four monopoles consisting of two positive and negative charges of magnitude  $m$ ; see Fig. S.9(b) that shows a schematic representation of the quadrupole geometry. The two positive charges are located at  $\mathbf{x}_+ = \pm \mathbf{a} = \pm R_{\text{exc}} [\cos \psi, \sin \psi]$  while the two negative charges are located at  $\mathbf{x}_- = \pm \boldsymbol{\varepsilon} \mathbf{a} = \pm R_{\text{exc}} (\sin \psi, -\cos \psi)$ , where  $\boldsymbol{\varepsilon}$  is the Levi-Civita tensor. For this configuration, the quadrupole tensor  $\mathbf{Q}$  defined in Eq. (2.49) becomes

$$\mathbf{Q} = m R_{\text{exc}}^2 \begin{bmatrix} \cos 2\psi & \sin 2\psi \\ \sin 2\psi & -\cos 2\psi \end{bmatrix}, \quad (3.12)$$

where  $Q_{ii} = 0$  and  $Q_{ij} = Q_{ji}$ . Using Eq. (2.79) to evaluate  $\bar{E}_c$  in Eq. (3.4), we find

$$\bar{E}_c = \frac{m^2 R_{\text{exc}}^2 Y^{\text{IS}} (3 + \nu^{\text{IS}})}{8\pi} \left( 1 - \left( \frac{R_{\text{exc}}}{R} \right)^2 \right) \simeq \frac{d_c^2 Y^{\text{IS}} (3 + \nu^{\text{IS}})}{16\pi} \quad (3.13)$$

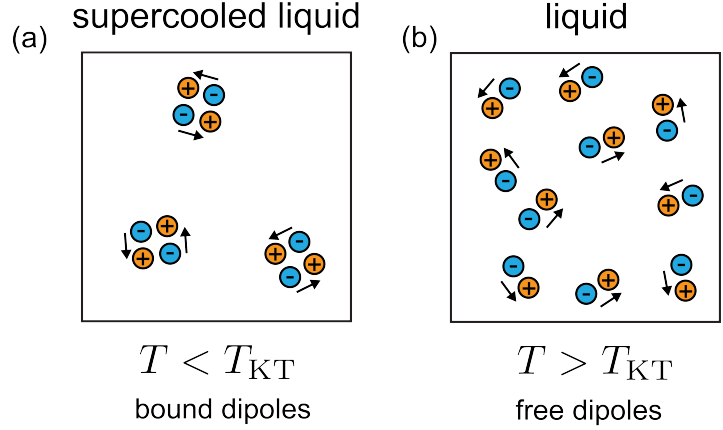

Figure S.10: An illustration of the binding-unbinding transition between free dipoles and bound-dipole pairs (quadrupoles). The existence of the critical temperature  $T_{KT}$  can be found via energy-entropy argument, although more careful analysis requires understanding of the interaction between dipoles.

for  $R_{exc}/R \rightarrow 0$  and  $d_c^2 = 2m^2 R_{exc}^2$ . Then, the partition function becomes

$$\bar{Q}_{iso,1} = 2\pi e^{-\beta \bar{E}_c} \left( \frac{R}{R_{exc}} \right)^2 \simeq 2\pi \exp \left( -\frac{\beta d_c^2 Y^{IS} (3 + \nu^{IS})}{16\pi} \right) \left( \frac{R}{R_{exc}} \right)^2, \quad (3.14)$$

and the free energy formation for a quadrupole is

$$\Delta F_f^{qdpl} \simeq \frac{d_c^2 Y^{IS} (3 + \nu^{IS})}{16\pi} - k_B T \ln(2\pi) - 2k_B T \ln \left( \frac{R}{R_{exc}} \right). \quad (3.15)$$

In the limit of large system sizes, we observe from Eq. (3.15) that

$$\lim_{R \rightarrow \infty} \Delta F_f^{qdpl} \rightarrow -\infty$$

at any temperature  $T$ . This result indicates that quadrupoles can form due to entropic reasons, even though there is a finite energetic cost to form bound-dipole pairs.

### Existence of a Binding-Unbinding Transition

The analysis for dipoles indicates that there exists a critical temperature  $k_B T_c = d_c^2 Y / 16\pi$  where free dipoles proliferate at high enough temperatures, and become rare at sufficiently low temperatures. Such critical temperature may be a possible candidate for the onset temperature for glassy dynamics. On the other hand, it is also possible for bound-dipole pairs (quadrupoles) to exist at any temperature, as indicated by the free energy in Eq. (3.15). These two observations seem to imply that there may exist a binding-unbinding transition between free dipoles and bound-dipole pairs, as illustrated in Fig. S.10. This conjectured transition can be formalized in the form an energy-entropy argument by comparing the free energy formation between one quadrupole and two free dipoles as follows

$$\Delta F_{qdpl \rightarrow dpls} = F_{dpls} - F_{qdpl} = \Delta F_f^{dpls} - \Delta F_f^{qdpl}, \quad (3.16)$$

where in the last equality we added and subtracted the empty state to express  $\Delta F_{qdpl \rightarrow dpls}$  in terms of the free energy of formation of two dipoles  $\Delta F_f^{dpls}$  and a quadrupole  $\Delta F_f^{qdpl}$ , respectively. The

quadrupolar free energy is given by Eq. (3.15), while  $\Delta F_f^{\text{dpls}}$  can be approximated by the free energy of formation of two non-interacting dipoles. Such an approximation implies  $\bar{Q}_{\text{iso},2}^{\text{dpls}} \simeq (\bar{Q}_{\text{iso},1}^{\text{dpl}})^2 / 2!$ , and thus Eq. (3.16) becomes

$$\Delta F_{\text{qdpl} \rightarrow \text{dpls}} \simeq \left( \frac{d_c^2 Y^{\text{IS}}}{4\pi} - 2k_B T \right) \ln \left( \frac{R}{R_{\text{exc}}} \right) - k_B T \ln \left( \frac{\pi}{2} \right) - \frac{d_c^2 Y^{\text{IS}} (3 + \nu)}{16\pi}. \quad (3.17)$$

From this result, we find that  $\Delta F_{\text{qdpl} \rightarrow \text{dpls}}$  is negative for  $k_B T > \frac{d_c^2 Y^{\text{IS}}}{8\pi}$ , which is twice of that predicted by the free energy argument for dipoles. At these high temperatures, free dipoles are thermodynamically favored while at low enough temperatures ( $k_B T < \frac{d_c^2 Y^{\text{IS}}}{8\pi}$ ), the system favors the formation of bound-dipole pairs at low temperatures. This new critical transition is twice the transition temperature predicted by the free energy argument for the dipoles (Eq. (3.11)). Such a result contradicts the existence of a single binding-unbinding transition temperature. However, the discrepancy may be understood as a result of neglecting the interaction between two dipoles, since  $\bar{Q}_{\text{iso},2}^{\text{dpls}}$  is approximated in terms of its non-interacting counterparts. Thus, a more careful analysis involving the interaction energies is needed to resolve this discrepancy.

The scenario we have described is similar to the one found in the Kosterlitz-Thouless-Halperin-Nelson-Young (KTHNY) theory for dislocation-mediated melting [5, 8–11]. In the KTHNY theory, we have a bound-dislocation pair with opposing Burgers vectors as the excitations of a two-dimensional crystal at low temperatures. As the temperature is increased, the crystal softens due to the presence of an increasing number of dislocations. Once the temperature surpasses the critical melting temperature  $T_{\text{KT}}$  there is sufficient entropic driving force to produce many dislocations, which destroys the translational long-range order completely.

Since geometric dipoles are equivalent to dislocations, we expect that the binding-unbinding transition found for the geometric dipoles is essentially identical to the KTHNY transition temperature. Furthermore, we should be able to construct the theory for onset temperature in an analogous way to the KTHNY theory. This will prove useful, for instance, in understanding the onset temperature as a melting transition for inherent states in supercooled liquids, as we will discuss Section 4.1. Lastly, we have alluded that interaction energies are needed to resolve the true transition temperature for these dipoles—the next section (Section 3.2) focuses on deriving the dipole-dipole interaction energy.

### 3.2 Interaction Energy for a System of Geometric Dipoles

To understand the binding-unbinding transition in greater detail, we need to derive the pair potential  $\bar{v}^{\mu\gamma}$  between two dipoles located at  $\mathbf{x} = \mathbf{q}^\mu$  and  $\mathbf{x} = \mathbf{q}^\gamma$ , respectively. The pair potential is given in Eq. (1.42) for any excitation, and similar to the self-energy, can also be written in terms of the Airy stress functions via the strain-stress-function relation in Eq. (2.16). Thus,

$$\bar{v}^{\mu\gamma} = \frac{1}{Y^{\text{IS}}} \int d^2 \mathbf{x} \left[ (1 + \nu^{\text{IS}}) \chi_{,ij}^\mu \chi_{,ij}^\gamma - \nu^{\text{IS}} \chi_{,kk}^\mu \chi_{,ll}^\gamma \right], \quad (3.18)$$

where  $\chi^\mu$  and  $\chi^\gamma$  are the Airy stress functions in Eq. (2.77) with the excitations centered at  $\mathbf{x}' = \mathbf{q}^\mu$  and  $\mathbf{x}' = \mathbf{q}^\gamma$ , as well as dipole-moment vectors  $\mathbf{d} = \mathbf{d}^\mu$  and  $\mathbf{d} = \mathbf{d}^\gamma$ , respectively.

Similar to the steps taken in Section 2.3 to yield boundary conditions, we may apply integration by parts and divergence theorem on Eq. (3.18) to obtain the following pair potential in vector-calculus notation:

$$\bar{v}^{\mu\gamma} = \frac{1}{Y^{\text{IS}}} \int d^2 \mathbf{x} \chi^\mu \nabla^4 \chi^\gamma, \quad (3.19)$$

where use has been made of the boundary conditions established in Section 2.3 to eliminate any boundary terms in Eq. (3.19). According to Section 2.2, the biharmonic term  $\nabla^4 \chi^\gamma$  can be replaced with the localized incompatibility source  $\eta(\mathbf{x}) = -d_k^\gamma \delta(\mathbf{x} - \mathbf{q}^\gamma)_{,k}$  for a dipole. This step yields,

$$\bar{v}^{\mu\gamma} = - \int d^2 \mathbf{x} \chi^\mu d_k^\gamma \delta(\mathbf{x} - \mathbf{q}^\gamma)_{,k} = d_k^\gamma \chi_{,k}^\mu(\mathbf{x} = \mathbf{q}^\gamma), \quad (3.20)$$

where the second inequality is obtained by integration by parts and integrating over the resulting delta function. Taking the gradient of the Airy stress function for a dipole in Eq. (2.77) with respect to  $\mathbf{x}$  and evaluating it at  $\mathbf{x} = \mathbf{q}^\gamma$  gives

$$\chi_{,k}^\mu(\mathbf{x} = \mathbf{q}^\gamma) = -\frac{Y^{\text{IS}}}{4\pi} d_i^\mu \left( \delta_{ik} \left( \ln \frac{q^{\mu\gamma}}{R} + C \right) + \frac{q_i^{\mu\gamma} q_k^{\mu\gamma}}{(q^{\mu\gamma})^2} \right), \quad (3.21)$$

where  $q_i^{\mu\gamma} = q_i^\mu - q_i^\gamma$  is the pair distance vector and  $q^{\mu\gamma} = \sqrt{q_i^{\mu\gamma} q_i^{\mu\gamma}}$ . Substituting this expression in Eq. (3.20) we obtain

$$\bar{v}^{\mu\gamma} = -\frac{Y^{\text{IS}}}{4\pi} \left( d_i^\mu d_i^\gamma \left( \ln \frac{q^{\mu\gamma}}{R} + C \right) + \frac{d_i^\mu q_i^{\mu\gamma} d_j^\gamma q_j^{\mu\gamma}}{(q^{\mu\gamma})^2} \right). \quad (3.22)$$

Given  $N_{\text{exc}}$ -many dipoles and the formula for the self-energy in Eq. (3.9), the total strain energy in Eq. (1.41), which governs the statistics of the isoconfigurational ensemble, can now be written as

$$\Delta \bar{U} = -\frac{Y^{\text{IS}}}{4\pi} \sum_{\langle \mu, \gamma \rangle} \left( d_i^\mu d_i^\gamma \left( \ln \frac{q^{\mu\gamma}}{R} + C \right) + \frac{d_i^\mu q_i^{\mu\gamma} d_j^\gamma q_j^{\mu\gamma}}{(q^{\mu\gamma})^2} \right) + \frac{Y^{\text{IS}}}{8\pi} \left( \sum_{\mu=1}^{N_{\text{exc}}} d_i^\mu d_i^\mu \right) \ln \frac{R}{R_{\text{exc}}}. \quad (3.23)$$

Equation (3.23) constitutes the most general total strain energy for a system of geometric dipoles.

Equation (3.23) is further simplified via an application of the dipole moment conservation law in such a way that the system size  $R$  dependence in Eq. (3.23) is eliminated. To see this, note that the logarithmic and  $C$  constant terms in the interaction energy can be re-written as

$$\ln \frac{q^{\mu\gamma}}{R} + C = \ln \frac{q^{\mu\gamma}}{a_{\text{dpl}}} + \ln \frac{a_{\text{dpl}}}{R} + C = \ln \frac{q^{\mu\gamma}}{a_{\text{dpl}}} - \ln \frac{R}{R_{\text{exc}}} + \tilde{C} \quad (3.24)$$

where  $\tilde{C} = \frac{1}{2} \ln 2 + C$  and  $a_{\text{dpl}} = \sqrt{2} R_{\text{exc}}$  is the smallest lengthscale for two neighboring dipoles; see Fig. S.9(b). Second, the dipole-moment conservation law implies that the dipole moment of the  $\mu$ -th excitation  $d_i^\mu$  can be determined as

$$d_i^\mu = - \sum_{\gamma \neq \mu} d_i^\gamma, \quad (3.25)$$

and the sum of the square of the dipole-moment magnitude over all possible  $\mu$ -th dipoles becomes

$$\sum_{\mu=1}^{N_{\text{exc}}} d_i^\mu d_i^\mu = - \sum_{\mu=1}^{N_{\text{exc}}} \sum_{\gamma \neq \mu} d_i^\mu d_i^\gamma = -2 \sum_{\langle \mu, \gamma \rangle} d_i^\mu d_i^\gamma, \quad (3.26)$$

where use is made of the definition for pair-wise sum  $\sum_{\langle \mu, \gamma \rangle} = \frac{1}{2} \sum_{\mu=1}^{N_{\text{exc}}} \sum_{\gamma \neq \mu}$  to obtain the second equality. Using Eqs. (3.24) and (3.26), we may can combine a portion of the interaction terms in Eq. (3.23) that does not depend on the pair distance  $q^{\mu\gamma}$  into the self-energy term. This yields,

$$\Delta \bar{U} = -\frac{Y^{\text{IS}}}{4\pi} \sum_{\langle \mu, \gamma \rangle} \left( d_i^\mu d_i^\gamma \ln \frac{q^{\mu\gamma}}{a_{\text{dpl}}} + \frac{d_i^\mu q_i^{\mu\gamma} d_j^\gamma q_j^{\mu\gamma}}{(q^{\mu\gamma})^2} \right) + \frac{Y^{\text{IS}}}{8\pi} \left( \sum_{\mu=1}^{N_{\text{exc}}} d_i^\mu d_i^\mu \right) \tilde{C}$$

$$+ \frac{Y^{\text{IS}}}{8\pi} \left( \sum_{\mu=1}^{N_{\text{exc}}} d_i^\mu d_i^\mu \right) \left( \ln \frac{R}{R_{\text{exc}}} - \ln \frac{R}{R_{\text{exc}}} \right) \quad (3.27)$$

$$= - \frac{Y^{\text{IS}}}{4\pi} \sum_{\langle \mu, \gamma \rangle} \left( d_i^\mu d_i^\gamma \ln \frac{q^{\mu\gamma}}{a_{\text{dpl}}} + \frac{d_i^\mu q_i^{\mu\gamma} d_j^\gamma q_j^{\mu\gamma}}{(q^{\mu\gamma})^2} \right) + \frac{Y^{\text{IS}}}{8\pi} \left( \sum_{\mu=1}^{N_{\text{exc}}} d_i^\mu d_i^\mu \right) \tilde{C}. \quad (3.28)$$

Equation (3.28) implies that when the dipole-moment conservation law is applied to the total strain energy, the logarithmic system-size dependence vanishes and the constant  $\tilde{C}$  term plays the role of an ‘effective’ self-energy, despite having its origins from the interaction energy.

To understand the pair-wise interaction better, we can compute what the stable energy-minimizing configuration is for a system composed of two dipoles. Assuming that each dipole-moment vector has the same magnitude  $d_c$ , the reduction of Eq. (3.28) for two dipoles yields

$$\Delta \bar{U}^{12} = - \frac{Y^{\text{IS}}}{4\pi} \left( d_i^1 d_i^2 \ln \frac{q^{12}}{a_{\text{dpl}}} + \frac{d_i^1 q_i^{12} d_j^2 q_j^{12}}{(q^{12})^2} \right) + \frac{Y^{\text{IS}} d_c^2}{4\pi} \tilde{C}. \quad (3.29)$$

Upon further usage of the dipole-moment conservation law, we find that  $d_i^1 = -d_i^2$  and

$$\Delta \bar{U}^{12} = \frac{Y^{\text{IS}}}{4\pi} \left( d_c^2 \ln \frac{q^{12}}{a_{\text{dpl}}} + \frac{d_i^1 q_i^{12} d_j^1 q_j^{12}}{(q^{12})^2} \right) + \frac{Y^{\text{IS}} d_c^2}{4\pi} \tilde{C}. \quad (3.30)$$

For further simplifications, let  $q_i^{12} = q [\cos \theta, \sin \theta]$  and  $d_i^1 = d_c [\cos \psi, \sin \psi]$ . In terms of these polar-coordinate variables, Eq. (3.30) becomes

$$\Delta \bar{U}^{12} = \frac{Y^{\text{IS}} d_c^2}{4\pi} \left( \ln \frac{q}{a_{\text{dpl}}} + \cos^2(\theta - \psi) \right) + \frac{Y^{\text{IS}} d_c^2}{4\pi} \tilde{C}. \quad (3.31)$$

Taking a derivative of  $\Delta \bar{U}^{12}$  with respect to the pair distance  $q$  yields

$$\frac{\partial \Delta \bar{U}^{12}}{\partial q} = \frac{Y^{\text{IS}} d_c^2}{4\pi q} > 0 \quad \text{for } q > 0. \quad (3.32)$$

Equation (3.32) implies that two opposing dipoles can continuously decrease its total energy by moving arbitrarily close to one another. Since we have a cut-off distance  $q = a_{\text{dpl}}$ , a "minimum" is reached when the two dipoles are bound to each other. Next, we take the derivative of Eq. (3.31) with respect to  $\theta$ :

$$\frac{\partial \Delta \bar{U}^{12}}{\partial \theta} = \frac{Y^{\text{IS}} d_c^2}{4\pi} (-2 \cos(\theta - \psi) \sin(\theta - \psi)) = -\frac{Y^{\text{IS}} d_c^2}{2\pi} \sin(2\theta - 2\psi) = 0. \quad (3.33)$$

The energy is extremized when  $\theta = \psi - \frac{n\pi}{2}$  where  $n$  is any integer. In other words, there are two possibilities: the pair distance vector  $\mathbf{q}^{\mu\gamma}$  and dipole moment vector  $\mathbf{d}^\mu$  are perpendicular ( $n$  odd) or parallel ( $n$  even) to each other. Using the second-order derivative test, we find that

$$\frac{\partial^2 \Delta \bar{U}^{12}}{\partial \theta^2} = -\frac{Y^{\text{IS}} d_c^2}{\pi} \cos(2\theta - 2\psi) \begin{cases} > 0 & \text{if } \mathbf{q}^{\mu\gamma} \perp \mathbf{d}^\mu \\ < 0 & \text{if } \mathbf{q}^{\mu\gamma} \parallel \mathbf{d}^\mu \end{cases}. \quad (3.34)$$

From Eq. (3.34), we see that a stable minimum is reached when the dipole-moment vector  $\mathbf{d}^\mu$  perpendicular to the pair-distance vector  $\mathbf{q}^{\mu\gamma}$ .

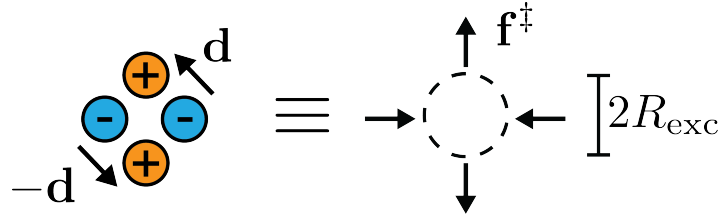

Figure S.11: Equivalence between a quadrupole (left) that controls the low-temperature excitations of the many-dipole system and a pure-shear excitation (right) that was originally proposed in Ref. [7] as the emergent excitations of a supercooled liquid.

Combining this result with Eq. (3.32), we conclude that the most stable energy-minimizing configuration is a bound-dipole pair with  $\mathbf{q}^{\mu\gamma}$  and  $\mathbf{d}^\mu$  perpendicular to each other; a configuration that was already considered in Section 3.1 (see Fig. S.9(b)). The perpendicular condition ( $\mathbf{q}^{\mu\gamma} \perp \mathbf{d}^\mu$ ) is important as it affects the form of the quadrupole tensor  $\mathbf{Q}$ . Using the general quadrupole tensor formula for a bound-dipole pair (Eq. (2.49)), we find that

$$\mathbf{Q} = \frac{d_c a_{\text{dpl}}}{2} \begin{bmatrix} \cos 2\psi & \sin 2\psi \\ \sin 2\psi & -\cos 2\psi \end{bmatrix}, \quad (3.35)$$

where  $a_{\text{dpl}} = |\mathbf{a}^{\text{dpl}}|$  and  $\psi$  is the orientation angle as defined in Fig. S.9. Note that Eq. (3.35) is equivalent to Eq. (3.12) since  $d_c = m a_{\text{dpl}}$  and  $a_{\text{dpl}} = 2R_{\text{dpl}} = \sqrt{2}R_{\text{exc}}$  according to Fig. S.9. Since  $\mathbf{Q}$  is traceless, this implies that the corresponding eigenstrain is traceless (see Section 2.2) and a bound-dipole pair is equivalent to a localized pure-shear excitation; see Fig. S.11. Pure-shear excitations were originally studied in previous work [7], and are proposed to be crucial in establishing the origin of excitations that drive dynamics in the supercooled liquid according to dynamical facilitation (DF) theory [2]. Thus, a theory for onset temperature based on geometric dipoles will simultaneously explain the emergence of localized pure-shear excitations, which fits with the original concept of an onset temperature within the context of DF theory.

We can take advantage of this connection between bound-dipole pairs and pure-shear excitations to construct a mapping between the parameters defining individual dipoles, such as the dipole-moment magnitude  $d_c$  and the undetermined constant  $\tilde{C}$ , to the ones defining the pure-shear excitations, such as the elastic moduli, the eigenstrain constant  $\epsilon_c$  and excitation size  $R_{\text{exc}}$ . Such a mapping, which yields a form of self-consistency between bound-dipole pairs and localized pure-shear excitations, is outlined in the next section.

### 3.3 Mapping Bound-Dipole Pairs to Pure-Shear Excitations

In this section, we map the parameters defining geometric dipoles, i.e., the dipole-moment magnitude  $d_c$  and constant  $\tilde{C}$ , to those defining a localized pure-shear excitation proposed in Ref. [7]. First, the dipole-moment magnitude  $d_c$  is mapped to the eigenstrain constant  $\epsilon_c$ , excitation size  $R_{\text{exc}}$ , and the elastic moduli by matching the stress field of the bound-dipole to that of the pure-shear excitation. Recall from Ref. [7] that a pure-shear excitation located at the origin is characterized by angular-dependent stress fields that scale as  $\sim 1/r^2$  for large distances. Let the principal components of the stress tensor be defined as

$$T_1 = -\frac{1}{2}(T_{xx} + T_{yy}), \quad T_2 = \frac{1}{2}(T_{yy} - T_{xx}), \quad T_3 = T_{xy}. \quad (3.36)$$

Using the force-dipole formalism [32], the stress fields for a pure-shear excitation can be written for  $r > 0$  as

$$T_1^\ddagger(r, \theta) = f^\ddagger R_{\text{exc}} \frac{\nu^{\text{IS}} + 1}{\pi r^2} \cos(2\theta - 2\psi), \quad (3.37)$$

$$T_2^\ddagger(r, \theta) = f^\ddagger R_{\text{exc}} \frac{\nu^{\text{IS}} + 1}{\pi r^2} \cos(4\theta - 2\psi), \quad (3.38)$$

$$T_3^\ddagger(r, \theta) = -f^\ddagger R_{\text{exc}} \frac{\nu^{\text{IS}} + 1}{\pi r^2} \sin(4\theta - 2\psi), \quad (3.39)$$

where  $f^\ddagger$  is the magnitude of the force needed to push one of the particles participating at the core of the pure-shear excitation, and it has a formula as follows [7]

$$f^\ddagger = \frac{\sqrt{2}\pi R_{\text{exc}} G^{\text{IS}} \epsilon_c}{(1 + \nu^{\text{IS}})}. \quad (3.40)$$

Note that the super-script  $\ddagger$  denotes the transition-state nature of the excitation. These stress fields can be compared to those obtained for a bound-dipole pair. Using the stress function solution for a general traceless quadrupole tensor (Eq. (2.79)), the quadrupole tensor in Eq. (3.35), and the relation between stress-function and stresses (Eq. (2.11)), we can derive the principal stresses associated with a bound-dipole pair. The result is

$$T_1^\ddagger(r, \theta) = Y^{\text{IS}} d_c a_{\text{dpl}} \frac{\cos(2\theta - 2\psi)}{4\pi r^2}, \quad (3.41)$$

$$T_2^\ddagger(r, \theta) = Y^{\text{IS}} d_c a_{\text{dpl}} \frac{\cos(4\theta - 2\psi)}{4\pi r^2}, \quad (3.42)$$

$$T_3^\ddagger(r, \theta) = -Y^{\text{IS}} d_c a_{\text{dpl}} \frac{\sin(4\theta - 2\psi)}{4\pi r^2}. \quad (3.43)$$

The solutions in Eqs. (3.41)–(3.43) are identical to Eqs. (3.37)–(3.39) if the following equation is true:

$$f^\ddagger (\nu^{\text{IS}} + 1) R_{\text{exc}} = \frac{1}{4} Y^{\text{IS}} d_c a_{\text{dpl}}. \quad (3.44)$$

Using Eq. (3.40) and the fact that  $Y^{\text{IS}} = 2G^{\text{IS}} (\nu^{\text{IS}} + 1)$ , we can reduce Eq. (3.44) into

$$\sqrt{2}\pi R_{\text{exc}}^2 \epsilon_c = \frac{1}{2} (\nu^{\text{IS}} + 1) d_c a_{\text{dpl}}. \quad (3.45)$$

Since  $a_{\text{dpl}} = \sqrt{2}R_{\text{exc}}$  (from Fig. S.9), we can turn Eq. (3.45) into a formula for the dipole-moment magnitude,

$$d_c = \frac{2\pi R_{\text{exc}} \epsilon_c}{\nu^{\text{IS}} + 1}, \quad (3.46)$$

where the size of excitation  $R_{\text{exc}}$  and eigenstrain  $\epsilon_c$  are worked in the theory of localized excitations in Ref. [7], with formulas given by

$$R_{\text{exc}} = \frac{\sqrt{3}\sigma_d}{2(1 + 2u^\ddagger/\sigma_d)}, \quad \epsilon_c = 2\sqrt{2} \left[ \frac{u^\ddagger/\sigma_d (1 + u^\ddagger/\sigma_d)}{1 + 2u^\ddagger/\sigma_d} \right], \quad (3.47)$$

where  $\sigma_d$  is the particle diameter, and  $u^\ddagger$  is the displacement magnitude needed to initiate the bond-breaking event, computable from the inherent-state radial distribution function [7]. Note that the

mapping for dipole magnitude also extends to the monopole charge since  $d_c = ma_{\text{dpl}}$ . In particular, we find that

$$m = \frac{\sqrt{2}\pi\epsilon_c}{\nu^{\text{IS}} + 1}. \quad (3.48)$$

Next, we determine  $\tilde{C}$  by first inspecting the total strain energy for two dipoles in Eq. (3.30). In particular, we evaluate Eq. (3.30) at its minimum, i.e., for a bound-dipole pair where  $q = a_{\text{dpl}}$  and  $d_i^\mu q_i^{\mu\gamma} = 0$ , which yields

$$\Delta\bar{U}_{\min}^{12} = \frac{Y^{\text{IS}}d_c^2}{4\pi}\tilde{C}. \quad (3.49)$$

Equation (3.49) says that the stored elastic energy of a bound-dipole pair is self-contained in the magnitude of the interaction energy at the smallest lengthscales, since the constant  $\tilde{C}$  has its origins in the interaction energy (see Section 2). Since a bound-dipole pair must be energetically equivalent to a quadrupole, the constant  $\tilde{C}$  must be matched to the self-energy  $\bar{E}_c$  for a quadrupole, as given by Eq. (3.13). Equating Eq. (3.13) with Eq. (3.49) yields

$$\frac{Y^{\text{IS}}d_c^2}{4\pi}\tilde{C} = \frac{d_c^2Y^{\text{IS}}(3 + \nu^{\text{IS}})}{16\pi}. \quad (3.50)$$

Using Eq. (3.50), we find that

$$\tilde{C} = \frac{3 + \nu^{\text{IS}}}{4}. \quad (3.51)$$

For  $\nu^{\text{IS}} \in [0, 1]$  we find that  $\tilde{C} \in [0.75, 1]$ .

Note that in the incompressible limit ( $\nu^{\text{IS}} \rightarrow 1$ ), the bound-dipole pair energy becomes

$$\Delta\bar{U}_{\min}^{12} = \frac{Y^{\text{IS}}d_c^2}{4\pi} = 2G^{\text{IS}}(1 + 1)\frac{4\pi^2R_{\text{exc}}^2\epsilon_c^2}{4\pi(1 + 1)^2} = G^{\text{IS}}\pi R_{\text{exc}}^2\epsilon_c^2, \quad (3.52)$$

where the rightmost part is equal to the energy barrier  $\Delta F^\ddagger$  for the rate of excitation events according to the theory of localized excitations in Ref. [7],

$$\Delta F^\ddagger = 6\pi G^{\text{IS}}\sigma_d^2 \frac{(\tilde{u}^\ddagger)^2(1 + \tilde{u}^\ddagger)^2}{(1 + 2\tilde{u}^\ddagger)^4}, \quad (3.53)$$

where  $\tilde{u}^\ddagger = u^\ddagger/\sigma_d$ . Despite this self-consistency at the level of energy barriers, we emphasize that this closure relation is not unique. One may analyze the total energy of two bound-dipole pairs and match it to the total energy of two quadrupoles. This may yield a slightly different estimate for  $\tilde{C}$  that is dependent on the quadrupole-quadrupole interaction. Thus, by matching  $\tilde{C}$  at the level of a single quadrupole, we make the implicit assumption that quadrupole interactions are negligible at low temperatures.

### 3.4 Grand Canonical Partition Function for Geometric Dipoles

Given the mapping of the geometric-dipole parameters Eqs. (3.46) and (3.50), we are ready to state the final grand canonical partition function  $\Xi_{\text{exc}}$  for geometric dipoles. This partition function is expressed in terms of dimensionless quantities, and we follow closely the convention of Halperin and Nelson [8] to define these quantities. To this end, let the dimensionless stiffness and compliance tensor be written as

$$\tilde{C}_{ijkl} = \beta d_c^2 C_{ijkl} \quad \text{and} \quad \tilde{S}_{ijkl} = \frac{k_B T}{d_c^2} S_{ijkl}, \quad (3.54)$$

respectively. If we use the total strain energy given in Eq. (3.28), then we need to use the term containing the  $\tilde{C}$  constant to act as an ‘effective’ self-energy. Following Ref. [8], we define the dimensionless self-energy for these dipoles as

$$\tilde{E}_c = \frac{\tilde{Y}^{\text{IS}}}{8\pi}(\tilde{C} + 1) = \frac{1}{4}(7 + \nu^{\text{IS}})\Delta F^\ddagger, \quad (3.55)$$

where  $\tilde{Y}^{\text{IS}} = \beta d_c^2 Y^{\text{IS}}$  is the dimensionless inherent-state Young’s modulus.

Continuing, let the dimensionless strain energy and dipole-moment vector be  $\Delta\tilde{U} = \beta\Delta\bar{U}$  and  $\tilde{d}_i^\mu = d_i^\mu/d_c$ , respectively. The strain energy (Eq. (3.28)) in dimensionless form is then

$$\Delta\tilde{U} = -\frac{\tilde{Y}^{\text{IS}}}{4\pi} \sum_{\langle\mu,\gamma\rangle} \left( \tilde{d}_i^\mu \tilde{d}_i^\gamma \ln \frac{q^{\mu\gamma}}{a_{\text{dpl}}} + \frac{\tilde{d}_i^\mu q_i^{\mu\gamma} \tilde{d}_j^\gamma q_j^{\mu\gamma}}{(q^{\mu\gamma})^2} \right) + \frac{\tilde{Y}^{\text{IS}}}{8\pi} \left( \sum_{\mu=1}^{N_{\text{exc}}} \tilde{d}_i^\mu \tilde{d}_i^\mu \right) \tilde{C}. \quad (3.56)$$

By re-writing  $\tilde{C} = \tilde{C} + 1 - 1$ , we can introduce the dimensionless self-energy into Eq. (3.56),

$$\Delta\tilde{U} = -\frac{\tilde{Y}^{\text{IS}}}{4\pi} \sum_{\langle\mu,\gamma\rangle} \left( \tilde{d}_i^\mu \tilde{d}_i^\gamma \ln \frac{q^{\mu\gamma}}{a_{\text{dpl}}} + \frac{\tilde{d}_i^\mu q_i^{\mu\gamma} \tilde{d}_j^\gamma q_j^{\mu\gamma}}{(q^{\mu\gamma})^2} \right) + \tilde{E}_c \left( \sum_{\mu=1}^{N_{\text{exc}}} \tilde{d}_i^\mu \tilde{d}_i^\mu \right) - \frac{\tilde{Y}^{\text{IS}}}{8\pi} \left( \sum_{\mu=1}^{N_{\text{exc}}} \tilde{d}_i^\mu \tilde{d}_i^\mu \right). \quad (3.57)$$

The last term in Eq. (3.57) can be combined into the interaction term using the relation in Eq. (3.26). This step yields

$$\Delta\tilde{U} = -\frac{\tilde{Y}^{\text{IS}}}{4\pi} \sum_{\langle\mu,\gamma\rangle} \left( \tilde{d}_i^\mu \tilde{d}_i^\gamma \left( \ln \frac{q^{\mu\gamma}}{a_{\text{dpl}}} - 1 \right) + \frac{\tilde{d}_i^\mu q_i^{\mu\gamma} \tilde{d}_j^\gamma q_j^{\mu\gamma}}{(q^{\mu\gamma})^2} \right) + \tilde{E}_c N_{\text{exc}}, \quad (3.58)$$

where use is made of the fact that  $\tilde{d}_i^\mu \tilde{d}_i^\mu = 1$  to obtain the last term.

Now, let the effective fugacity be defined as

$$\tilde{y} = e^{-\tilde{E}_c}. \quad (3.59)$$

The final grand canonical partition function  $\tilde{\Xi}_{\text{exc}}$  in Eq. (1.51) can be re-written as

$$\tilde{\Xi}_{\text{exc}} = \sum_{N_{\text{exc}}=0}^{N_d} Z_{N_{\text{exc}}} \tilde{y}^{N_{\text{exc}}}, \quad Z_{N_{\text{exc}}} = \frac{1}{(a_{\text{dpl}})^{N_{\text{exc}}d} N_{\text{exc}}!} \int \prod_{\mu=1}^{N_{\text{exc}}} d^2\mathbf{q}^\mu d\psi^\mu C(\{\psi^\mu\}) e^{-\tilde{\mathcal{H}}}, \quad (3.60)$$

$$\tilde{\mathcal{H}}(\{\mathbf{q}^\mu, \psi^\mu\}) = \sum_{\langle\mu,\gamma\rangle} \tilde{v}^{\mu\gamma}, \quad \tilde{v}^{\mu\gamma} = -\frac{\tilde{Y}^{\text{IS}}}{4\pi} \left( \tilde{d}_i^\mu \tilde{d}_i^\gamma \left( \ln \frac{q^{\mu\gamma}}{a_{\text{dpl}}} - 1 \right) + \frac{\tilde{d}_i^\mu q_i^{\mu\gamma} \tilde{d}_j^\gamma q_j^{\mu\gamma}}{(q^{\mu\gamma})^2} \right), \quad (3.61)$$

and  $C(\{\psi^\mu\})$  is a constraint function that enforces the dipole-moment conservation law. The grand partition function in Eq. (3.60) sets up the more detailed analysis of the binding-unbinding transition, beginning in Section 4. In particular, the analysis follows closely the one adopted in the KTHNY theory, where the use of renormalization group (RG) [35, 36] is crucial in obtaining an accurate prediction of the transition temperature.

## 4 Elastic Constants and Fluctuation Formulas

We begin our investigation of the binding-unbinding transition by emphasizing its dual picture as an excitation-mediated melting of inherent states in Section 4.1. This perspective adds new insight to the significance of the onset temperature, and justifies why investigating the renormalization of elastic moduli, whose fluctuation formula is also derived in this section, is crucial for determining the location of the binding-unbinding transition. Finally, we specialize these formulas to a case where only a pair of dipoles is present in Section 4.2.

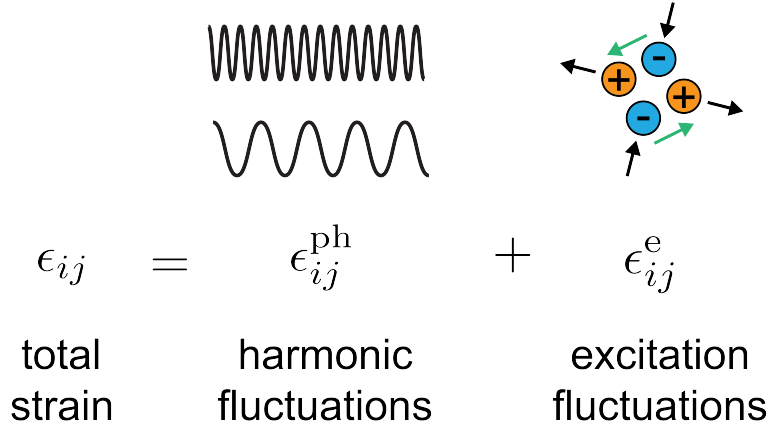

Figure S.12: A general illustration of what fluctuations are considered in the total strain tensor. The goal of subsequent analysis is to determine how the 'bare' elastic moduli, which controls the harmonic fluctuations, is renormalized under the influence of the excitation fluctuations

#### 4.1 The Binding-Unbinding Transition as an Inherent-State Melting Transition

Recall from Section 3 that the physics for the binding-unbinding transition of the geometric dipoles is similar to the one described by the KTHNY theory [5, 8–11]. In the KTHNY theory one begins with the two-dimensional crystal as a reference configuration and endow this crystal with two kinds of fluctuations: the harmonic lattice vibrations and the spontaneous production of dislocation pairs. The theory then predicts how the elastic moduli change as a function of temperature due to the presence of these fluctuations. At a critical temperature  $T_{\text{KT}}$ , the elastic moduli vanish indicating the dislocation-mediated melting of the crystalline solid, as well as the unbinding of dislocation pairs to free dislocations. The temperature  $T_{\text{KT}}$  is then determined by computing elastic moduli through a set of fluctuation formulas, which relate these moduli to fluctuations in the strain.

A similar situation exists for a supercooled liquid. At timescales  $t \sim \langle \tau_{\text{jump}} \rangle \ll \tau_{\text{eq}}$  (see Eq. (1.2)) a supercooled liquid can be thought of as an isotropic solid that also experiences two kinds of fluctuations. The first kind is the harmonic or phononic strain fluctuations  $\epsilon_{ij}^{\text{ph}}$ , whose statistics was established in previous work [7] to be governed by the following partition function:

$$\bar{Q}_{\text{ph}} = \int \mathcal{D}\mathbf{u}^{\text{ph}} e^{-\beta \Delta F}, \quad \Delta F[\epsilon_{ij}^{\text{ph}}] = \frac{1}{2} \int d^d \mathbf{x} \epsilon_{ij}^{\text{ph}} C_{ijkl}^{\text{IS}} \epsilon_{kl}^{\text{ph}}, \quad (4.1)$$

and  $\epsilon_{ij}^{\text{ph}} = \frac{1}{2} (u_{i,j}^{\text{ph}} + u_{j,i}^{\text{ph}})$ . The second kind of fluctuations are the ones induced by the inherent-state jumps, which we model through the elastic strain of localized excitations  $\epsilon_{ij}^{\text{e}}$ . From Section 1.2 and Section 3 we know that the partition function describing these jumps is the grand canonical partition function  $\bar{\Xi}_{\text{exc}}$  in Eq. (3.60). As illustrated in Fig. S.12, the total strain fluctuations observed in a supercooled liquid is the sum of harmonic and excitation fluctuations,

$$\epsilon_{ij} = \epsilon_{ij}^{\text{ph}} + \epsilon_{ij}^{\text{e}}, \quad (4.2)$$

and its statistics is governed by a partition function composed of the following product of partition functions:

$$\bar{\mathcal{Z}} = \bar{Q}_{\text{ph}} \bar{\Xi}_{\text{exc}}. \quad (4.3)$$

In writing Eq. (4.3) the harmonic and excitation fluctuations become statistically independent, i.e.,  $\langle \epsilon_{ij}^{\text{ph}} \epsilon_{ij}^{\text{e}} \rangle = \langle \epsilon_{ij}^{\text{ph}} \rangle \langle \epsilon_{ij}^{\text{e}} \rangle$ . The corresponding free-energy can then be written as

$$\bar{\Gamma}(T) = -k_{\text{B}} T \ln \bar{Q}_{\text{ph}} - k_{\text{B}} T \ln \bar{\Xi}_{\text{exc}}. \quad (4.4)$$

As we shear the supercooled liquid at the intermediate timescales, its macroscopic elastic behavior is affected by both the harmonic and excitation fluctuations. A static linear response theory can then be used to understand the role of these fluctuations as it yields a formula relating the compliance tensor with the total strain fluctuation  $\epsilon_{ij}$ . These fluctuation formulas are then used to determine the location of the melting point  $T_{KT}$ . In the linear response framework, we perturb the system via an application of a uniform external stress  $T_{ij}$ , which induces fluctuations in the area-averaged strain tensor

$$\hat{\epsilon}_{ij} = \frac{1}{A_0} \int d^2\mathbf{x} \epsilon_{ij}(\mathbf{x}), \quad (4.5)$$

where  $A_0$  is the total area of the reference configuration. The perturbation in the Hamiltonian can be written as

$$\Delta\mathcal{H} = -A_0 T_{ij} \hat{\epsilon}_{ij}. \quad (4.6)$$

The change in free energy  $\Delta\bar{\Gamma}(T_{ij}, T) = \bar{\Gamma}(T_{ij}, T) - \bar{\Gamma}(T)$  due to this perturbation can be computed via free-energy perturbation (FEP) [37]

$$\bar{\Gamma}(T_{ij}, T) - \bar{\Gamma}(T) = -k_B T \ln \left\langle e^{-\beta \Delta\mathcal{H}} \right\rangle = -k_B T \ln \left\langle e^{\beta A_0 T_{ij} \hat{\epsilon}_{ij}} \right\rangle, \quad (4.7)$$

where  $\langle \dots \rangle$  is to denote ensemble average at zero external stress. Taylor expanding the rightmost part of Eq. (4.7) around  $T_{ij} = 0$  yields

$$\bar{\Gamma}(T_{ij}, T) - \bar{\Gamma}(0, T) \approx -A_0 \delta T_{ij} \langle \hat{\epsilon}_{ij} \rangle - \frac{\beta A_0^2}{2} \delta T_{ij} \langle \hat{\epsilon}_{ij} \hat{\epsilon}_{kl} \rangle \delta T_{kl} \quad (4.8)$$

$$= -\frac{\beta A_0^2}{2} \delta T_{ij} \langle \hat{\epsilon}_{ij} \hat{\epsilon}_{kl} \rangle \delta T_{kl}, \quad (4.9)$$

where use is made of the fact  $\langle \hat{\epsilon}_{ij} \rangle = 0$  under the presence of zero external stress. From classical thermodynamics, the free-energy  $\bar{\Gamma}(T_{ij}, T)$  can also be viewed as a generalized Gibbs free energy, whose fundamental thermodynamic relation is

$$d\bar{\Gamma}(T_{ij}, T) = -S dT - A_0 \langle \hat{\epsilon}_{ij} \rangle_f dT_{ij}, \quad (4.10)$$

where angular brackets  $\langle \dots \rangle_f$  denote ensemble averages at non-zero stress. According to the fundamental thermodynamic relation, the components of the macroscopic strain is related to the free-energy derivatives as

$$\langle \hat{\epsilon}_{ij} \rangle := \lim_{T_{ij} \rightarrow 0} \langle \hat{\epsilon}_{ij} \rangle_f = -\frac{1}{A_0} \left. \frac{\partial \bar{\Gamma}(0, T)}{\partial T_{ij}} \right|_T, \quad (4.11)$$

which is zero if  $T_{ij} = 0$ . By definition, the compliance tensor  $S_{ijkl}^R$  is

$$S_{ijkl}^R := \lim_{T_{ij} \rightarrow 0} \left. \frac{\partial \langle \hat{\epsilon}_{ij} \rangle_f}{\partial T_{kl}} \right|_T = -\frac{1}{A_0} \left. \frac{\partial^2 \bar{\Gamma}(0, T)}{\partial T_{ij} \partial T_{kl}} \right|_T, \quad (4.12)$$

where use is made of Eq. (4.11) to obtain the second equality. Note that the superscript ‘R’ distinguishes  $S_{ijkl}^R$  from its inherent-state counterpart  $S_{ijkl}^{IS}$ , since  $S_{ijkl}^R$  will include fluctuation corrections that renormalize the ‘bare’ value from  $S_{ijkl}^{IS}$ . Comparing this definition with the second-order term of the series expansion in Eq. (4.9), we find that

$$S_{ijkl}^R = \beta A_0 \langle \hat{\epsilon}_{ij} \hat{\epsilon}_{kl} \rangle. \quad (4.13)$$

Substituting the strain decomposition in Eq. (4.2) gives

$$S_{ijkl}^R = \beta A_0 \langle \hat{\epsilon}_{ij}^{\text{ph}} \hat{\epsilon}_{kl}^{\text{ph}} \rangle + \beta A_0 \langle \hat{\epsilon}_{ij}^{\text{e}} \hat{\epsilon}_{kl}^{\text{ph}} + \hat{\epsilon}_{ij}^{\text{ph}} \hat{\epsilon}_{kl}^{\text{e}} \rangle + \beta A_0 \langle \hat{\epsilon}_{ij}^{\text{e}} \hat{\epsilon}_{kl}^{\text{e}} \rangle \quad (4.14)$$

$$= \beta A_0 \langle \hat{\epsilon}_{ij}^{\text{ph}} \hat{\epsilon}_{kl}^{\text{ph}} \rangle + \beta A_0 \langle \hat{\epsilon}_{ij}^{\text{e}} \hat{\epsilon}_{kl}^{\text{e}} \rangle, \quad (4.15)$$

where we used the fact that  $\langle \epsilon_{ij}^{\text{ph}} \epsilon_{ij}^{\text{e}} \rangle = \langle \epsilon_{ij}^{\text{ph}} \rangle \langle \epsilon_{ij}^{\text{e}} \rangle$  and  $\langle \epsilon_{ij}^{\text{ph}} \rangle = \langle \epsilon_{ij}^{\text{e}} \rangle = 0$  to yield the second equality. From the partition function in Eq. (4.1), we see that  $\hat{\epsilon}_{kl}^{\text{ph}}$  has Gaussian statistics, whose inverse covariance function is given by  $C_{ijkl}^{\text{IS}}$ . This implies that the renormalized compliance is

$$S_{ijkl}^R = S_{ijkl}^{\text{IS}} + \beta A_0 \langle \hat{\epsilon}_{ij}^{\text{e}} \hat{\epsilon}_{kl}^{\text{e}} \rangle. \quad (4.16)$$

In terms of the non-dimensionalization of Section 3.4, the fluctuation formula can be written as

$$\tilde{S}_{ijkl}^R = \tilde{S}_{ijkl}^{\text{IS}} + \frac{A_0}{d_c^2} \langle \hat{\epsilon}_{ij}^{\text{e}} \hat{\epsilon}_{kl}^{\text{e}} \rangle. \quad (4.17)$$

In an isotropic system, only two components of the stiffness tensor are needed. For instance, the bulk modulus is

$$\frac{1}{\tilde{B}^R} := \tilde{S}_{iikk}^R = \frac{1}{\tilde{B}^{\text{IS}}} + \frac{A_0}{d_c^2} \langle \hat{\epsilon}_{ii}^{\text{e}} \hat{\epsilon}_{kk}^{\text{e}} \rangle \quad (4.18)$$

and the shear modulus can be obtained by noting that  $S_{ijij}^R = \frac{1}{G^R} + \frac{1}{2B^R}$ . This yields

$$\frac{1}{\tilde{G}^R} = \frac{1}{\tilde{G}^{\text{IS}}} + \frac{A_0}{d_c^2} \left( \langle \hat{\epsilon}_{ij}^{\text{e}} \hat{\epsilon}_{ij}^{\text{e}} \rangle - \frac{1}{2} \langle \hat{\epsilon}_{ii}^{\text{e}} \hat{\epsilon}_{kk}^{\text{e}} \rangle \right). \quad (4.19)$$

It will also be useful to have the fluctuation formula for the Young's modulus,

$$\frac{1}{\tilde{Y}^R} = \frac{1}{4} \left( \frac{1}{\tilde{G}^R} + \frac{1}{\tilde{B}^R} \right) = \frac{1}{\tilde{Y}^{\text{IS}}} + \frac{A_0}{4d_c^2} \left( \langle \hat{\epsilon}_{ij}^{\text{e}} \hat{\epsilon}_{ij}^{\text{e}} \rangle + \frac{1}{2} \langle \hat{\epsilon}_{ii}^{\text{e}} \hat{\epsilon}_{kk}^{\text{e}} \rangle \right), \quad (4.20)$$

since the Young's modulus is the elastic modulus that directly enters into the interaction energy of the excitations.

Equations (4.18) to (4.20) can be interpreted in the language of renormalization. To see this, consider a shearing experiment performed on a supercooled liquid at timescales  $t \sim \langle \tau_{\text{jump}}(T) \rangle \ll \tau_{\text{eq}}$ ; see Eq. (1.2). The macroscopic elastic response is dictated by the shear modulus in Eq. (4.19), which is an aggregate of the 'bare' shear modulus, as given by  $G^{\text{IS}}$ , and a fluctuation correction due to the excitations. Depending on the operating temperature  $T$ , these fluctuation corrections may dominate the linear response since excitations (on average) increasingly soften the initial inherent state at higher temperatures in the same way that dislocations do for a 2D crystal in the KTHNY theory. Once the critical temperature is reached, the softening reaches a point where  $G^R = 0$  at these intermediate timescales, and thus any initial inherent state 'melts' and mechanically responds like a fluid. In light of this scenario, we may interpret the onset temperature as an inherent-state melting transition.

Guided by the KTHNY theory, our task now is to predict when this vanishing of the shear modulus (or the stiffness tensor  $C_{ijkl}^R$  in general) occurs, and this can be achieved via the renormalization group (RG) method [35, 36]. Before we embark on applying the RG method, which is described in Section 5, we need a formula for  $\hat{\epsilon}_{ij}^{\text{e}}$  as a function of excitation coordinates  $\{\mathbf{q}^\mu\}$  and orientation angles  $\{\psi^\mu\}$ , since the ensemble average in Eqs. (4.18)–(4.20) involves a grand-canonical ensemble average over a variable number of excitations and configurations. The derivation for such a formula is provided in the next section, Section 4.2.

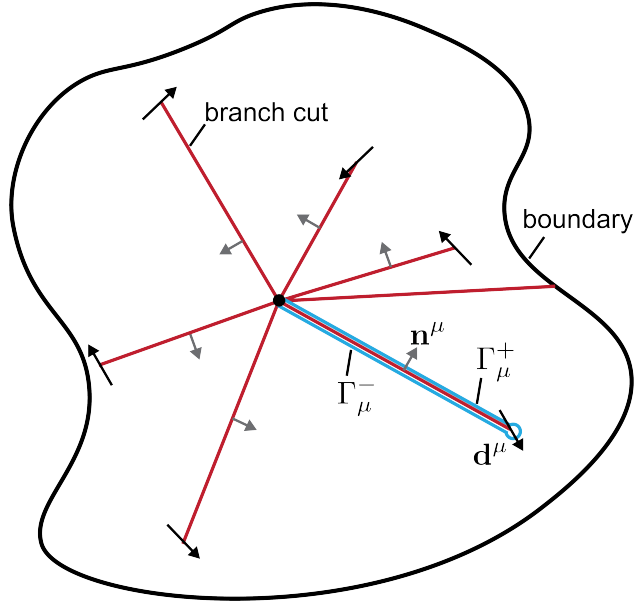

Figure S.13: Schematic of the line discontinuities, i.e., branch cuts, of the displacement field in a system consisting of many dipoles. All line discontinuities terminate at the center of mass of the dipoles. Every branch cut is associated with an enclosing curve that has two sides,  $\Gamma_\mu^+$  and  $\Gamma_\mu^-$ . These two sides pick up the displacement jump across the branch cut upon the usage of Green's theorem.

## 4.2 Strain Formula for a System of Dipoles

In this section, we derive a formula for the area-averaged strain that arises from  $N_{\text{exc}}$ -many dipoles. We begin from its definition that consists of a sum over individual strains

$$\hat{\epsilon}_{ij}^e := \frac{1}{A_0} \sum_{\mu=1}^{N_{\text{exc}}} \int d^2\mathbf{x} \, \epsilon_{ij}^\mu, \quad (4.21)$$

where  $\epsilon_{ij}^\mu$  is the elastic strain of a dipolar excitation with dipole moment  $\mathbf{d}^\mu$  at position  $\mathbf{q}^\mu$ . From Section 2.2, we know that each dipole exhibits a straight line discontinuity in its displacement field  $u_i^\mu$ , and this needs to be accounted for in the computation of Eq. (4.21). To resolve the discontinuity problem, suppose that  $\epsilon_{ij}^\mu$  in Eq. (4.21) is written in terms of the gradient of  $u_i^\mu$ , which leads to

$$\hat{\epsilon}_{ij}^e = \frac{1}{2A_0} \sum_{\mu=1}^{N_{\text{exc}}} \int d^2\mathbf{x} \, (u_{i,j}^\mu + u_{j,i}^\mu). \quad (4.22)$$

In this form, we may account for the discontinuity in  $u_i^\mu$  via Green's theorem, where we replace the area integral in Eq. (4.22) with line integrals, and each integral is taken over a curve that encloses a line discontinuity [8].

To write Eq. (4.22) in terms of such line integrals, consider a configuration of many dipoles in Fig. S.13. Each line discontinuity from the dipole is oriented in an arbitrary angle with respect to the dipole-moment vector  $\mathbf{d}^\mu$ <sup>‡</sup>. Each line discontinuity is also referred to as a branch cut of the

<sup>‡</sup>In general, the orientation of the line discontinuity with respect to  $\mathbf{d}^\mu$  dictates the mode of induced elastic deformation. See Section 2.2 where we demonstrate how a geometric dipole with  $\mathbf{d}^\mu$  that is parallel and perpendicular to the line discontinuity corresponds to a Mode I and Mode II dislocation, respectively.

displacement field  $u_i^\mu$ <sup>§</sup>, and it terminates at the center of mass of the many-dipole system. Now, let  $\Gamma_\mu^+$  and  $\Gamma_\mu^-$  be the straight line curve that extends along the branch cut with a corresponding normal vector given by  $n_j^\mu$  and  $-n_j^\mu$ , respectively; see Fig. S.13 for its orientation relative to its respective branch. For every branch cut, the enclosing curve for the line integral is a piecewise curve made up of  $\Gamma_\mu^+$ ,  $\Gamma_\mu^-$ , and a circle with vanishing radius that wraps around the  $\mu$ -th dipole. Given these piecewise curves, we can write the result of applying Green's theorem to Eq. (4.22) as

$$\hat{\epsilon}_{ij}^e = -\frac{1}{2A_0} \sum_{\mu=1}^{N_{\text{exc}}} \left[ \int_{\Gamma_\mu^+} d\mathcal{C} \left( u_i^{\mu,+} n_j^\mu + u_j^{\mu,+} n_i^\mu \right) - \int_{\Gamma_\mu^-} d\mathcal{C} \left( u_i^{\mu,-} n_j^\mu + u_j^{\mu,-} n_i^\mu \right) \right], \quad (4.23)$$

where  $u_i^{\mu,+}$  and  $u_i^{\mu,-}$  is the elastic displacement due to the  $\mu$ -th dipole at  $\Gamma_\mu^+$  and  $\Gamma_\mu^-$ , respectively, and the boundary terms are set to zero. Note the minus sign in front of Eq. (4.23), which arises from the fact that the closed line integrals are defined in the interior of the body, not on its boundary.

From Section 2.2, we also know that the displacement jump  $[[u_i^\mu]] := u_i^{\mu,+} - u_i^{\mu,-}$  across the cut is constant, which results in the elastic strain emanating from a geometric dipole to be identical to that of a dislocation with Burgers vector  $b_i^\mu = \varepsilon_{ij} d_j^\mu$  (Eq. (2.42)). This mapping between dislocations and geometric dipoles is useful since the displacement jump  $[[u_i^\mu]] = b_i^\mu$ , by definition of the Burgers vector. Given that the normal vector of each cut is also constant, this leads to

$$\hat{\epsilon}_{ij}^e = -\frac{1}{2A_0} \sum_{\mu=1}^{N_{\text{exc}}} \left[ b_i^\mu n_j^\mu + b_j^\mu n_i^\mu \right] \left( \int_{\Gamma_\mu^+} d\mathcal{C} \right), \quad (4.24)$$

where use is made of the fact that  $\int_{\Gamma_\mu^+} d\mathcal{C} = \int_{\Gamma_\mu^-} d\mathcal{C}$ .

Equation (4.24) can be further written in terms of the dipole position,  $\mathbf{q}^\mu$ . Let  $\Delta\mathbf{q}^\mu$  be the location of the  $\mu$ -th dipole with respect to the center of mass. Because  $\Delta\mathbf{q}^\mu$  is oriented along its respective branch cut, we find that  $\int_{\Gamma_\mu} d\mathcal{C} = |\Delta\mathbf{q}^\mu| = \Delta q^\mu$  and

$$\hat{\epsilon}_{ij}^e = -\frac{1}{2A_0} \sum_{\mu=1}^{N_{\text{exc}}} \left[ b_i^\mu n_j^\mu + b_j^\mu n_i^\mu \right] \Delta q^\mu. \quad (4.25)$$

Furthermore,  $\Delta\mathbf{q}^\mu \cdot \mathbf{n}^\mu = 0$  as  $\Delta\mathbf{q}^\mu$  is perpendicular to  $\mathbf{n}^\mu$ . Since the Levi-Civita tensor can represent a clockwise 90° rotation with respect to the origin, we can write  $n_i^\mu = -\varepsilon_{ij} \Delta q_j^\mu / \Delta q^\mu$ . Substituting this result in Eq. (4.24), we arrive at

$$\hat{\epsilon}_{ij}^e = \frac{1}{2A_0} \sum_{\mu=1}^{N_{\text{exc}}} \left( b_i^\mu \varepsilon_{jk} \Delta q_k^\mu + b_j^\mu \varepsilon_{ik} \Delta q_k^\mu \right). \quad (4.26)$$

Using the correspondence between Burgers vectors and geometric dipoles (Eq. (2.42)),  $b_i = \varepsilon_{ij} d_j$  as well as the identity  $\varepsilon_{il} \varepsilon_{jk} = \delta_{ij} \delta_{lk} - \delta_{ik} \delta_{lj}$ , we obtain

$$\hat{\epsilon}_{ij}^e = \frac{1}{2A_0} \sum_{\mu=1}^{N_{\text{exc}}} \left( 2d_k^\mu \Delta q_k^\mu \delta_{ij} - d_i^\mu \Delta q_j^\mu - d_j^\mu \Delta q_i^\mu \right). \quad (4.27)$$

Equation (4.27) constitutes the most general formula for the area-averaged strain due to  $N_{\text{exc}}$ -many dipoles. Combined with Eqs. (4.18)–(4.20), they provide the final set of equations that we use to compute the renormalized elastic moduli. The computation of Eqs. (4.18)–(4.20) via the renormalization group (RG) method is provided in the next section, Section 5.

<sup>§</sup>The ‘branch cut’ terminology also carries a mathematical definition; it is the location of discontinuity for a function like  $u_i^\mu$  when viewing the 2D  $xy$ -plane as the complex plane. See Ref. [38] for a more extensive discussion.

Table 1: Table of fugacity parameter  $\tilde{y}$  at the onset temperature  $T_o$  for all model glass formers considered in this work. Although  $\tilde{y}$  is sufficiently small around the onset, a fugacity expansion may still be divergent due to the existence of critical fluctuations, hence the need for a perturbative RG method. For details on the model glass formers studied in this work, see Section 5.4.

| Model                                | Fugacity $\tilde{y}(T_o)$ | Onset Temperature $T_o$ |
|--------------------------------------|---------------------------|-------------------------|
| Poly-(12,0), ( $\varepsilon = 0.2$ ) | $2.7 \cdot 10^{-3}$       | 0.25                    |
| Poly-(12,6), ( $\varepsilon = 0.2$ ) | $2.6 \cdot 10^{-2}$       | 0.17                    |
| Poly-(18,0), ( $\varepsilon = 0.0$ ) | $8.5 \cdot 10^{-4}$       | 1.1                     |
| Poly-(18,0), ( $\varepsilon = 0.2$ ) | $7.0 \cdot 10^{-3}$       | 0.39                    |
| Poly-(10,6), ( $\varepsilon = 0.1$ ) | $3.9 \cdot 10^{-4}$       | 0.17                    |
| Poly-(10,6), ( $\varepsilon = 0.2$ ) | $1.6 \cdot 10^{-2}$       | 0.14                    |

## 5 Renormalization Group (RG) Analysis of Geometric Dipoles

In this section, we apply renormalization group (RG) techniques to compute the elastic moduli in Eqs. (4.18)–(4.20) and the melting point  $T_{KT}$ , following closely the analysis taken in Ref. [8]. We begin by explaining the strategy behind RG in Section 5.1 and highlight the usage of perturbative RG in the current theory. As a first step in implementing perturbative RG, we also develop in Section 5.1 a fugacity expansion of Eqs. (4.18)–(4.20) and use this expansion to derive the RG equations in Section 5.2. These equations are then analyzed around the melting point  $T_{KT}$  in Section 5.3, revealing the universal scaling behavior of the elastic moduli near  $T_{KT}$ . In Section 5.4, we calculate the renormalized elastic moduli for the atomistic models of glass formers used in this work, thereby determining their  $T_{KT}$ . Lastly, we close our analysis by evaluating the displacement and density correlations at  $T < T_{KT}$  in Section 5.5, where we confirm the recent observations from computer simulations that a 2D supercooled liquid can, indeed, behave as a 2D solid at the short intermediate timescales [12, 14].

The main difference between our analysis and the setup in Ref. [8] lies in the nature of the excitations/elastic defects. In our analysis, we have geometric dipoles that are able to attain continuous orientation angles due to the amorphous nature of the medium. In Ref. [8], the corresponding excitations are dislocations that can only attain discrete orientation angles as dictated by the underlying crystalline solid. This difference warrants a repeat of the RG analysis to see if any change exists. But for the expert readers, they may skip to the end of Section 5.2, in particular, Eqs. (5.130)–(5.133), which are the final RG equations derived from our analysis.

### 5.1 The Idea of RG and Fugacity Expansion

We are interested in computing elastic moduli, whose formulas are given by Eqs. (4.18)–(4.20), to predict the location of the melting point  $T_{KT}$ . Their computation requires ensemble averages of the following product of elastic strains:

$$\langle \hat{\epsilon}_{ij}^e \hat{\epsilon}_{kl}^e \rangle = \frac{1}{\Xi_{\text{exc}}} \sum_{N_{\text{exc}}=2}^{\infty} \frac{\tilde{y}^{N_{\text{exc}}}}{(a_{\text{dpl}})^{N_{\text{exc}}d} N_{\text{exc}}!} \int \prod_{\mu=1}^{N_{\text{exc}}} d^2 \mathbf{q}^{\mu} d\psi^{\mu} C(\{\psi^{\mu}\}) \hat{\epsilon}_{ij}^e \hat{\epsilon}_{kl}^e e^{-\tilde{\mathcal{H}}}, \quad (5.1)$$

where the formula for  $\hat{\epsilon}_{ij}^e$  is given in Eq. (4.27). A potentially feasible strategy for computing Eq. (5.1) is a perturbative expansion around  $\tilde{y} = 0$ , since  $\tilde{y} \sim \mathcal{O}(10^{-2})$  at most even around the onset temperature; see Table 1. This fugacity expansion, however, breaks down as  $T \rightarrow T_{KT}$  because the melting point is also a critical point. In other words, fluctuations do not average out at a finite

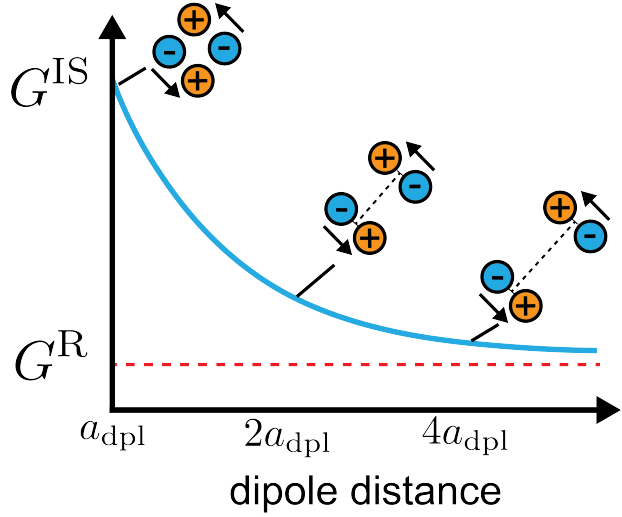

Figure S.14: An illustration of the RG flow, i.e., a solution to the RG equation, as applied to the renormalization of shear modulus. The RG method retrieves the renormalized value of the shear modulus by integrating sequentially the fluctuation corrections due to dipole pairs separated at different distances, feeding in the result from smaller scales to the integration of fluctuations at larger scales. This sequential integration results in a trajectory shown above, which is the evolution of  $G^{\text{IS}}$  as a function of lengthscale.

lengthscale and instead, persist from the smallest lengthscale  $a_{\text{dpl}}$  to the macroscopic lengthscale  $R$ . In the thermodynamic limit ( $R \rightarrow \infty$ ), this results in divergent integrals entering the expansion for any value of  $\tilde{y}$ .

The renormalization group (RG) method [35, 36] may be used to provide a self-consistent calculation of renormalized elastic moduli near the critical point. As applied to our problem, the RG method yields a set of ordinary differential equations (ODEs), i.e., the RG equations, that describe the scale transformation of the elastic moduli towards their renormalized values as a result of integrating fluctuations of dipole pairs separated at increasingly larger lengthscales; see Fig. S.14 for an illustration. Furthermore, studying the phase portrait of the RG equations can be used to understand the behavior of the system near the melting point. This is done by obtaining scaling relations and critical exponents from asymptotic solutions of the flow near the fixed point [35], which governs the location of the melting point.

The RG method used in this work follows that of the KTHNY theory [5, 8–11], and is perturbative in nature [35, 36]. In particular, the perturbative RG method requires an initial divergent expansion, e.g., a fugacity expansion, as input for constructing the RG equations since the scale invariance that needs to be incorporated into the RG flow is encoded within the divergent integrals entering the expansion<sup>†</sup>. Thus, a first step in applying RG to our problem is to develop the fugacity expansion of Eq. (5.1). This expansion is obtained by first Taylor expanding  $\frac{1}{\Xi_{\text{exc}}}$  around  $\tilde{y} = 0$  to yield

$$\frac{1}{\Xi_{\text{exc}}} = \frac{1}{1 + \sum_{N_{\text{exc}}=1}^{\infty} Z_{N_{\text{exc}}} \tilde{y}^{N_{\text{exc}}}} = 1 - Z_1 + \mathcal{O}(\tilde{y}^2) = 1 + \mathcal{O}(\tilde{y}^2), \quad (5.2)$$

where use is made of the dipole-moment conservation law to set  $Z_1 = 0$  in the second equality of Eq. (5.2), i.e., a single dipole cannot obey the dipole-moment conservation. Substituting Eq. (5.2)

<sup>†</sup>A more expanded discussion on the ideas behind perturbative RG is provided in Section 5.2.

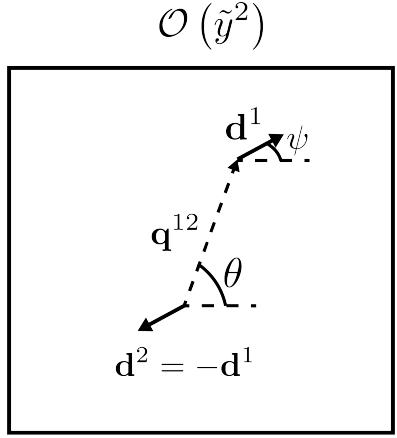

Figure S.15: Illustration for the configuration considered in  $\mathcal{O}(y^2)$  of the perturbation theory. If only two dipoles are present, then the line discontinuity from each dipole is parallel with each other and is oriented along the pair distance vector  $\mathbf{q}^{12}$ .

into Eq. (5.1) gives us

$$\langle \hat{\epsilon}_{ij}^e \hat{\epsilon}_{kl}^e \rangle = \sum_{m=2}^{\infty} (\hat{\epsilon}_{ij}^e \hat{\epsilon}_{kl}^e)_m \tilde{y}^m, \quad (5.3)$$

where  $(\hat{\epsilon}_{ij}^e \hat{\epsilon}_{kl}^e)_m$  is the  $m$ -th-order coefficient of the fugacity expansion of  $\hat{\epsilon}_{ij}^e \hat{\epsilon}_{kl}^e$ , with the first two coefficients written as

$$(\hat{\epsilon}_{ij}^e \hat{\epsilon}_{kl}^e)_2 = \frac{1}{(a_{\text{dpl}})^4 2!} \int \prod_{\mu=1}^2 d^2 \mathbf{q}^{\mu} d\psi^{\mu} C(\{\psi^{\mu}\}) \hat{\epsilon}_{ij}^e \hat{\epsilon}_{kl}^e e^{-\tilde{\mathcal{H}}}, \quad (5.4)$$

$$(\hat{\epsilon}_{ij}^e \hat{\epsilon}_{kl}^e)_3 = \frac{1}{(a_{\text{dpl}})^6 3!} \int \prod_{\mu=1}^3 d^2 \mathbf{q}^{\mu} d\psi^{\mu} C(\{\psi^{\mu}\}) \hat{\epsilon}_{ij}^e \hat{\epsilon}_{kl}^e e^{-\tilde{\mathcal{H}}}, \quad (5.5)$$

and higher-order coefficients may be obtained manually or via diagrammatic techniques such as the Ursell-Mayer cluster expansion method [23]. For the analysis of the RG flow, we develop the expansion up to  $\mathcal{O}(\tilde{y}^3)$ . The general formulas for both the  $\mathcal{O}(\tilde{y}^2)$  and  $\mathcal{O}(\tilde{y}^3)$  terms are developed in the next two subsections.

### Order $\mathcal{O}(\tilde{y}^2)$

To begin, consider the configuration of two dipoles in Fig. S.15, which we use for the second-order calculation. We first simplify the general strain formula in Eq. (4.27) to the case of two dipoles,

$$\hat{\epsilon}_{ij}^e = \frac{1}{2A_0} (2d_k^1 \Delta q_k^1 \delta_{ij} - d_i^1 \Delta q_j^1 - d_j^1 \Delta q_i^1 + 2d_k^2 \Delta q_k^2 \delta_{ij} - d_i^2 \Delta q_j^2 - d_j^2 \Delta q_i^2), \quad (5.6)$$

where  $\Delta \mathbf{q}^{\mu}$  is the position of the  $\mu$ -th dipole with respect to the many-dipole center of mass. Letting  $\mathbf{q}^{12} = \mathbf{q}^1 - \mathbf{q}^2$ , Eq. (5.6) can be further reduced upon noting that the line discontinuities from each dipole align with each other when only two dipoles are present (Fig. S.15). Since  $\Delta \mathbf{q}^{\mu}$  is oriented along each line discontinuity, this implies that  $\Delta \mathbf{q}^1 = -\Delta \mathbf{q}^2 = \mathbf{q}^{12}/2$ , which in turn gives

$$\hat{\epsilon}_{ij}^e = \frac{1}{2A_0} \left( d_k^{12} q_k^{12} \delta_{ij} - \frac{d_i^{12} q_j^{12} + d_j^{12} q_i^{12}}{2} \right), \quad (5.7)$$

where  $d_k^{12} = d_k^1 - d_k^2$  is the difference in the dipole-moment vectors.

We now proceed to compute the second-order coefficient by noting from the dipole-moment conservation law that the dipole-moment vector  $\mathbf{d}^1 = -\mathbf{d}^2$ . This reduces the orientational degrees of freedom to one, turning Eq. (5.4) into

$$(\hat{\epsilon}_{ij}^e \hat{\epsilon}_{kl}^e)_2 = \frac{1}{(a_{\text{dpl}})^4 2!} \int \prod_{\mu=1}^2 d^2 \mathbf{q}^\mu \int_0^{2\pi} d\psi^1 \hat{\epsilon}_{ij}^e \hat{\epsilon}_{kl}^e e^{-\tilde{\mathcal{H}}}. \quad (5.8)$$

Let us write in polar coordinates  $\mathbf{q}^{12} = q^{12} [\cos \theta^{12}, \sin \theta^{12}]$  and  $\mathbf{d}^\mu = d_c [\cos \psi^\mu, \sin \psi^\mu]$ . The effective Hamiltonian in Eq. (3.61) for the two-dipole case is

$$\tilde{\mathcal{H}} = -\frac{\tilde{Y}^{\text{IS}}}{4\pi} \left[ -(\tilde{\mathbf{d}}^1 \cdot \tilde{\mathbf{d}}^1) \left( \ln \frac{q^{12}}{a_{\text{dpl}}} - 1 \right) - \frac{(\tilde{\mathbf{d}}^1 \cdot \mathbf{q}^{12})(\tilde{\mathbf{d}}^1 \cdot \mathbf{q}^{12})}{(q^{12})^2} \right] \quad (5.9)$$

$$= -\frac{\tilde{Y}^{\text{IS}}}{4\pi} \left[ -\ln \frac{q^{12}}{a_{\text{dpl}}} - (\cos^2(\theta^{12} - \psi^1) - 1) \right] \quad (5.10)$$

$$= -\frac{\tilde{Y}^{\text{IS}}}{4\pi} \left[ -\ln \frac{q^{12}}{a_{\text{dpl}}} + \frac{1}{2}(1 - \cos(2\psi^1 - 2\theta^{12})) \right]. \quad (5.11)$$

Switching to a barycentric coordinate system

$$\mathbf{Q} = \frac{\mathbf{q}^1 + \mathbf{q}^2}{2}, \quad \mathbf{q} = \mathbf{q}^1 - \mathbf{q}^2, \quad \psi = \psi^1, \quad (5.12)$$

which provides a linear transformation of  $(\mathbf{q}^1, \mathbf{q}^2) \rightarrow (\mathbf{Q}, \mathbf{q})$  that has unit determinant, we can express the Hamiltonian in Eq. (5.11) and the integration in Eq. (5.8) as

$$\tilde{\mathcal{H}} = -\frac{\tilde{Y}^{\text{IS}}}{4\pi} \left[ -\ln \frac{q}{a_{\text{dpl}}} + \frac{1}{2}(1 - \cos(2\psi - 2\theta)) \right], \quad (5.13)$$

$$\int \prod_{\mu=1}^2 d^2 \mathbf{q}^\mu = \int d^2 \mathbf{Q} \int d^2 \mathbf{q} = A_0 \int d^2 \mathbf{q}, \quad (5.14)$$

respectively, where  $\int d^2 \mathbf{Q} = A_0$  since neither the Hamiltonian nor the strain formulas depend on  $\mathbf{Q}$  at this level of perturbation theory. Substituting Eqs. (5.13) and (5.14) into Eq. (5.8) yields

$$(\hat{\epsilon}_{ij}^e \hat{\epsilon}_{kl}^e)_2 = \frac{A_0 e^{\frac{\tilde{Y}^{\text{IS}}}{8\pi}}}{(a_{\text{dpl}})^4 2!} \int d^2 \mathbf{q} \int_0^{2\pi} d\psi \hat{\epsilon}_{ij}^e \hat{\epsilon}_{kl}^e \left( \frac{q}{a_{\text{dpl}}} \right)^{\frac{-\tilde{Y}^{\text{IS}}}{4\pi}} e^{-\frac{\tilde{Y}^{\text{IS}}}{8\pi} \cos(2\psi - 2\theta)}. \quad (5.15)$$

Switching to polar coordinates for  $\mathbf{q} = q [\cos \theta, \sin \theta]$ , we can write Eq. (5.15) as

$$(\hat{\epsilon}_{ij}^e \hat{\epsilon}_{kl}^e)_2 = \frac{A_0 e^{\frac{\tilde{Y}^{\text{IS}}}{8\pi}}}{(a_{\text{dpl}})^2 2!} \int_{a_{\text{dpl}}}^R \frac{dq}{a_{\text{dpl}}} \int_0^{2\pi} d\theta \int_0^{2\pi} d\psi \hat{\epsilon}_{ij}^e \hat{\epsilon}_{kl}^e \left( \frac{q}{a_{\text{dpl}}} \right)^{1 - \frac{\tilde{Y}^{\text{IS}}}{4\pi}} e^{-\frac{\tilde{Y}^{\text{IS}}}{8\pi} \cos(2\psi - 2\theta)}, \quad (5.16)$$

which is the most general formula for the second-order coefficient in the fugacity expansion.

Although Eq. (5.16) is expressed in terms of a tensorial product, the fluctuation formulas for the elastic moduli in Eqs. (4.18)–(4.20) require only two kinds of products, namely  $\hat{\epsilon}_{ii}^e \hat{\epsilon}_{kk}^e$  and  $\hat{\epsilon}_{ij}^e \hat{\epsilon}_{ij}^e$ . These products of strains have a more compact form in polar coordinates when only two dipoles are involved. To see this, we first compute the following product of strains:

$$\hat{\epsilon}_{ii}^e \hat{\epsilon}_{kk}^e = \frac{1}{4A_0^2} (2d_i^{12} q_i^{12} - d_i^{12} q_i^{12}) (2d_k^{12} q_k^{12} - d_k^{12} q_k^{12}) = \frac{1}{4A_0^2} (\mathbf{d}^{12} \cdot \mathbf{q}^{12})^2. \quad (5.17)$$

Note that Eq. (5.17) contributes to the renormalization of the bulk modulus; see Eq. (4.18). Letting  $\mathbf{d}^{12} = d_c[\cos \psi^1 - \cos \psi^2, \sin \psi^1 - \sin \psi^2]$ , the dot product in the second equality of Eq. (5.17) can be written in terms of trigonometric functions,

$$\mathbf{d}^{12} \cdot \mathbf{q}^{12} = d_c q^{12} (\cos(\psi^1 - \theta^{12}) - \cos(\psi^2 - \theta^{12})) \quad (5.18)$$

$$= -2d_c q^{12} \sin\left(\frac{\delta\psi^{12}}{2}\right) \sin(\Psi^{12} - \theta^{12}), \quad (5.19)$$

where  $\delta\psi^{12} = \psi^1 - \psi^2$  and  $\Psi^{12} = \frac{\psi^1 + \psi^2}{2}$ . To obey the dipole-moment conservation law,  $d_i^1 = -d_i^2$  and this implies that  $\delta\psi^{12} = \pi$ . Substituting  $\delta\psi^{12} = \pi$  into Eq. (5.19) yields

$$\mathbf{d}^{12} \cdot \mathbf{q}^{12} = -2d_c q^{12} \sin\left(\psi^1 - \frac{\pi}{2} - \theta^{12}\right) = 2d_c q^{12} \cos(\psi^1 - \theta^{12}), \quad (5.20)$$

$$(\mathbf{d}^{12} \cdot \mathbf{q}^{12})^2 = 4(d_c q^{12})^2 \cos^2(\psi^1 - \theta^{12}) = 2(d_c q^{12})^2 (1 + \cos(2\psi^1 - 2\theta^{12})). \quad (5.21)$$

Substituting Eq. (5.21) into Eq. (5.17) gives us the following formula:

$$\hat{\epsilon}_{ii}^e \hat{\epsilon}_{kk}^e = \frac{(d_c q^{12})^2}{2A_0^2} (1 + \cos(2\psi^1 - 2\theta^{12})). \quad (5.22)$$

We may also write Eq. (5.22) in terms of the polar coordinates entering the general formula for the second-order coefficient in Eq. (5.16), where  $\theta^{12} \rightarrow \theta$ ,  $\psi^1 \rightarrow \psi$ , and  $q^{12} \rightarrow q$ . This yields,

$$\hat{\epsilon}_{ii}^e \hat{\epsilon}_{kk}^e = \frac{(d_c q)^2}{2A_0^2} (1 + \cos(2\psi - 2\theta)). \quad (5.23)$$

The next product of strains to compute is

$$\hat{\epsilon}_{ij}^e \hat{\epsilon}_{ij}^e = \frac{1}{4A_0^2} \left( d_k^{12} q_k^{12} \delta_{ij} - \frac{d_i^{12} q_j^{12} + d_j^{12} q_i^{12}}{2} \right) \left( d_m^{12} q_m^{12} \delta_{ij} - \frac{d_i^{12} q_j^{12} + d_j^{12} q_i^{12}}{2} \right) \quad (5.24)$$

$$= \frac{1}{8A_0^2} \left[ (d_k^{12} q_k^{12})^2 + (d_k^{12} d_k^{12}) (q_k^{12} q_k^{12}) \right], \quad (5.25)$$

which contributes to the renormalization of the shear modulus in Eq. (4.19). In vector notation, Eq. (5.25) can be written as

$$\hat{\epsilon}_{ij}^e \hat{\epsilon}_{ij}^e = \frac{1}{8A_0^2} \left[ (\mathbf{d}^{12} \cdot \mathbf{q}^{12})^2 + |\mathbf{d}^{12}|^2 |\mathbf{q}^{12}|^2 \right]. \quad (5.26)$$

The second term in the parentheses of Eq. (5.26) can again be expressed in terms of trigonometric functions,

$$|\mathbf{d}^{12}|^2 |\mathbf{q}^{12}|^2 = (d_c q^{12})^2 [(\cos \psi^1 - \cos \psi^2)^2 + (\sin \psi^1 - \sin \psi^2)^2] \quad (5.27)$$

$$= 2(d_c q^{12})^2 (1 - \cos \delta\psi^{12}). \quad (5.28)$$

Substituting  $\delta\psi^{12} = \pi$  into Eq. (5.28) yields

$$|\mathbf{d}^{12}|^2 |\mathbf{q}^{12}|^2 = 2(d_c q^{12})^2, \quad (5.29)$$

and further substituting Eq. (5.29) into Eq. (5.26), we obtain

$$\hat{\epsilon}_{ij}^e \hat{\epsilon}_{ij}^e = \frac{(d_c q^{12})^2}{4A_0^2} [3 + \cos(2\psi^1 - 2\theta^{12})] . \quad (5.30)$$

In terms of the polar coordinates entering Eq. (5.16), we can re-write Eq. (5.30) as

$$\hat{\epsilon}_{ij}^e \hat{\epsilon}_{ij}^e = \frac{(d_c q)^2}{4A_0^2} (3 + \cos(2\psi - 2\theta)) . \quad (5.31)$$

Applying the second-order coefficient formula in Eq. (5.16) to the strain products given in Eqs. (5.23) and (5.31), we find that

$$(\hat{\epsilon}_{ii}^e \hat{\epsilon}_{kk}^e)_2 = \frac{(d_c)^2}{2A_0^2} (\mathcal{P}^{(1)} + \mathcal{P}^{(2)}) , \quad (5.32)$$

$$(\hat{\epsilon}_{ij}^e \hat{\epsilon}_{ij}^e)_2 = \frac{(d_c)^2}{4A_0^2} (3\mathcal{P}^{(1)} + \mathcal{P}^{(2)}) , \quad (5.33)$$

where  $\mathcal{P}^{(1)}$  and  $\mathcal{P}^{(2)}$  are the two integrals that needed to be evaluated explicitly,

$$\mathcal{P}^{(1)} = \frac{A_0 e^{\frac{\tilde{\gamma}^{\text{IS}}}{8\pi}}}{(a_{\text{dpl}})^2 2!} \int_{a_{\text{dpl}}}^R \frac{dq}{a_{\text{dpl}}} \int_0^{2\pi} d\theta \int_0^{2\pi} d\psi q^2 \left( \frac{q}{a_{\text{dpl}}} \right)^{1 - \frac{\tilde{\gamma}^{\text{IS}}}{4\pi}} e^{-\cos(2\psi - 2\theta)} \quad (5.34)$$

$$= \frac{A_0 e^{\frac{\tilde{\gamma}^{\text{IS}}}{8\pi}}}{2!} \int_{a_{\text{dpl}}}^R \frac{dq}{a_{\text{dpl}}} \left( \frac{q}{a_{\text{dpl}}} \right)^{3 - \frac{\tilde{\gamma}^{\text{IS}}}{4\pi}} \left( \int_0^{2\pi} d\theta \int_0^{2\pi} d\psi e^{-\frac{\tilde{\gamma}^{\text{IS}}}{8\pi} \cos(2\psi - 2\theta)} \right) , \quad (5.35)$$

$$\mathcal{P}^{(2)} = \frac{A_0 e^{\frac{\tilde{\gamma}^{\text{IS}}}{8\pi}}}{(a_{\text{dpl}})^2 2!} \int_{a_{\text{dpl}}}^R \frac{dq}{a_{\text{dpl}}} \int_0^{2\pi} d\theta \int_0^{2\pi} d\psi q^2 \left( \frac{q}{a_{\text{dpl}}} \right)^{1 - \frac{\tilde{\gamma}^{\text{IS}}}{4\pi}} \cos(2\psi - 2\theta) e^{-\cos(2\psi - 2\theta)} \quad (5.36)$$

$$= \frac{A_0 e^{\frac{\tilde{\gamma}^{\text{IS}}}{8\pi}}}{2!} \int_{a_{\text{dpl}}}^R \frac{dq}{a_{\text{dpl}}} \left( \frac{q}{a_{\text{dpl}}} \right)^{3 - \frac{\tilde{\gamma}^{\text{IS}}}{4\pi}} \left( \int_0^{2\pi} d\theta \int_0^{2\pi} d\psi \cos(2\psi - 2\theta) e^{-\frac{\tilde{\gamma}^{\text{IS}}}{8\pi} \cos(2\psi - 2\theta)} \right) . \quad (5.37)$$

To simplify the expressions in Eqs. (5.35) and (5.37), we first evaluate the angular integral in Eq. (5.35) using the following Bessel function identity:

$$\int_0^{2\pi} d\theta \int_0^{2\pi} d\psi e^{-\frac{\tilde{\gamma}^{\text{IS}}}{8\pi} \cos(2\psi - 2\theta)} = (2\pi)^2 I_0 \left( \frac{\tilde{\gamma}^{\text{IS}}}{8\pi} \right) , \quad (5.38)$$

where  $I_n(x)$  denotes the  $n$ -th order modified Bessel function of the first kind. Substituting Eq. (5.38) into Eq. (5.35) yields

$$\mathcal{P}^{(1)} = 2\pi^2 A_0 e^{\frac{\tilde{\gamma}^{\text{IS}}}{8\pi}} I_0 \left( \frac{\tilde{\gamma}^{\text{IS}}}{8\pi} \right) \int_{a_{\text{dpl}}}^R \frac{dq}{a_{\text{dpl}}} \left( \frac{q}{a_{\text{dpl}}} \right)^{3 - \frac{\tilde{\gamma}^{\text{IS}}}{4\pi}} . \quad (5.39)$$

On the other hand, the angular integral in Eq. (5.37) can be simplified using another Bessel function identity

$$\int_0^{2\pi} d\theta \int_0^{2\pi} d\psi \cos(2\psi - 2\theta) e^{-\frac{\tilde{\gamma}^{\text{IS}}}{8\pi} \cos(2\psi - 2\theta)} = -(2\pi)^2 I_1 \left( \frac{\tilde{\gamma}^{\text{IS}}}{8\pi} \right) , \quad (5.40)$$

which turns Eq. (5.37) into

$$\mathcal{P}^{(2)} = -2\pi^2 A_0 e^{\frac{\tilde{Y}^{\text{IS}}}{8\pi}} I_1 \left( \frac{\tilde{Y}^{\text{IS}}}{8\pi} \right) \int_{a_{\text{dpl}}}^R \frac{dq}{a_{\text{dpl}}} \left( \frac{q}{a_{\text{dpl}}} \right)^{3 - \frac{\tilde{Y}^{\text{IS}}}{4\pi}}. \quad (5.41)$$

Equations (5.32), (5.33), (5.39) and (5.41) constitute the final results of the second-order perturbation theory. Before we move on to the third-order calculation, we highlight that the integral responsible for the divergence of the perturbation theory is

$$\mathcal{I} = \int_{a_{\text{dpl}}}^R \frac{dq}{a_{\text{dpl}}} \left( \frac{q}{a_{\text{dpl}}} \right)^{3 - \frac{\tilde{Y}^{\text{IS}}}{4\pi}} = \frac{1}{4 - \frac{\tilde{Y}^{\text{IS}}}{4\pi}} \left[ \left( \frac{R}{a_{\text{dpl}}} \right)^{4 - \frac{\tilde{Y}^{\text{IS}}}{4\pi}} - 1 \right] \quad (5.42)$$

and it diverges when  $R \rightarrow \infty$  if  $\tilde{Y}^{\text{IS}} \leq 16\pi$ . The point that signals the onset of divergence,  $\tilde{Y}^{\text{IS}} = 16\pi$ , coincides with the binding-unbinding transition predicted by energy-entropy arguments (see Section 3).

### Order $\mathcal{O}(\tilde{y}^3)$

Applying the dipole-moment conservation law to the configuration of dipoles in Fig. S.16(b), we find that

$$\psi^2 = \psi^1 + 2\pi/3, \quad \psi^3 = \psi^1 - 2\pi/3. \quad (5.43)$$

This leaves us with one orientational degree of freedom  $\psi^1$ , and thus the third-order coefficient in Eq. (5.5) can be written as

$$(\hat{\epsilon}_{ij}^e \hat{\epsilon}_{kl}^e)_3 = \frac{1}{(a_{\text{dpl}})^6 3!} \int \prod_{\mu=1}^3 d^2 \mathbf{q}^\mu \int_0^{2\pi} d\psi^1 \hat{\epsilon}_{ij}^e \hat{\epsilon}_{kl}^e e^{-\tilde{\mathcal{H}}}. \quad (5.44)$$

Following the KTHNY theory, in particular the analysis of Ref. [8–11], we assume that the effect of the three-body interaction is to yield an effective two-body interaction between a dipole and a composite dipole made up of two dipoles, e.g., dipole (2) and (3) in Fig. S.16(b). This approximation introduces a cut-off lengthscale  $r_{\text{max}}$  that sets the maximum distance in which dipole (2) and (3) can be separated, allowing us to treat the two dipoles as a composite one. The choice of  $r_{\text{max}}$  is tied to the renormalization scheme of the RG method, and thus its further discussion will be delegated to Section 5.2.

At this stage, we proceed with applying the composite-dipole approximation to the general strain formula in Eq. (4.27). For the three-dipole case, we have

$$\hat{\epsilon}_{ij}^e = \frac{1}{2A_0} \sum_{\mu=1}^3 \left( 2d_k^\mu \Delta q_k^\mu \delta_{ij} - d_i^\mu \Delta q_j^\mu - d_j^\mu \Delta q_i^\mu \right). \quad (5.45)$$

Let us set the center of mass of dipole (2) and (3) as the position of the composite dipole  $\mathbf{q}^{2*} := \frac{\mathbf{q}^2 + \mathbf{q}^3}{2}$ . According to Fig. S.16(b), the pair distance  $\mathbf{q}^{23} = \mathbf{q}^2 - \mathbf{q}^3 \approx 0$ , and thus  $\Delta \mathbf{q}^2 \approx \Delta \mathbf{q}^3 \approx \Delta \mathbf{q}^{2*}$ . Defining  $d_i^{2*} = d_k^2 + d_k^3$  as the dipole-moment vector of the composite dipole, we find that the approximation turns Eq. (5.45) into

$$\hat{\epsilon}_{ij}^e \approx \frac{1}{2A_0} \left( 2d_k^1 \Delta q_k^1 \delta_{ij} - d_i^1 \Delta q_j^1 - d_j^1 \Delta q_i^1 + 2d_k^{2*} \Delta q_k^{2*} \delta_{ij} - d_i^{2*} \Delta q_j^{2*} - d_j^{2*} \Delta q_i^{2*} \right). \quad (5.46)$$

$\mathcal{O}(\tilde{y}^3)$

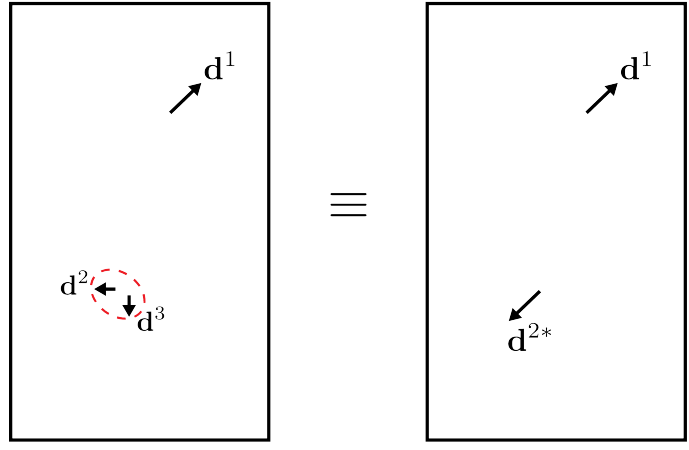

Figure S.16: Illustrations for configurations considered in  $\mathcal{O}(y^3)$  of the perturbation theory. As seen in Eq. (5.59), interaction between dipole and composite dipole is identical to that of regular dipole pair. However, the internal DOFs of the composite dipole contributes to an additional term (Eq. (5.60)) in the final Hamiltonian.

Similar to the  $\mathcal{O}(\tilde{y}^2)$  calculation, we use the fact that in a two-body problem,  $\Delta q_i^1 = q_i^{12*}/2$  and  $\Delta q_i^{2*} = -q_i^{12*}/2$  so that Eq. (5.46) becomes

$$\tilde{\epsilon}_{ij}^e \approx \frac{1}{2A_0} \left( d_k^{12*} q_k^{12*} \delta_{ij} - \frac{d_i^{12*} q_j^{12*} + d_j^{12*} q_i^{12*}}{2} \right), \quad (5.47)$$

where  $d_j^{12*} = d_j^1 - d_j^{2*}$ . Equation (5.47) is identical in form to the two-dipole case in Eq. (5.7). Thus, the area-averaged strain of a three-dipole system turns into that of an effective two-dipole system under the composite-dipole approximation.

Next, we apply the composite-dipole approximation to the computation of the third-order coefficient in Eq. (5.44). The approximation turns the Hamiltonian  $\mathcal{H}$  into a sum of a new effective Hamiltonian  $\tilde{\mathcal{H}}_{\text{cd}}$ , which describes the interaction of a dipole with a composite dipole, as well as another Hamiltonian  $\tilde{\mathcal{H}}_{\text{int}}$ , which describes the internal DOFs of the composite dipole. To derive these new Hamiltonians, we first write down the original Hamiltonian in Eq. (3.61) for the three-body problem in polar coordinates,

$$\begin{aligned} \tilde{\mathcal{H}} = -\frac{\tilde{Y}^{\text{IS}}}{4\pi} & \left[ \cos \delta \psi^{12} \left( \ln \frac{q^{12}}{a_{\text{dpl}}} - 1 \right) + \cos(\theta^{12} - \psi^1) \cos(\theta^{12} - \psi^2) \right. \\ & + \cos \delta \psi^{13} \left( \ln \frac{q^{13}}{a_{\text{dpl}}} - 1 \right) + \cos(\theta^{13} - \psi^1) \cos(\theta^{13} - \psi^3) \\ & \left. + \cos \delta \psi^{23} \left( \ln \frac{q^{23}}{a_{\text{dpl}}} - 1 \right) + \cos(\theta^{23} - \psi^2) \cos(\theta^{23} - \psi^3) \right], \end{aligned} \quad (5.48)$$

where  $\delta \psi^{\mu\gamma} = \psi^\mu - \psi^\gamma$ . Substituting Eq. (5.43) into Eq. (5.48), we obtain

$$\begin{aligned} \tilde{\mathcal{H}} = -\frac{\tilde{Y}^{\text{IS}}}{4\pi} & \left[ -\frac{1}{2} \left( \ln \frac{q^{12}}{a_{\text{dpl}}} - 1 \right) + \cos(\theta^{12} - \psi^1) \cos(\theta^{12} - \psi^1 - 2\pi/3) \right. \\ & \left. -\frac{1}{2} \left( \ln \frac{q^{13}}{a_{\text{dpl}}} - 1 \right) + \cos(\theta^{13} - \psi^1) \cos(\theta^{13} - \psi^1 + 2\pi/3) \right. \\ & \left. -\frac{1}{2} \left( \ln \frac{q^{23}}{a_{\text{dpl}}} - 1 \right) + \cos(\theta^{23} - \psi^2) \cos(\theta^{23} - \psi^2 + 2\pi/3) \right] \end{aligned}$$

$$-\frac{1}{2} \left( \ln \frac{q^{23}}{a_{\text{dpl}}} - 1 \right) + \cos(\theta^{23} - \psi^1 - 2\pi/3) \cos(\theta^{23} - \psi^1 + 2\pi/3) \Big]. \quad (5.49)$$

Defining a new set of coordinates

$$\mathbf{q} = \mathbf{q}^1 - \frac{\mathbf{q}^2 + \mathbf{q}^3}{2}, \quad \mathbf{Q}' = \frac{\mathbf{q}^2 + \mathbf{q}^3}{2}, \quad \mathbf{q}' = \mathbf{q}^2 - \mathbf{q}^3, \quad \psi = \psi^1, \quad (5.50)$$

which yields a unit determinant for the linear transformation  $(\mathbf{q}^1, \mathbf{q}^2, \mathbf{q}^3) \rightarrow (\mathbf{q}, \mathbf{q}', \mathbf{Q})$ , we can express the integral in Eq. (5.5) as

$$\int \prod_{\mu=1}^3 d^2 \mathbf{q}^\mu = \int d^2 \mathbf{q} \int d^2 \mathbf{q}' \int d\mathbf{Q}' = A_0 \int d^2 \mathbf{q} \int d^2 \mathbf{q}', \quad (5.51)$$

where we integrated  $\mathbf{Q}'$  in the second equality since neither the Hamiltonian nor the pair-wise observable will depend on  $\mathbf{Q}'$ . Under the composite-dipole approximation,  $|\mathbf{q}'| < r_{\text{max}} \ll |\mathbf{q}|$ , where  $r_{\text{max}}$  is the maximum length of separation between dipole (2) and (3), and thus

$$\mathbf{q}^{12} = \mathbf{q} - \frac{\mathbf{q}'}{2} \approx \mathbf{q}, \quad \mathbf{q}^{13} = \mathbf{q} + \frac{\mathbf{q}'}{2} \approx \mathbf{q}. \quad (5.52)$$

Equation (5.52) implies that the pair distance between dipole (1) and the dipoles making up the composite dipole is approximately equal to the pair distance between dipole (1) and the two-dipole center of mass  $\mathbf{Q}'$ , which act as the position of the composite dipole.

At this stage, we may use Eq. (5.52) to reduce Eq. (5.49) into

$$\begin{aligned} \tilde{\mathcal{H}} \approx & -\frac{\tilde{Y}^{\text{IS}}}{4\pi} \left[ -\frac{1}{2} \left( \ln \frac{q}{a_{\text{dpl}}} - 1 \right) + \cos(\theta - \psi) \cos(\theta - \psi - 2\pi/3) \right. \\ & -\frac{1}{2} \left( \ln \frac{q}{a_{\text{dpl}}} - 1 \right) + \cos(\theta - \psi) \cos(\theta - \psi + 2\pi/3) \\ & \left. -\frac{1}{2} \left( \ln \frac{q'}{a_{\text{dpl}}} - 1 \right) + \cos(\theta' - \psi - 2\pi/3) \cos(\theta' - \psi + 2\pi/3) \right] \end{aligned} \quad (5.53)$$

$$\begin{aligned} = & -\frac{\tilde{Y}^{\text{IS}}}{4\pi} \left[ -\left( \ln \frac{q}{a_{\text{dpl}}} - 1 \right) + \cos(\theta - \psi) (\cos(\theta - \psi - 2\pi/3) + \cos(\theta - \psi + 2\pi/3)) \right. \\ & \left. -\frac{1}{2} \left( \ln \frac{q'}{a_{\text{dpl}}} - 1 \right) + \cos(\theta' - \psi - 2\pi/3) \cos(\theta' - \psi + 2\pi/3) \right]. \end{aligned} \quad (5.54)$$

Using the following trigonometric identities:

$$\cos(x) (\cos(x - 2\pi/3) + \cos(x + 2\pi/3)) = -\cos^2 x = -\frac{1}{2} (1 + \cos(2x)), \quad (5.55)$$

$$\cos(x - 2\pi/3) \cos(x + 2\pi/3) = \frac{1}{4} (-1 + 2 \cos(2x)), \quad (5.56)$$

we can simplify Eq. (5.54) into

$$\tilde{\mathcal{H}} \approx -\frac{\tilde{Y}^{\text{IS}}}{4\pi} \left[ -\ln \frac{q}{a_{\text{dpl}}} + \frac{1}{2} (1 - \cos(2\theta - 2\psi)) - \frac{1}{2} \ln \frac{q'}{a_{\text{dpl}}} + \frac{1}{4} (1 + 2 \cos(2\theta' - 2\psi)) \right] \quad (5.57)$$

$$= \tilde{\mathcal{H}}_{\text{cd}} + \tilde{\mathcal{H}}_{\text{int}}, \quad (5.58)$$

where the effective Hamiltonian

$$\tilde{\mathcal{H}}_{\text{cd}} = -\frac{\tilde{Y}^{\text{IS}}}{4\pi} \left[ -\ln \frac{q}{a_{\text{dpl}}} + \frac{1}{2} (1 - \cos(2\theta - 2\psi)) \right] \quad (5.59)$$

is identical to the two-body interaction of regular dipoles (see Eq. (5.13)), and the new Hamiltonian

$$\tilde{\mathcal{H}}_{\text{int}} = -\frac{\tilde{Y}^{\text{IS}}}{4\pi} \left[ -\frac{1}{2} \ln \frac{q'}{a_{\text{dpl}}} + \frac{1}{4} (1 + 2 \cos(2\theta' - 2\psi)) \right] \quad (5.60)$$

governs the separation length and relative orientation of dipoles (2) and (3), which now act as the internal DOFs of the composite dipole.

The third-order coefficient in Eq. (5.44) can now be approximated with Eqs. (5.58) and (5.60), which yields

$$(\hat{\epsilon}_{ij}^e \hat{\epsilon}_{kl}^e)_3 \approx \frac{A_0}{(a_{\text{dpl}})^6 1!1!} \int d^2 \mathbf{q} \int d^2 \mathbf{q}' d\psi \hat{\epsilon}_{ij}^e \hat{\epsilon}_{kl}^e e^{-\tilde{\mathcal{H}}_{\text{cd}}} e^{-\tilde{\mathcal{H}}_{\text{int}}}, \quad (5.61)$$

where the formula for  $\hat{\epsilon}_{ij}^e$  is given in Eq. (5.47). Note that the  $1!1!$  factorial in Eq. (5.61) replaces the  $3!$  factorial in Eq. (5.44) because there are now two distinguishable dipoles instead of three indistinguishable dipoles in the system. Using Eqs. (5.59) and (5.60), we write the following Boltzmann factors

$$e^{-\tilde{\mathcal{H}}_{\text{cd}}} = e^{-\frac{\tilde{Y}^{\text{IS}}}{8\pi}} \left( \frac{q}{a_{\text{dpl}}} \right)^{-\frac{\tilde{Y}^{\text{IS}}}{4\pi}} e^{-\frac{\tilde{Y}^{\text{IS}}}{8\pi} \cos(2\theta - 2\psi)}, \quad e^{-\tilde{\mathcal{H}}_{\text{int}}} = e^{-\frac{\tilde{Y}^{\text{IS}}}{16\pi}} \left( \frac{q'}{a_{\text{dpl}}} \right)^{-\frac{\tilde{Y}^{\text{IS}}}{8\pi}} e^{\frac{\tilde{Y}^{\text{IS}}}{8\pi} \cos(2\theta' - 2\psi)} \quad (5.62)$$

to write Eq. (5.61) as

$$\begin{aligned} (\hat{\epsilon}_{ij}^e \hat{\epsilon}_{kl}^e)_3 &= \frac{A_0}{(a_{\text{dpl}})^6} \int_0^{2\pi} d\psi \left( \int d^2 \mathbf{q} \hat{\epsilon}_{ij}^e \hat{\epsilon}_{kl}^e e^{-\frac{\tilde{Y}^{\text{IS}}}{8\pi}} \left( \frac{q}{a_{\text{dpl}}} \right)^{-\frac{\tilde{Y}^{\text{IS}}}{4\pi}} e^{-\frac{\tilde{Y}^{\text{IS}}}{8\pi} \cos(2\theta - 2\psi)} \right) \\ &\quad \times \left( \int d^2 \mathbf{q}' e^{-\frac{\tilde{Y}^{\text{IS}}}{16\pi}} \left( \frac{q'}{a_{\text{dpl}}} \right)^{-\frac{\tilde{Y}^{\text{IS}}}{8\pi}} e^{\frac{\tilde{Y}^{\text{IS}}}{8\pi} \cos(2\theta' - 2\psi)} \right). \end{aligned} \quad (5.63)$$

Combined with Eq. (5.47), Eq. (5.63) constitutes the most general formula for the third-order coefficient of the perturbation theory under the composite-dipole approximation.

Since the strain formula in Eq. (5.47) is identical to the two-body one, the corresponding formulas for the strain products  $\hat{\epsilon}_{ii}^e \hat{\epsilon}_{kk}^e$  and  $\hat{\epsilon}_{ij}^e \hat{\epsilon}_{ij}^e$  are identical to Eqs. (5.22) and (5.30), respectively. Thus, the third-order coefficients  $(\hat{\epsilon}_{ii}^e \hat{\epsilon}_{kk}^e)_3$  and  $(\hat{\epsilon}_{ij}^e \hat{\epsilon}_{ij}^e)_3$  are obtained by applying Eq. (5.63) to Eqs. (5.23) and (5.31). This yields,

$$(\hat{\epsilon}_{ii}^e \hat{\epsilon}_{kk}^e)_3 = \frac{(d_c)^2}{2A_0^2} \left( \mathcal{J}^{(1)} + \mathcal{J}^{(2)} \right), \quad (5.64)$$

$$(\hat{\epsilon}_{ij}^e \hat{\epsilon}_{ij}^e)_3 = \frac{(d_c)^2}{4A_0^2} \left( 3\mathcal{J}^{(1)} + \mathcal{J}^{(2)} \right), \quad (5.65)$$

where  $\mathcal{J}^{(1)}$  and  $\mathcal{J}^{(2)}$  are the two integrals that needed to be evaluated explicitly,

$$\mathcal{J}^{(1)} = A_0 \left( e^{\frac{\tilde{Y}^{\text{IS}}}{8\pi}} \int_{a_{\text{dpl}}}^R \frac{dq}{a_{\text{dpl}}} \left( \frac{q}{a_{\text{dpl}}} \right)^{3 - \frac{\tilde{Y}^{\text{IS}}}{4\pi}} \right) \left( e^{\frac{\tilde{Y}^{\text{IS}}}{16\pi}} \int_{a_{\text{dpl}}}^{r_{\text{max}}} \frac{dq'}{a_{\text{dpl}}} \left( \frac{q'}{a_{\text{dpl}}} \right)^{1 - \frac{\tilde{Y}^{\text{IS}}}{8\pi}} \right)$$

$$\times \left( \int_0^{2\pi} d\psi \int_0^{2\pi} d\theta \int_0^{2\pi} d\theta' e^{\frac{\tilde{Y}^{\text{IS}}}{8\pi} (\cos(2\theta' - 2\psi) - \cos(2\theta - 2\psi))} \right), \quad (5.66)$$

$$\begin{aligned} \mathcal{J}^{(2)} = A_0 & \left( e^{\frac{\tilde{Y}^{\text{IS}}}{8\pi}} \int_{a_{\text{dpl}}}^R \frac{dq}{a_{\text{dpl}}} \left( \frac{q}{a_{\text{dpl}}} \right)^{3 - \frac{\tilde{Y}^{\text{IS}}}{4\pi}} \right) \left( e^{\frac{\tilde{Y}^{\text{IS}}}{16\pi}} \int_{a_{\text{dpl}}}^{r_{\text{max}}} \frac{dq'}{a_{\text{dpl}}} \left( \frac{q'}{a_{\text{dpl}}} \right)^{1 - \frac{\tilde{Y}^{\text{IS}}}{8\pi}} \right) \\ & \times \left( \int_0^{2\pi} d\psi \int_0^{2\pi} d\theta \int_0^{2\pi} d\theta' \cos(2\theta - 2\psi) e^{\frac{\tilde{Y}^{\text{IS}}}{8\pi} (\cos(2\theta' - 2\psi) - \cos(2\theta - 2\psi))} \right). \end{aligned} \quad (5.67)$$

To simplify the expressions in Eqs. (5.67) and (5.69), we first re-write the angular integral in Eq. (5.66) via the following Bessel function identity:

$$\left( \int_0^{2\pi} d\psi \int_0^{2\pi} d\theta \int_0^{2\pi} d\theta' e^{\frac{\tilde{Y}^{\text{IS}}}{8\pi} (\cos(2\theta' - 2\psi) - \cos(2\theta - 2\psi))} \right) = (2\pi)^3 I_0 \left( \frac{\tilde{Y}^{\text{IS}}}{8\pi} \right) I_0 \left( \frac{\tilde{Y}^{\text{IS}}}{8\pi} \right). \quad (5.68)$$

Thus, Eq. (5.66) becomes

$$\begin{aligned} \mathcal{J}^{(1)} = A_0 & \left( 2\pi^2 e^{\frac{\tilde{Y}^{\text{IS}}}{8\pi}} I_0 \left( \frac{\tilde{Y}^{\text{IS}}}{8\pi} \right) \int_{a_{\text{dpl}}}^R \frac{dq}{a_{\text{dpl}}} \left( \frac{q}{a_{\text{dpl}}} \right)^{3 - \frac{\tilde{Y}^{\text{IS}}}{4\pi}} \right) \\ & \times \left( 4\pi e^{\frac{\tilde{Y}^{\text{IS}}}{16\pi}} I_0 \left( \frac{\tilde{Y}^{\text{IS}}}{8\pi} \right) \int_{a_{\text{dpl}}}^{r_{\text{max}}} \frac{dq'}{a_{\text{dpl}}} \left( \frac{q'}{a_{\text{dpl}}} \right)^{1 - \frac{\tilde{Y}^{\text{IS}}}{8\pi}} \right). \end{aligned} \quad (5.69)$$

If we compare Eq. (5.69) with the corresponding integral  $\mathcal{P}^{(1)}$  found at second-order (Eq. (5.39)), we see that  $\mathcal{J}^{(1)}$  can be expressed as  $\mathcal{P}^{(1)}$  times a factor arising from the composite dipole's internal DOFs, i.e.,

$$\mathcal{J}^{(1)} = \mathcal{P}^{(1)} \left( 4\pi e^{\frac{\tilde{Y}^{\text{IS}}}{16\pi}} I_0 \left( \frac{\tilde{Y}^{\text{IS}}}{8\pi} \right) \int_{a_{\text{dpl}}}^{r_{\text{max}}} \frac{dq'}{a_{\text{dpl}}} \left( \frac{q'}{a_{\text{dpl}}} \right)^{1 - \frac{\tilde{Y}^{\text{IS}}}{8\pi}} \right). \quad (5.70)$$

This result is unique to the composite-dipole approximation, and it also generalizes to Eq. (5.67). To see this, we first simplify the angular integral in Eq. (5.67) using the following Bessel function identity:

$$\int_0^{2\pi} d\psi \int_0^{2\pi} d\theta \int_0^{2\pi} d\theta' \cos(2\theta - 2\psi) e^{\frac{\tilde{Y}^{\text{IS}}}{8\pi} (\cos(2\theta' - 2\psi) - \cos(2\theta - 2\psi))} = -(2\pi)^3 I_1 \left( \frac{\tilde{Y}^{\text{IS}}}{8\pi} \right) I_0 \left( \frac{\tilde{Y}^{\text{IS}}}{8\pi} \right), \quad (5.71)$$

which reduces Eq. (5.67) to

$$\begin{aligned} \mathcal{J}^{(2)} = A_0 & \left( -2\pi^2 e^{\frac{\tilde{Y}^{\text{IS}}}{8\pi}} I_1 \left( \frac{\tilde{Y}^{\text{IS}}}{8\pi} \right) \int_{a_{\text{dpl}}}^R \frac{dq}{a_{\text{dpl}}} \left( \frac{q}{a_{\text{dpl}}} \right)^{3 - \frac{\tilde{Y}^{\text{IS}}}{4\pi}} \right) \\ & \times \left( 4\pi e^{\frac{\tilde{Y}^{\text{IS}}}{16\pi}} I_0 \left( \frac{\tilde{Y}^{\text{IS}}}{8\pi} \right) \int_{a_{\text{dpl}}}^{r_{\text{max}}} \frac{dq'}{a_{\text{dpl}}} \left( \frac{q'}{a_{\text{dpl}}} \right)^{1 - \frac{\tilde{Y}^{\text{IS}}}{8\pi}} \right). \end{aligned} \quad (5.72)$$

If we compare Eq. (5.72) with the one from the second-order perturbation theory Eq. (5.41), we also see that  $\mathcal{J}^{(2)}$  can be expressed as  $\mathcal{P}^{(2)}$  times a factor arising from the composite dipole's internal DOFs:

$$\mathcal{J}^{(2)} = \mathcal{P}^{(2)} \left( 4\pi \tilde{y} e^{\frac{\tilde{Y}^{\text{IS}}}{16\pi}} I_0 \left( \frac{\tilde{Y}^{\text{IS}}}{8\pi} \right) \int_{a_{\text{dpl}}}^{r_{\text{max}}} \frac{dq'}{a_{\text{dpl}}} \left( \frac{q'}{a_{\text{dpl}}} \right)^{1 - \frac{\tilde{Y}^{\text{IS}}}{8\pi}} \right). \quad (5.73)$$

Equations (5.64), (5.65), (5.70) and (5.73) constitute the final results of the third-order perturbation theory.

### Summary of Fugacity Expansion

Using Eqs. (5.39), (5.41), (5.70) and (5.73), the fugacity expansion for the ensemble averages  $\langle \hat{\epsilon}_{ii}^e \hat{\epsilon}_{kk}^e \rangle$  and  $\langle \hat{\epsilon}_{ij}^e \hat{\epsilon}_{ij}^e \rangle$  can be written as

$$\langle \hat{\epsilon}_{ii}^e \hat{\epsilon}_{kk}^e \rangle = \frac{(d_c \tilde{y})^2}{2A_0^2} \left( \mathcal{P}^{(1)} + \mathcal{P}^{(2)} \right) \left( 1 + 4\pi \tilde{y} e^{\frac{\tilde{Y}^{\text{IS}}}{16\pi}} I_0 \left( \frac{\tilde{Y}^{\text{IS}}}{8\pi} \right) \int_{a_{\text{dpl}}}^{r_{\text{max}}} \frac{dq'}{a_{\text{dpl}}} \left( \frac{q'}{a_{\text{dpl}}} \right)^{1 - \frac{\tilde{Y}^{\text{IS}}}{8\pi}} \right) + \mathcal{O}(\tilde{y}^4), \quad (5.74)$$

$$\langle \hat{\epsilon}_{ij}^e \hat{\epsilon}_{ij}^e \rangle = \frac{(d_c \tilde{y})^2}{4A_0^2} \left( 3\mathcal{P}^{(1)} + \mathcal{P}^{(2)} \right) \left( 1 + 4\pi \tilde{y} e^{\frac{\tilde{Y}^{\text{IS}}}{16\pi}} I_0 \left( \frac{\tilde{Y}^{\text{IS}}}{8\pi} \right) \int_{a_{\text{dpl}}}^{r_{\text{max}}} \frac{dq'}{a_{\text{dpl}}} \left( \frac{q'}{a_{\text{dpl}}} \right)^{1 - \frac{\tilde{Y}^{\text{IS}}}{8\pi}} \right) + \mathcal{O}(\tilde{y}^4). \quad (5.75)$$

Substituting Eqs. (5.74) and (5.75) into Eqs. (4.18)–(4.20), we obtain the following fugacity expansion up to third order of the renormalized elastic moduli:

$$\frac{1}{\tilde{B}^{\text{R}}} = \frac{1}{\tilde{B}^{\text{IS}}} + \frac{\tilde{y}^2}{2A_0} \left( \mathcal{P}^{(1)} + \mathcal{P}^{(2)} \right) \left( 1 + 4\pi \tilde{y} e^{\frac{\tilde{Y}^{\text{IS}}}{16\pi}} I_0 \left( \frac{\tilde{Y}^{\text{IS}}}{8\pi} \right) \int_{a_{\text{dpl}}}^{r_{\text{max}}} \frac{dq'}{a_{\text{dpl}}} \left( \frac{q'}{a_{\text{dpl}}} \right)^{1 - \frac{\tilde{Y}^{\text{IS}}}{8\pi}} \right) + \mathcal{O}(\tilde{y}^4), \quad (5.76)$$

$$\frac{1}{\tilde{G}^{\text{R}}} = \frac{1}{\tilde{G}^{\text{IS}}} + \frac{\tilde{y}^2}{2A_0} \mathcal{P}^{(1)} \left( 1 + 4\pi \tilde{y} e^{\frac{\tilde{Y}^{\text{IS}}}{16\pi}} I_0 \left( \frac{\tilde{Y}^{\text{IS}}}{8\pi} \right) \int_{a_{\text{dpl}}}^{r_{\text{max}}} \frac{dq'}{a_{\text{dpl}}} \left( \frac{q'}{a_{\text{dpl}}} \right)^{1 - \frac{\tilde{Y}^{\text{IS}}}{8\pi}} \right) + \mathcal{O}(\tilde{y}^4), \quad (5.77)$$

$$\frac{1}{\tilde{Y}^{\text{R}}} = \frac{1}{\tilde{Y}^{\text{IS}}} + \frac{\tilde{y}^2}{8A_0} \left( 2\mathcal{P}^{(1)} + \mathcal{P}^{(2)} \right) \left( 1 + 4\pi \tilde{y} e^{\frac{\tilde{Y}^{\text{IS}}}{16\pi}} I_0 \left( \frac{\tilde{Y}^{\text{IS}}}{8\pi} \right) \int_{a_{\text{dpl}}}^{r_{\text{max}}} \frac{dq'}{a_{\text{dpl}}} \left( \frac{q'}{a_{\text{dpl}}} \right)^{1 - \frac{\tilde{Y}^{\text{IS}}}{8\pi}} \right) + \mathcal{O}(\tilde{y}^4), \quad (5.78)$$

where  $\mathcal{P}^{(1)}$  and  $\mathcal{P}^{(2)}$  are given by Eqs. (5.39) and (5.41), respectively. Equations (5.76)–(5.78) can be used for deriving the RG equations, which we proceed to do below in Section 5.2.

## 5.2 Deriving the RG Equations

Until now, we construct the fugacity expansion at low orders as a first step in applying the perturbative RG method. The next step is to derive the RG equations by inspecting the integral responsible for the expansion's divergent behavior, i.e., Eq. (5.42). The goal here is to find the scale-invariant property embedded in the expansion, which can be used to build a self-consistent scale transformation of the elastic moduli. To begin, suppose that we rescale  $a_{\text{dpl}} \rightarrow ba_{\text{dpl}}$ , where  $b$  is a scaling factor. This turns Eq. (5.42) into

$$\mathcal{I} = \int_{a_{\text{dpl}}b}^R \frac{dq}{a_{\text{dpl}}b} \left( \frac{q}{a_{\text{dpl}}b} \right)^{3 - \frac{\tilde{Y}^{\text{IS}}}{4\pi}}. \quad (5.79)$$

The integral in Eq. (5.79) can be made self-similar to the original integral in Eq. (5.42) by rescaling the pair distance as

$$\tilde{q} = q/b, \quad (5.80)$$

which yields

$$\int_{a_{\text{dpl}}b}^R \frac{dq}{a_{\text{dpl}}} \left( \frac{q}{a_{\text{dpl}}} \right)^{3-\frac{\tilde{Y}^{\text{IS}}}{4\pi}} = b^{4-\frac{\tilde{Y}^{\text{IS}}}{4\pi}} \int_{a_{\text{dpl}}}^{\tilde{R}} \frac{d\tilde{q}}{a_{\text{dpl}}} \left( \frac{\tilde{q}}{a_{\text{dpl}}} \right)^{3-\frac{\tilde{Y}^{\text{IS}}}{4\pi}}, \quad (5.81)$$

where  $\tilde{R} = R/b$ . Comparing Eq. (5.81) with Eq. (5.42), we see that the integration at lengthscales  $a_{\text{dpl}} < \tilde{q} < \tilde{R}$  is self-similar to the one at lengthscales  $a_{\text{dpl}} < q < R$ . In the limit of  $R \rightarrow \infty$ , Eq. (5.81) implies that the integral  $\mathcal{I} = \mathcal{I}(a_{\text{dpl}})$  transforms as

$$\mathcal{I}(ba_{\text{dpl}}) = b^{4-\frac{\tilde{Y}^{\text{IS}}}{4\pi}} \mathcal{I}(a_{\text{dpl}}). \quad (5.82)$$

Eq. (5.82) defines the scale-invariance property of the integral, and thereby the fugacity expansion of the elastic moduli. If  $\tilde{Y}^{\text{IS}} = 16\pi$ , which is the onset of divergence for the integral, then the rescaling factor vanishes. Such point indicates the onset of critical phenomena, since fluctuation corrections from lengthscales  $q > a_{\text{dpl}}$  are equal, without rescaling factors, to fluctuation corrections from the larger scales  $q > ba_{\text{dpl}}$ , given any choice of  $b > 1$ .

The scale-invariant property in Eq. (5.82) is now used to construct the RG equations via the following procedure:

1. *Choosing a Renormalization Condition:* As applied to our problem, a renormalization condition ensures that the RG flow preserves the dipole-pair picture of the physics at all lengthscales. By choosing an appropriate renormalization condition, we obtain a formula that defines a renormalized fugacity parameter  $\tilde{y}_R$ . Thus, one constructs RG flow not just on the space of elastic moduli, but also on the fugacity parameter.
2. *Splitting and Rescaling:* Next, we derive recursion relations governing the scale transformation of elastic moduli and fugacity, via a splitting-and-rescaling procedure. The splitting step splits the integrals entering Eqs. (5.76)–(5.78) into two parts: the first part integrates shorter-scale fluctuations around  $a_{\text{dpl}} < q < a_{\text{dpl}}e^{\delta\ell}$ , where  $\delta\ell$  is a small change in scale, and the second part integrates larger-scale fluctuations around  $a_{\text{dpl}}e^{\delta\ell} < q < R$ . The rescaling step transforms the pair distance  $q \rightarrow qe^{\delta\ell}$ , i.e., the same rescaling step in Eq. (5.80).

This procedure results in new terms entering Eqs. (5.76)–(5.78), such as new short-distance integrals and a multiplicative rescaling factor  $e^{\delta\ell(4-\frac{\tilde{Y}^{\text{IS}}}{4\pi})}$ . Using a similar renormalization condition to the one established in step one, we can uniquely define a set of scale-dependent elastic moduli  $\tilde{G}(\delta\ell)$ ,  $\tilde{B}(\delta\ell)$ , and  $\tilde{Y}(\delta\ell)$ , as well as fugacity  $\tilde{y}(\delta\ell)$  by absorbing the new terms appropriately into the bare parameters. Thus, the renormalization condition ensures that the scale-invariant property of Eq. (5.82) is embedded in the definition for the scale-dependent parameters, while preserving the dipole-pair picture of the physics.

3. *Linearizing the Recursion Relations:* Finally, we derive the RG equations governing infinitesimally small scale transformations of the elastic moduli and fugacity by linearizing the recursion relations from step two. This step has the geometric interpretation of constructing a tangent line for the RG flow around  $\ell$ . The slope of these tangent lines defines the ordinary differential equation (ODE) that we call the RG equation.

By following these three steps, the final RG flow describes the renormalization of elastic moduli due to the incorporation of dipole-pair fluctuations separated at increasingly larger lengthscales. These three steps are now outlined in the next three subsections.

### Step One: Choosing a Renormalization Condition

To begin, note that the structure of the expansion in Eqs. (5.76)–(5.78) resembles the second-order expansion, which can be written as

$$\frac{1}{\tilde{B}^{\text{R}}} = \frac{1}{\tilde{B}^{\text{IS}}} + \frac{\tilde{y}^2}{2A_0} \left( \mathcal{P}^{(1)} + \mathcal{P}^{(2)} \right) + \mathcal{O}(\tilde{y}^3), \quad (5.83)$$

$$\frac{1}{\tilde{G}^{\text{R}}} = \frac{1}{\tilde{G}^{\text{IS}}} + \frac{\tilde{y}^2}{2A_0} \mathcal{P}^{(1)} + \mathcal{O}(\tilde{y}^3), \quad (5.84)$$

$$\frac{1}{\tilde{Y}^{\text{R}}} = \frac{1}{\tilde{Y}^{\text{IS}}} + \frac{\tilde{y}^2}{8A_0} \left( 2\mathcal{P}^{(1)} + \mathcal{P}^{(2)} \right) + \mathcal{O}(\tilde{y}^3), \quad (5.85)$$

with the only difference being a multiplying factor

$$\left( 1 + 4\pi\tilde{y}e^{\frac{\tilde{Y}^{\text{IS}}}{16\pi}} I_0 \left( \frac{\tilde{Y}^{\text{IS}}}{8\pi} \right) \int_{a_{\text{dpl}}}^{r_{\text{max}}} \frac{dq'}{a_{\text{dpl}}} \left( \frac{q'}{a_{\text{dpl}}} \right)^{1-\frac{\tilde{Y}^{\text{IS}}}{8\pi}} \right) \quad (5.86)$$

that arises from the composite-dipole approximation. This observation leads to a renormalization condition that preserves the single dipole-pair picture of the problem; any  $m$ -th order fugacity expansion of the moduli ( $m = 3$  for Eqs. (5.76)–(5.78)) is to be written (in the composite-dipole approximation) as an effective second-order expansion, i.e.,

$$\frac{1}{\tilde{B}^{\text{R}}} = \frac{1}{\tilde{B}^{\text{IS}}} + \frac{(\tilde{y}_{\text{R}})^2}{2A_0} \left( \mathcal{P}^{(1)} + \mathcal{P}^{(2)} \right) + \mathcal{O}(\tilde{y}^{m+1}), \quad (5.87)$$

$$\frac{1}{\tilde{G}^{\text{R}}} = \frac{1}{\tilde{G}^{\text{IS}}} + \frac{(\tilde{y}_{\text{R}})^2}{2A_0} \left( \mathcal{P}^{(1)} \right) + \mathcal{O}(\tilde{y}^{m+1}), \quad (5.88)$$

$$\frac{1}{\tilde{Y}^{\text{R}}} = \frac{1}{\tilde{Y}^{\text{IS}}} + \frac{(\tilde{y}_{\text{R}})^2}{8A_0} \left( 2\mathcal{P}^{(1)} + \mathcal{P}^{(2)} \right) + \mathcal{O}(\tilde{y}^{m+1}), \quad (5.89)$$

where  $\tilde{y}_{\text{R}}$  is a renormalized fugacity parameter. The fact that fugacity is also renormalized implies that the phase space of the RG flow is now extended to include fugacity parameter.

The conditions set by Eqs. (5.87) and (5.89) imply the following renormalization of the fugacity parameter at the third order of the perturbation theory:

$$\tilde{y}_{\text{R}} := \tilde{y} \sqrt{1 + 4\pi\tilde{y}e^{\frac{\tilde{Y}^{\text{IS}}}{16\pi}} I_0 \left( \frac{\tilde{Y}^{\text{IS}}}{8\pi} \right) \int_{a_{\text{dpl}}}^{r_{\text{max}}} \frac{dq'}{a_{\text{dpl}}} \left( \frac{q'}{a_{\text{dpl}}} \right)^{1-\frac{\tilde{Y}^{\text{IS}}}{8\pi}}}, \quad (5.90)$$

which can be simplified upon further use of the series expansion of  $\sqrt{1+x}$ :

$$\tilde{y}_{\text{R}} = \tilde{y} + 2\pi\tilde{y}^2e^{\frac{\tilde{Y}^{\text{IS}}}{16\pi}} I_0 \left( \frac{\tilde{Y}^{\text{IS}}}{8\pi} \right) \int_{a_{\text{dpl}}}^{r_{\text{max}}} \frac{dq'}{a_{\text{dpl}}} \left( \frac{q'}{a_{\text{dpl}}} \right)^{1-\frac{\tilde{Y}^{\text{IS}}}{8\pi}} + \mathcal{O}(\tilde{y}^3), \quad (5.91)$$

providing a perturbative expansion for the renormalized fugacity, that arises purely as a consequence of satisfying the renormalization condition.

Substituting the formulas for the integrals  $\mathcal{P}^{(1)}$  (Eq. (5.39)) and  $\mathcal{P}^{(2)}$  (Eq. (5.41)) as well as Eq. (5.91) into Eqs. (5.76)–(5.78), we obtain the following formulas for the renormalized elastic moduli:

$$\frac{1}{\tilde{B}^{\text{R}}} = \frac{1}{\tilde{B}^{\text{IS}}} + (\tilde{y}_{\text{R}})^2 \pi^2 e^{\frac{\tilde{Y}^{\text{IS}}}{8\pi}} \left( I_0 \left( \frac{\tilde{Y}^{\text{IS}}}{8\pi} \right) - I_1 \left( \frac{\tilde{Y}^{\text{IS}}}{8\pi} \right) \right) \int_{a_{\text{dpl}}}^R \frac{dq}{a_{\text{dpl}}} \left( \frac{q}{a_{\text{dpl}}} \right)^{3-\frac{\tilde{Y}^{\text{IS}}}{4\pi}} + \mathcal{O}(\tilde{y}^4), \quad (5.92)$$

$$\frac{1}{\tilde{G}^R} = \frac{1}{\tilde{G}^{IS}} + (\tilde{y}_R)^2 \pi^2 e^{\frac{\tilde{Y}^{IS}}{8\pi}} I_0 \left( \frac{\tilde{Y}^{IS}}{8\pi} \right) \int_{a_{\text{dpl}}}^R \frac{dq}{a_{\text{dpl}}} \left( \frac{q}{a_{\text{dpl}}} \right)^{3-\frac{\tilde{Y}^{IS}}{4\pi}} + \mathcal{O}(\tilde{y}^4), \quad (5.93)$$

$$\frac{1}{\tilde{Y}^R} = \frac{1}{\tilde{Y}^{IS}} + \frac{1}{4} (\tilde{y}_R)^2 \pi^2 e^{\frac{\tilde{Y}^{IS}}{8\pi}} \left( 2I_0 \left( \frac{\tilde{Y}^{IS}}{8\pi} \right) - I_1 \left( \frac{\tilde{Y}^{IS}}{8\pi} \right) \right) \int_{a_{\text{dpl}}}^R \frac{dq}{a_{\text{dpl}}} \left( \frac{q}{a_{\text{dpl}}} \right)^{3-\frac{\tilde{Y}^{IS}}{4\pi}} + \mathcal{O}(\tilde{y}^4). \quad (5.94)$$

The form of Eqs. (5.92)–(5.94) establishes a linear proportionality between the (inverse) elastic moduli and the integral that exhibits the scale-invariance property. This is useful for the splitting-and-rescaling procedure in step two, where we further use the renormalization condition to prescribe formulas for the scale-dependent renormalized parameters.

### Step Two: Splitting and Rescaling

The procedure for deriving recursion relations of the elastic moduli and fugacity is done by first splitting the integrals in Eqs. (5.92)–(5.94) into two parts:

$$\int_{a_{\text{dpl}}}^R \frac{dq}{a_{\text{dpl}}} \left( \frac{q}{a_{\text{dpl}}} \right)^{3-\frac{\tilde{Y}^{IS}}{4\pi}} = \int_{a_{\text{dpl}}}^{a_{\text{dpl}}e^{\delta\ell}} \frac{dq}{a_{\text{dpl}}} \left( \frac{q}{a_{\text{dpl}}} \right)^{3-\frac{\tilde{Y}^{IS}}{4\pi}} + \int_{a_{\text{dpl}}e^{\delta\ell}}^R \frac{dq}{a_{\text{dpl}}} \left( \frac{q}{a_{\text{dpl}}} \right)^{3-\frac{\tilde{Y}^{IS}}{4\pi}}, \quad (5.95)$$

where  $\delta\ell$  sets a small perturbation in lengthscales away from  $a_{\text{dpl}}$ . Equation (5.95) can be substituted into Eqs. (5.92)–(5.94) to yield

$$\frac{1}{\tilde{B}^R} = \frac{1}{\tilde{B}(\delta\ell)} + \pi^2 (\tilde{y}_R)^2 e^{\frac{\tilde{Y}^{IS}}{8\pi}} \left( I_0 \left( \frac{\tilde{Y}^{IS}}{8\pi} \right) - I_1 \left( \frac{\tilde{Y}^{IS}}{8\pi} \right) \right) \int_{a_{\text{dpl}}e^{\delta\ell}}^R \frac{dq}{a_{\text{dpl}}} \left( \frac{q}{a_{\text{dpl}}} \right)^{3-\frac{\tilde{Y}^{IS}}{4\pi}} + \mathcal{O}(\tilde{y}^4), \quad (5.96)$$

$$\frac{1}{\tilde{G}^R} = \frac{1}{\tilde{G}(\delta\ell)} + \pi^2 (\tilde{y}_R)^2 e^{\frac{\tilde{Y}^{IS}}{8\pi}} I_0 \left( \frac{\tilde{Y}^{IS}}{8\pi} \right) \int_{a_{\text{dpl}}e^{\delta\ell}}^R \frac{dq}{a_{\text{dpl}}} \left( \frac{q}{a_{\text{dpl}}} \right)^{3-\frac{\tilde{Y}^{IS}}{4\pi}} + \mathcal{O}(\tilde{y}^4), \quad (5.97)$$

$$\frac{1}{\tilde{Y}^R} = \frac{1}{\tilde{Y}(\delta\ell)} + \frac{\pi^2}{4} (\tilde{y}_R)^2 e^{\frac{\tilde{Y}^{IS}}{8\pi}} \left( 2I_0 \left( \frac{\tilde{Y}^{IS}}{8\pi} \right) - I_1 \left( \frac{\tilde{Y}^{IS}}{8\pi} \right) \right) \int_{a_{\text{dpl}}e^{\delta\ell}}^R \frac{dq}{a_{\text{dpl}}} \left( \frac{q}{a_{\text{dpl}}} \right)^{3-\frac{\tilde{Y}^{IS}}{4\pi}} + \mathcal{O}(\tilde{y}^4), \quad (5.98)$$

where  $\tilde{B}(\delta\ell)$ ,  $\tilde{G}(\delta\ell)$ , and  $\tilde{Y}(\delta\ell)$  are the new scale-dependent elastic moduli obtained by absorbing the integration of shorter-scale fluctuations,

$$\frac{1}{\tilde{B}(\delta\ell)} = \frac{1}{\tilde{B}^{IS}} + \pi^2 (\tilde{y}_R)^2 e^{\frac{\tilde{Y}^{IS}}{8\pi}} \left( I_0 \left( \frac{\tilde{Y}^{IS}}{8\pi} \right) - I_1 \left( \frac{\tilde{Y}^{IS}}{8\pi} \right) \right) \int_{a_{\text{dpl}}}^{a_{\text{dpl}}e^{\delta\ell}} \frac{dq}{a_{\text{dpl}}} \left( \frac{q}{a_{\text{dpl}}} \right)^{3-\frac{\tilde{Y}^{IS}}{4\pi}}, \quad (5.99)$$

$$\frac{1}{\tilde{G}(\delta\ell)} = \frac{1}{\tilde{G}^{IS}} + \pi^2 (\tilde{y}_R)^2 e^{\frac{\tilde{Y}^{IS}}{8\pi}} I_0 \left( \frac{\tilde{Y}^{IS}}{8\pi} \right) \int_{a_{\text{dpl}}}^{a_{\text{dpl}}e^{\delta\ell}} \frac{dq}{a_{\text{dpl}}} \left( \frac{q}{a_{\text{dpl}}} \right)^{3-\frac{\tilde{Y}^{IS}}{4\pi}}, \quad (5.100)$$

$$\frac{1}{\tilde{Y}(\delta\ell)} = \frac{1}{\tilde{Y}^{IS}} + \frac{\pi^2}{4} (\tilde{y}_R)^2 e^{\frac{\tilde{Y}^{IS}}{8\pi}} \left( 2I_0 \left( \frac{\tilde{Y}^{IS}}{8\pi} \right) - I_1 \left( \frac{\tilde{Y}^{IS}}{8\pi} \right) \right) \int_{a_{\text{dpl}}}^{a_{\text{dpl}}e^{\delta\ell}} \frac{dq}{a_{\text{dpl}}} \left( \frac{q}{a_{\text{dpl}}} \right)^{3-\frac{\tilde{Y}^{IS}}{4\pi}}. \quad (5.101)$$

To obtain the corresponding scale-dependent formulas for  $\tilde{y}_R$ , recall that there is an upper cutoff  $r_{\text{max}}$  that we need to choose that sets the maximum separation distance between the two dipoles making up the composite dipole. Following Ref. [8], we set  $r_{\text{max}} = a_{\text{dpl}}e^{\delta\ell}$  so that the integral entering  $\tilde{y}_R$  becomes

$$\int_{a_{\text{dpl}}}^{r_{\text{max}}} \frac{dq'}{a_{\text{dpl}}} \left( \frac{q'}{a_{\text{dpl}}} \right)^{1-\frac{\tilde{Y}^{IS}}{8\pi}} = \int_{a_{\text{dpl}}}^{a_{\text{dpl}}e^{\delta\ell}} \frac{dq'}{a_{\text{dpl}}} \left( \frac{q'}{a_{\text{dpl}}} \right)^{1-\frac{\tilde{Y}^{IS}}{8\pi}}. \quad (5.102)$$

This keeps the fluctuations for the separation distance at a small range of lengthscales, and thereby keeping the two dipoles as a composite one. Using Eq. (5.102), we find that

$$\tilde{y}_R(\delta\ell) = \tilde{y} \left( 1 + 2\pi\tilde{y}e^{\frac{\tilde{Y}^{\text{IS}}}{16\pi}} I_0\left(\frac{\tilde{Y}^{\text{IS}}}{8\pi}\right) \int_{a_{\text{dpl}}}^{a_{\text{dpl}}e^{\delta\ell}} \frac{dq'}{a_{\text{dpl}}} \left(\frac{q'}{a_{\text{dpl}}}\right)^{1-\frac{\tilde{Y}^{\text{IS}}}{8\pi}} \right) + \mathcal{O}(\tilde{y}^3). \quad (5.103)$$

The next step in this procedure is to rescale the spatial integral in Eqs. (5.96)–(5.98) by substitution of variables  $q = e^{\delta\ell}\tilde{q}$  so that

$$\int_{a_{\text{dpl}}e^{\delta\ell}}^R \frac{dq}{a_{\text{dpl}}} \left(\frac{q}{a_{\text{dpl}}}\right)^{3-\frac{\tilde{Y}^{\text{IS}}}{4\pi}} = e^{\delta\ell\left(4-\frac{\tilde{Y}^{\text{IS}}}{4\pi}\right)} \int_{a_{\text{dpl}}}^{\tilde{R}} \frac{d\tilde{q}}{a_{\text{dpl}}} \left(\frac{\tilde{q}}{a_{\text{dpl}}}\right)^{3-\frac{\tilde{Y}^{\text{IS}}}{4\pi}}, \quad (5.104)$$

where  $\tilde{R} = Re^{-\delta\ell}$  is the new system size. Using Eq. (5.104), Eqs. (5.96)–(5.98) can be written as

$$\frac{1}{\tilde{B}^{\text{R}}} = \frac{1}{\tilde{B}(\delta\ell)} + \pi^2 e^{\delta\ell\left(4-\frac{\tilde{Y}^{\text{IS}}}{4\pi}\right)} (\tilde{y}_R)^2 e^{\frac{\tilde{Y}^{\text{IS}}}{8\pi}} \left( I_0\left(\frac{\tilde{Y}^{\text{IS}}}{8\pi}\right) - I_1\left(\frac{\tilde{Y}^{\text{IS}}}{8\pi}\right) \right) \int_{a_{\text{dpl}}}^{\tilde{R}} \frac{d\tilde{q}}{a_{\text{dpl}}} \left(\frac{\tilde{q}}{a_{\text{dpl}}}\right)^{3-\frac{\tilde{Y}^{\text{IS}}}{4\pi}}, \quad (5.105)$$

$$\frac{1}{\tilde{G}^{\text{R}}} = \frac{1}{\tilde{G}(\delta\ell)} + \pi^2 e^{\delta\ell\left(4-\frac{\tilde{Y}^{\text{IS}}}{4\pi}\right)} (\tilde{y}_R)^2 e^{\frac{\tilde{Y}^{\text{IS}}}{8\pi}} I_0\left(\frac{\tilde{Y}^{\text{IS}}}{8\pi}\right) \int_{a_{\text{dpl}}}^{\tilde{R}} \frac{d\tilde{q}}{a_{\text{dpl}}} \left(\frac{\tilde{q}}{a_{\text{dpl}}}\right)^{3-\frac{\tilde{Y}^{\text{IS}}}{4\pi}}, \quad (5.106)$$

$$\frac{1}{\tilde{Y}^{\text{R}}} = \frac{1}{\tilde{Y}(\delta\ell)} + \frac{\pi^2}{4} e^{\delta\ell\left(4-\frac{\tilde{Y}^{\text{IS}}}{4\pi}\right)} (\tilde{y}_R)^2 e^{\frac{\tilde{Y}^{\text{IS}}}{8\pi}} \left( 2I_0\left(\frac{\tilde{Y}^{\text{IS}}}{8\pi}\right) - I_1\left(\frac{\tilde{Y}^{\text{IS}}}{8\pi}\right) \right) \int_{a_{\text{dpl}}}^{\tilde{R}} \frac{d\tilde{q}}{a_{\text{dpl}}} \left(\frac{\tilde{q}}{a_{\text{dpl}}}\right)^{3-\frac{\tilde{Y}^{\text{IS}}}{4\pi}}, \quad (5.107)$$

up to order  $\mathcal{O}(\tilde{y}^4)$ , where a factor  $e^{\delta\ell\left(4-\frac{\tilde{Y}^{\text{IS}}}{4\pi}\right)}$  is obtained that rescale the integration of fluctuations to larger lengthscales. To ensure that Eqs. (5.105)–(5.107) obeys a renormalization condition similar to Eqs. (5.87)–(5.89), we can absorb the multiplicative rescaling factor into Eq. (5.103), giving us

$$\tilde{y}(\delta\ell) := \tilde{y}_R(\delta\ell) e^{\delta\ell\left(2-\frac{\tilde{Y}^{\text{IS}}}{8\pi}\right)} \quad (5.108)$$

$$= e^{\delta\ell\left(2-\frac{\tilde{Y}^{\text{IS}}}{8\pi}\right)} \tilde{y} \left( 1 + 2\pi\tilde{y}e^{\frac{\tilde{Y}^{\text{IS}}}{16\pi}} I_0\left(\frac{\tilde{Y}^{\text{IS}}}{8\pi}\right) \int_{a_{\text{dpl}}}^{a_{\text{dpl}}e^{\delta\ell}} \frac{dq'}{a_{\text{dpl}}} \left(\frac{q'}{a_{\text{dpl}}}\right)^{1-\frac{\tilde{Y}^{\text{IS}}}{8\pi}} \right) + \mathcal{O}(\tilde{y}^3), \quad (5.109)$$

which turns Eqs. (5.105)–(5.107) into

$$\frac{1}{\tilde{B}^{\text{R}}} = \frac{1}{\tilde{B}(\delta\ell)} + \pi^2 (\tilde{y}(\delta\ell))^2 e^{\frac{\tilde{Y}^{\text{IS}}}{8\pi}} \left( I_0\left(\frac{\tilde{Y}^{\text{IS}}}{8\pi}\right) - I_1\left(\frac{\tilde{Y}^{\text{IS}}}{8\pi}\right) \right) \int_{a_{\text{dpl}}}^{\tilde{R}} \frac{d\tilde{q}}{a_{\text{dpl}}} \left(\frac{\tilde{q}}{a_{\text{dpl}}}\right)^{3-\frac{\tilde{Y}^{\text{IS}}}{4\pi}} + \mathcal{O}(\tilde{y}^4), \quad (5.110)$$

$$\frac{1}{\tilde{G}^{\text{R}}} = \frac{1}{\tilde{G}(\delta\ell)} + \pi^2 (\tilde{y}(\delta\ell))^2 e^{\frac{\tilde{Y}^{\text{IS}}}{8\pi}} I_0\left(\frac{\tilde{Y}^{\text{IS}}}{8\pi}\right) \int_{a_{\text{dpl}}}^{\tilde{R}} \frac{d\tilde{q}}{a_{\text{dpl}}} \left(\frac{\tilde{q}}{a_{\text{dpl}}}\right)^{3-\frac{\tilde{Y}^{\text{IS}}}{4\pi}} + \mathcal{O}(\tilde{y}^4), \quad (5.111)$$

$$\frac{1}{\tilde{Y}^{\text{R}}} = \frac{1}{\tilde{Y}(\delta\ell)} + \frac{\pi^2}{4} (\tilde{y}(\delta\ell))^2 e^{\frac{\tilde{Y}^{\text{IS}}}{8\pi}} \left( 2I_0\left(\frac{\tilde{Y}^{\text{IS}}}{8\pi}\right) - I_1\left(\frac{\tilde{Y}^{\text{IS}}}{8\pi}\right) \right) \int_{a_{\text{dpl}}}^{\tilde{R}} \frac{d\tilde{q}}{a_{\text{dpl}}} \left(\frac{\tilde{q}}{a_{\text{dpl}}}\right)^{3-\frac{\tilde{Y}^{\text{IS}}}{4\pi}} + \mathcal{O}(\tilde{y}^4). \quad (5.112)$$

Note that Eqs. (5.110)–(5.112) are identical in form to the ones in Eqs. (5.92)–(5.94), where we first applied the renormalization condition.

The process of splitting and rescaling can be repeated one more time to Eqs. (5.110)–(5.112). This yields a new set of scale-dependent elastic moduli:

$$\frac{1}{\tilde{B}(2\delta\ell)} = \frac{1}{\tilde{B}(\delta\ell)} + \pi^2 (\tilde{y}(\delta\ell))^2 e^{\frac{\tilde{Y}^{\text{IS}}}{8\pi}} \left( I_0\left(\frac{\tilde{Y}^{\text{IS}}}{8\pi}\right) - I_1\left(\frac{\tilde{Y}^{\text{IS}}}{8\pi}\right) \right) \int_{a_{\text{dpl}}}^{a_{\text{dpl}}e^{\delta\ell}} \frac{dq}{a_{\text{dpl}}} \left( \frac{q}{a_{\text{dpl}}} \right)^{3-\frac{\tilde{Y}^{\text{IS}}}{4\pi}}, \quad (5.113)$$

$$\frac{1}{\tilde{G}(2\delta\ell)} = \frac{1}{\tilde{G}(\delta\ell)} + \pi^2 (\tilde{y}(\delta\ell))^2 e^{\frac{\tilde{Y}^{\text{IS}}}{8\pi}} I_0\left(\frac{\tilde{Y}^{\text{IS}}}{8\pi}\right) \int_{a_{\text{dpl}}}^{a_{\text{dpl}}e^{\delta\ell}} \frac{dq}{a_{\text{dpl}}} \left( \frac{q}{a_{\text{dpl}}} \right)^{3-\frac{\tilde{Y}^{\text{IS}}}{4\pi}}, \quad (5.114)$$

$$\frac{1}{\tilde{Y}(2\delta\ell)} = \frac{1}{\tilde{Y}(\delta\ell)} + \frac{\pi^2}{4} (\tilde{y}(\delta\ell))^2 e^{\frac{\tilde{Y}^{\text{IS}}}{8\pi}} \left( 2I_0\left(\frac{\tilde{Y}^{\text{IS}}}{8\pi}\right) - I_1\left(\frac{\tilde{Y}^{\text{IS}}}{8\pi}\right) \right) \int_{a_{\text{dpl}}}^{a_{\text{dpl}}e^{\delta\ell}} \frac{dq}{a_{\text{dpl}}} \left( \frac{q}{a_{\text{dpl}}} \right)^{3-\frac{\tilde{Y}^{\text{IS}}}{4\pi}}, \quad (5.115)$$

where the corresponding formula for the new scale-dependent fugacity is

$$\tilde{y}(2\delta\ell) = \tilde{y}e^{(2\delta\ell)(2-\frac{\tilde{Y}^{\text{IS}}}{8\pi})} \left( 1 + 2\pi\tilde{y}e^{\frac{\tilde{Y}^{\text{IS}}}{16\pi}} I_0\left(\frac{\tilde{Y}^{\text{IS}}}{8\pi}\right) \int_{a_{\text{dpl}}}^{a_{\text{dpl}}e^{\delta\ell}} \frac{dq'}{a_{\text{dpl}}} \left( \frac{q'}{a_{\text{dpl}}} \right)^{1-\frac{\tilde{Y}^{\text{IS}}}{8\pi}} \right) + \mathcal{O}(\tilde{y}^3). \quad (5.116)$$

Unlike the first iteration, these new elastic moduli and fugacity are not solely dependent on their corresponding values at  $\delta\ell$ ; the initial bare parameters from  $\delta\ell = 0$  such as  $Y^{\text{IS}}$  still enter Eqs. (5.113)–(5.116).

To obtain appropriate recursion relations, we may replace the bare Young's modulus  $Y^{\text{IS}}$  and fugacity  $\tilde{y}$  entering Eqs. (5.113)–(5.116) with their scale-dependent versions,  $\tilde{Y}(\delta\ell)$  and  $\tilde{y}(\delta\ell)$ . This replacement is achieved by noting from Eqs. (5.99)–(5.101) that

$$\frac{1}{\tilde{B}(\delta\ell)} = \frac{1}{\tilde{B}^{\text{IS}}} + \mathcal{O}(\tilde{y}(\delta\ell))^2, \quad \frac{1}{\tilde{G}(\delta\ell)} = \frac{1}{\tilde{G}^{\text{IS}}} + \mathcal{O}(\tilde{y}(\delta\ell))^2, \quad \frac{1}{\tilde{Y}(\delta\ell)} = \frac{1}{\tilde{Y}^{\text{IS}}} + \mathcal{O}(\tilde{y}(\delta\ell))^2, \quad (5.117)$$

and also noting from Eq. (5.109) that

$$\tilde{y}(\delta\ell) = \tilde{y} + \mathcal{O}(\delta\ell). \quad (5.118)$$

Furthermore, from Eq. (5.117), we see that the Bessel and exponential functions can be written as

$$I_0\left(\frac{\tilde{Y}^{\text{IS}}}{8\pi}\right) = I_0\left(\frac{\tilde{Y}(\delta\ell)}{8\pi}\right) + \mathcal{O}(\tilde{y}(\delta\ell)^2), \quad e^{\frac{\tilde{Y}^{\text{IS}}}{16\pi}} = e^{\frac{\tilde{Y}(\delta\ell)}{16\pi}} + \mathcal{O}(\tilde{y}(\delta\ell)^2). \quad (5.119)$$

Substituting Eqs. (5.118) and (5.119) into Eqs. (5.113)–(5.116) yields

$$\frac{1}{\tilde{B}(2\delta\ell)} = \frac{1}{\tilde{B}(\delta\ell)} + \pi^2 (\tilde{y}(\delta\ell))^2 e^{\frac{\tilde{Y}(\delta\ell)}{8\pi}} \left( I_0\left(\frac{\tilde{Y}(\delta\ell)}{8\pi}\right) - I_1\left(\frac{\tilde{Y}(\delta\ell)}{8\pi}\right) \right) \int_{a_{\text{dpl}}}^{a_{\text{dpl}}e^{\delta\ell}} \frac{dq}{a_{\text{dpl}}} \left( \frac{q}{a_{\text{dpl}}} \right)^{3-\frac{\tilde{Y}(\delta\ell)}{4\pi}}, \quad (5.120)$$

$$\frac{1}{\tilde{G}(2\delta\ell)} = \frac{1}{\tilde{G}(\delta\ell)} + \pi^2 (\tilde{y}(\delta\ell))^2 e^{\frac{\tilde{Y}(\delta\ell)}{8\pi}} I_0\left(\frac{\tilde{Y}(\delta\ell)}{8\pi}\right) \int_{a_{\text{dpl}}}^{a_{\text{dpl}}e^{\delta\ell}} \frac{dq}{a_{\text{dpl}}} \left( \frac{q}{a_{\text{dpl}}} \right)^{3-\frac{\tilde{Y}(\delta\ell)}{4\pi}}, \quad (5.121)$$

$$\frac{1}{\tilde{Y}(2\delta\ell)} = \frac{1}{\tilde{Y}(\delta\ell)} + \frac{\pi^2}{4} (\tilde{y}(\delta\ell))^2 e^{\frac{\tilde{Y}(\delta\ell)}{8\pi}} \left( 2I_0\left(\frac{\tilde{Y}(\delta\ell)}{8\pi}\right) - I_1\left(\frac{\tilde{Y}(\delta\ell)}{8\pi}\right) \right) \int_{a_{\text{dpl}}}^{a_{\text{dpl}}e^{\delta\ell}} \frac{dq}{a_{\text{dpl}}} \left( \frac{q}{a_{\text{dpl}}} \right)^{3-\frac{\tilde{Y}(\delta\ell)}{4\pi}}, \quad (5.122)$$

up to order  $\mathcal{O}(\tilde{y}(\delta\ell)^4)$  and

$$\tilde{y}(2\delta\ell) = \tilde{y}(\delta\ell) e^{(2\delta\ell)\left(2 - \frac{\tilde{Y}(\delta\ell)}{8\pi}\right)} \left( 1 + 2\pi\tilde{y}(\delta\ell) e^{\frac{\tilde{Y}(\delta\ell)}{16\pi}} I_0\left(\frac{\tilde{Y}(\delta\ell)}{8\pi}\right) \int_{a_{\text{dpl}}}^{a_{\text{dpl}}e^{\delta\ell}} \frac{dq}{a_{\text{dpl}}} \left(\frac{q}{a_{\text{dpl}}}\right)^{1 - \frac{\tilde{Y}(\delta\ell)}{8\pi}} \right), \quad (5.123)$$

up to order  $\mathcal{O}(\tilde{y}(\delta\ell)^3)$ .

Repeating the splitting-and-integral procedure  $m$  many times, we build a more general set of recursion relations, where elastic moduli and fugacity at a scale  $(m+1)\delta\ell := \ell + \delta\ell$  are self-generated from the ones at the smaller scale  $\ell := m\delta\ell$ . The final set of recursion relations up to order  $\mathcal{O}(\tilde{y}(\ell)^4)$  for the elastic moduli can be derived as follows:

$$\frac{1}{\tilde{B}(\ell + \delta\ell)} = \frac{1}{\tilde{B}(\ell)} + \pi^2 (\tilde{y}(\ell))^2 e^{\frac{\tilde{Y}(\ell)}{8\pi}} \left( I_0\left(\frac{\tilde{Y}(\ell)}{8\pi}\right) - I_1\left(\frac{\tilde{Y}(\ell)}{8\pi}\right) \right) \int_{a_{\text{dpl}}}^{a_{\text{dpl}}e^{\delta\ell}} \frac{dq}{a_{\text{dpl}}} \left(\frac{q}{a_{\text{dpl}}}\right)^{3 - \frac{\tilde{Y}(\ell)}{4\pi}}, \quad (5.124)$$

$$\frac{1}{\tilde{G}(\ell + \delta\ell)} = \frac{1}{\tilde{G}(\ell)} + \pi^2 (\tilde{y}(\ell))^2 e^{\frac{\tilde{Y}(\ell)}{8\pi}} I_0\left(\frac{\tilde{Y}(\ell)}{8\pi}\right) \int_{a_{\text{dpl}}}^{a_{\text{dpl}}e^{\delta\ell}} \frac{dq}{a_{\text{dpl}}} \left(\frac{q}{a_{\text{dpl}}}\right)^{3 - \frac{\tilde{Y}(\ell)}{4\pi}}, \quad (5.125)$$

$$\frac{1}{\tilde{Y}(\ell + \delta\ell)} = \frac{1}{\tilde{Y}(\ell)} + \frac{\pi^2}{4} (\tilde{y}(\ell))^2 e^{\frac{\tilde{Y}(\ell)}{8\pi}} \left( 2I_0\left(\frac{\tilde{Y}(\ell)}{8\pi}\right) - I_1\left(\frac{\tilde{Y}(\ell)}{8\pi}\right) \right) \int_{a_{\text{dpl}}}^{a_{\text{dpl}}e^{\delta\ell}} \frac{dq}{a_{\text{dpl}}} \left(\frac{q}{a_{\text{dpl}}}\right)^{3 - \frac{\tilde{Y}(\ell)}{4\pi}}, \quad (5.126)$$

and the fugacity recursion relation up to order  $\mathcal{O}(\tilde{y}(\ell)^3)$  is

$$\tilde{y}(\ell + \delta\ell) = \tilde{y}(\ell) e^{(\ell + \delta\ell)\left(2 - \frac{\tilde{Y}(\ell)}{8\pi}\right)} \left( 1 + 2\pi\tilde{y}(\ell) e^{\frac{\tilde{Y}(\ell)}{16\pi}} I_0\left(\frac{\tilde{Y}(\ell)}{8\pi}\right) \int_{a_{\text{dpl}}}^{a_{\text{dpl}}e^{\delta\ell}} \frac{dq}{a_{\text{dpl}}} \left(\frac{q}{a_{\text{dpl}}}\right)^{1 - \frac{\tilde{Y}(\ell)}{8\pi}} \right). \quad (5.127)$$

Equations (5.124)–(5.127) form the basis of the RG equations, which can be viewed as a differential form of these recursion relations. Note that the recursion relations for the bulk and shear modulus are driven by the fugacity and Young's modulus only. This implies that the phase space of the final RG flow is two-dimensional and is spanned by  $\tilde{Y}^{-1}$  and  $\tilde{y}$ .

### Step Three: Linearization of Recursion Relations

We are now interested in how the elastic moduli and fugacities change under infinitesimal transformation in scale  $\delta\ell$ . Specializing to the fugacity and Young's modulus, we note that under infinitesimal change in  $\delta\ell$ , it should be possible add fluctuation corrections to  $\tilde{y}(\ell)$  and  $\tilde{Y}^{-1}(\ell)$  as follows:

$$\tilde{y}(\ell + \delta\ell) = \tilde{y}(\ell) + \frac{d\tilde{y}(\ell)}{d\ell} \delta\ell + \mathcal{O}(\delta\ell^2), \quad (5.128)$$

$$\frac{1}{\tilde{Y}(\ell + \delta\ell)} = \frac{1}{\tilde{Y}(\ell)} + \frac{d\tilde{Y}^{-1}(\ell)}{d\ell} \delta\ell + \mathcal{O}(\delta\ell^2). \quad (5.129)$$

As illustrated in Fig. S.17, Eqs. (5.128) and (5.129) can be geometrically interpreted as the tangent lines for the RG flow up to scale  $\ell$ , where the flow is reconstructed when we piece these tangent lines into a curve.

Equations (5.128) and (5.129) can be obtained by linearizing the recursion relations in Eqs. (5.124)–(5.127), and we can use the slope as the ODE that generates the RG flow. For instance, Taylor

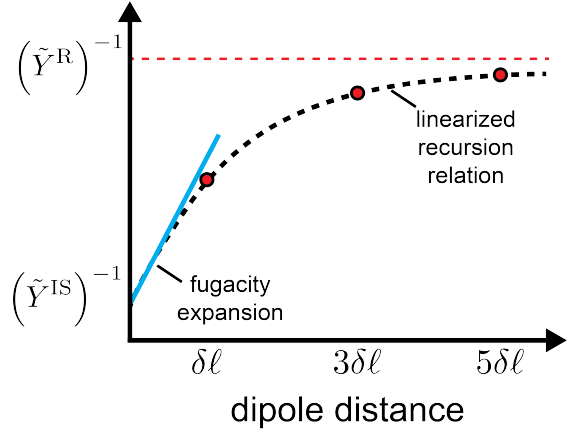

Figure S.17: An illustration of the RG flow for the inverse Young's modulus as a geometric (re)construction via a series of linearized recursion relations (dashed grey). The tangent line at  $\delta\ell = 0$  (blue line) coincides with the linearized version of the original fugacity expansion, i.e., Eq. (5.78).

expanding the fugacity recursion relation in Eq. (5.127) around  $\delta\ell = 0$  yields

$$\frac{d\tilde{y}(\ell)}{d\ell} = \left(2 - \frac{\tilde{Y}(\ell)}{8\pi}\right) \tilde{y}(\ell) + 2\pi (\tilde{y}(\ell))^2 e^{\frac{\tilde{Y}(\ell)}{16\pi}} I_0\left(\frac{\tilde{Y}(\ell)}{8\pi}\right) + \mathcal{O}(\tilde{y}(\ell)^3), \quad \tilde{y}(0) = \tilde{y}, \quad (5.130)$$

which is precisely the RG equation for the fugacity and  $\tilde{y}(0)$  being the initial datum of the flow.

The RG equations for the elastic moduli can also be derived in a similar fashion, where Taylor expansion of Eqs. (5.124)–(5.126) around  $\delta\ell = 0$  yields

$$\frac{d\tilde{B}^{-1}(\ell)}{d\ell} = \pi^2 (\tilde{y}(\ell))^2 e^{\frac{\tilde{Y}(\ell)}{8\pi}} \left( I_0\left(\frac{\tilde{Y}(\ell)}{8\pi}\right) - I_1\left(\frac{\tilde{Y}(\ell)}{8\pi}\right) \right) + \mathcal{O}(\tilde{y}(\ell)^3), \quad \tilde{B}(0) = \tilde{B}^{\text{IS}}, \quad (5.131)$$

$$\frac{d\tilde{G}^{-1}(\ell)}{d\ell} = \pi^2 (\tilde{y}(\ell))^2 e^{\frac{\tilde{Y}(\ell)}{8\pi}} I_0\left(\frac{\tilde{Y}(\ell)}{8\pi}\right) + \mathcal{O}(\tilde{y}(\ell)^3), \quad \tilde{G}(0) = \tilde{G}^{\text{IS}}, \quad (5.132)$$

$$\frac{d\tilde{Y}^{-1}(\ell)}{d\ell} = \frac{\pi^2}{4} (\tilde{y}(\ell))^2 e^{\frac{\tilde{Y}(\ell)}{8\pi}} \left( 2I_0\left(\frac{\tilde{Y}(\ell)}{8\pi}\right) - I_1\left(\frac{\tilde{Y}(\ell)}{8\pi}\right) \right) + \mathcal{O}(\tilde{y}(\ell)^3), \quad \tilde{Y}(0) = \tilde{Y}^{\text{IS}}. \quad (5.133)$$

Given these RG equations the final renormalized values of the elastic moduli and fugacity are obtained from the large-scale limit of the RG flow,

$$\tilde{B}_{\text{R}} = \lim_{\ell \rightarrow \infty} \tilde{B}(\ell), \quad \tilde{G}_{\text{R}} = \lim_{\ell \rightarrow \infty} \tilde{G}(\ell), \quad \tilde{Y}_{\text{R}} = \lim_{\ell \rightarrow \infty} \tilde{Y}(\ell), \quad \tilde{y}_{\text{R}} = \lim_{\ell \rightarrow \infty} \tilde{y}(\ell). \quad (5.134)$$

From Eqs. (5.130)–(5.133), we see that the bulk and shear modulus are driven solely by Young's modulus and fugacity. Thus, Eqs. (5.130) and (5.133) provide a sufficient description for the RG flow.

At this stage we provide one last remark before moving on to the analysis of the RG flow. If the recursion relations are linearized at  $\ell = 0$  (the shortest lengthscale), then the slopes are given by

$$\left. \frac{d\tilde{y}(\ell)}{d\ell} \right|_{\ell=0} = \left(2 - \frac{\tilde{Y}^{\text{IS}}}{8\pi}\right) \tilde{y} + 2\pi \tilde{y}^2 e^{\frac{\tilde{Y}^{\text{IS}}}{16\pi}} I_0\left(\frac{\tilde{Y}^{\text{IS}}}{8\pi}\right) + \mathcal{O}(\tilde{y}^3), \quad (5.135)$$

$$\left. \frac{d\tilde{B}^{-1}(\ell)}{d\ell} \right|_{\ell=0} = \pi^2 \tilde{y}^2 e^{\frac{\tilde{Y}^{\text{IS}}}{8\pi}} \left( I_0\left(\frac{\tilde{Y}^{\text{IS}}}{8\pi}\right) - I_1\left(\frac{\tilde{Y}^{\text{IS}}}{8\pi}\right) \right) + \mathcal{O}(\tilde{y}^3), \quad (5.136)$$

$$\left. \frac{d\tilde{G}^{-1}(\ell)}{d\ell} \right|_{\ell=0} = \pi^2 \tilde{y}^2 e^{\frac{\tilde{Y}^{\text{IS}}}{8\pi}} I_0\left(\frac{\tilde{Y}^{\text{IS}}}{8\pi}\right) + \mathcal{O}(\tilde{y}^3), \quad (5.137)$$

$$\left. \frac{d\tilde{Y}^{-1}(\ell)}{d\ell} \right|_{\ell=0} = \frac{\pi^2}{4} \tilde{y}^2 e^{\frac{\tilde{Y}^{\text{IS}}}{8\pi}} \left( 2I_0\left(\frac{\tilde{Y}^{\text{IS}}}{8\pi}\right) - I_1\left(\frac{\tilde{Y}^{\text{IS}}}{8\pi}\right) \right) + \mathcal{O}(\tilde{y}^3). \quad (5.138)$$

One may verify that the RHS of these expressions can be obtained from linearizing the original fugacity expansion in Eqs. (5.76)–(5.78) for the elastic moduli, and the expansion in Eq. (5.109) for the fugacity parameter. <sup>\*</sup> This result provides additional insight into how the perturbative RG method works; even though the initial expansion is divergent upon integrating to macroscopic lengthscales, its linearization at the smallest lengthscales may be used as a perturbative approximation to the true RG flow. To ensure correct extrapolation to larger scales, scale-invariance is incorporated to this linearized flow through appropriate renormalization of the fugacity parameter, e.g., absorption of the multiplicative rescaling factor  $b^{4-\frac{\tilde{Y}^{\text{IS}}}{4\pi}}$  into  $\tilde{y}_R$ . This is what then allows us to take the initial slope of the linearized flow as an infinitesimal generator of the full RG flow, and integrate the generator to obtain fluctuation corrections in a scale-invariant manner. <sup>||</sup>

### 5.3 Analysis of the RG Equations

Having derived the RG equations in Section 5.2 we analyze the RG flow to obtain an understanding of the global macroscopic behavior of the system. To this end, let  $\hat{Y} = \frac{\tilde{Y}}{8\pi}$  and  $w(x) = e^x (I_0(x) - I_1(x)/2)/2$ . The RG equations in Eqs. (5.130) and (5.133) can now be written as

$$\frac{d\tilde{y}}{d\ell} = (2 - \hat{Y}) \tilde{y} + 2\pi \tilde{y}^2 e^{\hat{Y}/2} I_0(\hat{Y}), \quad (5.139a)$$

$$\frac{d\hat{Y}^{-1}}{d\ell} = 8\pi^3 \tilde{y}^2 w(\hat{Y}). \quad (5.139b)$$

The location of the fixed points  $(y^*, \hat{Y}^*)$  are obtained by setting the derivatives in Eqs. (5.139a) and (5.139b) to zero:

$$0 = (2 - \hat{Y}^*) \tilde{y}^* + 2\pi (\tilde{y}^*)^2 e^{\hat{Y}^*/2} I_0(\hat{Y}^*), \quad (5.140a)$$

$$0 = 8\pi^3 (\tilde{y}^*)^2 w(\hat{Y}^*). \quad (5.140b)$$

Note that by setting  $\tilde{y}^* = 0$ , we can satisfy Eqs. (5.140a) and (5.140b) regardless of the value of  $\hat{Y}^*$ , implying that the entire set of all possible  $\hat{Y}^*$  at  $\tilde{y}^* = 0$  is a set of fixed points of the flow. Using linear stability analysis, we also find that

$$\frac{d\delta\tilde{y}}{d\ell} = (2 - \hat{Y}^*) \delta\tilde{y} + \mathcal{O}((\delta\tilde{y}\delta\hat{Y})), \quad (5.141a)$$

$$\frac{d\delta\hat{Y}}{d\ell} = \mathcal{O}((\delta\tilde{y}^2)). \quad (5.141b)$$

---

<sup>\*</sup>This can be seen by replacing the system size  $R \rightarrow a_{\text{dpl}} e^{\delta\ell}$  and the upper cutoff  $r_{\text{max}} \rightarrow a_{\text{dpl}} e^{\delta\ell}$ , and Taylor expanding the resulting integral around  $\delta\ell = 0$ .

<sup>||</sup>The rigorous justification for these arguments is based on the group-theory aspect of RG; it explains why standard textbook procedure on field-theoretic perturbative RG [35, 36] may skip the step of developing a full set of recursion relations like in Eqs. (5.124)–(5.127), and proceed directly with the linearization of the perturbative expansion (after applying the renormalization condition).

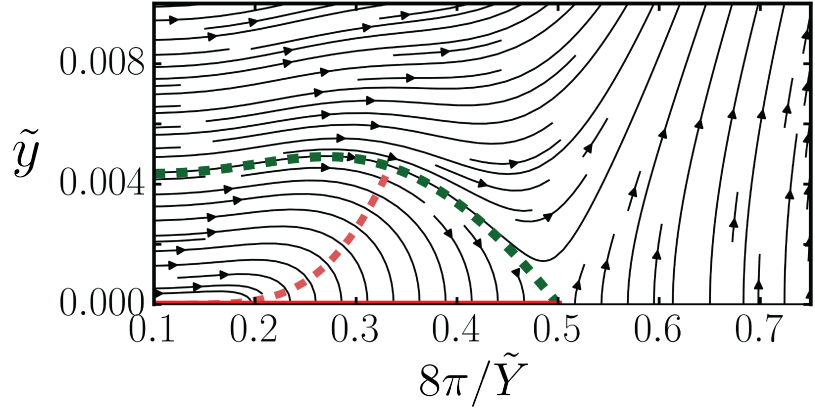

Figure S.18: Phase-space portrait of the RG equations in Eqs. (5.139a) and (5.139b). Horizontal red line corresponds to a line of fixed points terminating at the critical point of  $\tilde{Y} = 16\pi$ . Green dashed line is the separatrix line, delineating the low-temperature supercooled liquid from the high-temperature liquid. Red dashed line is the possible initial conditions for the RG flow.

where  $\delta\tilde{y} = \tilde{y} - \tilde{y}^*$  and  $\delta\tilde{Y} = \tilde{Y} - \tilde{Y}^*$ . Thus, there exists a special value of the dimensionless Young's modulus

$$\hat{Y}_{\text{KT}} = 2 \rightarrow \tilde{Y}_{\text{KT}} = 16\pi \quad (5.142)$$

above which the fixed points become stable (since  $\frac{d\delta\tilde{y}}{d\ell} < 0$ ), and below which they become unstable (since  $\frac{d\delta\tilde{y}}{d\ell} > 0$ ). This result is also confirmed in the phase portrait of Eqs. (5.139a) and (5.139b) provided in Fig. S.18.

The critical value in Eq. (5.142) defines the melting point of the system. To see this, we note from the phase portrait that there exists a separatrix curve (green dashed line, Fig. S.18) where the flow converges to  $(\tilde{y}_R, \tilde{Y}_R) = (0, 16\pi)$ . Initial conditions below the separatrix define a region where the flow converges towards the set of stable fixed points. The full renormalized values  $(\tilde{y}_R, \tilde{Y}_R) = (0, \tilde{Y}^*)$  indicate a system that behaves like a solid with no defects, and thus this region defines the supercooled state of the glass former. Above the separatrix, the flow converges to  $(\tilde{y}_R, \tilde{Y}_R) = (\infty, 0)$  indicating the fluid phase, or equivalently the high-temperature liquid state of the glass former. Thus, the separatrix outlines the fluid-solid phase boundary, and the intersection of the initial-condition curve with the separatrix defines the melting point  $T_{\text{KT}}$  for a given system.

The initial conditions needed for determining the melting point  $T_{\text{KT}}$  are already defined in Section 3.4; the bare fugacity and dimensionless Young's modulus can be written in terms of the original dimensional variables as,

$$\tilde{y} = e^{-\beta\bar{E}_c}, \quad E_c = \frac{1}{4}(7 + \nu^{\text{IS}})\Delta F^\ddagger, \quad \tilde{Y}^{\text{IS}} = \beta d_c^2 Y^{\text{IS}}, \quad d_c = \frac{2\pi R_{\text{exc}}\epsilon_c}{\nu^{\text{IS}} + 1}. \quad (5.143)$$

where  $\Delta F^\ddagger$  is given in Eq. (3.53), and  $R_{\text{exc}}$  and  $\epsilon_c$  are given in Eq. (3.47). Since all bare parameters are a function of temperature  $T$ , the initial conditions defined by Eq. (5.143) outlines a curve  $(\tilde{y}(T), \tilde{Y}(T))$  parametrized by  $T$ , as shown in Fig. S.18. The non-linearity of the RG equations may prohibit a closed-form solution for the intersection of the initial-condition curve and separatrix, but it can still be computed via a shooting method. This method locates the melting point  $T_{\text{KT}}$  by iteratively finding the initial condition that takes the numerical integration of the RG equations to a value of  $\tilde{Y}(\ell_f) \approx 16\pi$  for a sufficiently large final scale  $\ell_f$ . The values of  $T_{\text{KT}}$  reported in Table 1 of the main text are obtained in this manner, with  $\ell_f \approx 200$ .

Having explored the nature of the fixed points, we are now ready to study the asymptotic solutions near the fixed points. Defining the perturbation in the inverse Young's modulus as  $x = 2\hat{Y}^{-1} - 1$ , we can linearize the Bessel and exponential functions entering Eqs. (5.139a) and (5.139b) and retain terms up to quadratic order in both  $x$  and  $y$  to obtain

$$\frac{dy}{d\ell} \simeq 2xy + 2\pi B y^2, \quad (5.144a)$$

$$\frac{dx}{d\ell} \simeq 16\pi^3 A y^2, \quad (5.144b)$$

where  $A = w(2) \simeq 5.48365$  and  $B = e^1 I_0(2) \simeq 6.19656$  are constants evaluated at the fixed point.

To study the critical behavior, we need the solutions for Eqs. (5.144a) and (5.144b) near the separatrix curve and close to the fixed point. An approximate separatrix may be found in the form of a straight line  $y = mx$  when analyzing the flow near the fixed point. Differentiating this with respect to  $x$ , we obtain the condition that defines the separatrix

$$\frac{dy}{dx} = m. \quad (5.145)$$

Substituting the linear separatrix equation in Eq. (5.144a) we find

$$\frac{dy}{d\ell} \simeq 2mx^2 + 2\pi B m^2 x^2 \quad (5.146)$$

and dividing with Eq. (5.144b) we obtain

$$\frac{dy}{dx} = \frac{1 + \pi B m}{8\pi^3 A m}. \quad (5.147)$$

Comparing Eq. (5.145) with Eq. (5.147), we obtain the following quadratic equation for  $m$

$$8A\pi^3 m^2 - B\pi m - 1 = 0, \quad (5.148)$$

which has the following roots

$$m_{\pm} = \frac{B \pm \sqrt{B^2 + 32A\pi}}{16A\pi^2}. \quad (5.149)$$

Since the separatrix that defines the solid-fluid phase boundary has a negative slope near the critical point, the relevant separatrix curve is the one defined by  $y(x) = m_- x$ .

To determine the scaling behavior of the elastic moduli at low temperatures, we first look for asymptotic solutions in  $y$  that is parametrized as a small perturbation near the separatrix, i.e.,

$$y(\ell) = m_- x(\ell) + \delta y(\ell), \quad (5.150)$$

where the perturbation around separatrix  $\delta y(\ell)$  is assumed to have an initial condition  $\delta y_0 = -c_0 |t|$  where  $|t| = \left| \frac{T - T_{KT}}{T_{KT}} \right|$  and  $c_0 > 0$  is an arbitrary constant. This restricts our analysis to the critical point. The differential equation for  $\delta y(\ell)$  is obtained by substituting Eqs. (5.150) and (5.144b) in Eq. (5.144a):

$$\frac{d\delta y(\ell)}{d\ell} = 2x(m_- x + \delta y) + (2\pi B - 16m_- \pi^3 A)(m_-^2 x^2 + 2m_- x \delta y + \mathcal{O}(\delta y^2)) \quad (5.151)$$

$$= -2x\delta y, \quad (5.152)$$

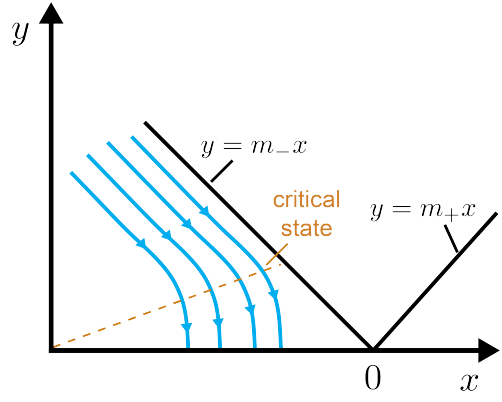

Figure S.19: An illustration of the RG flow near the separatrix. For every trajectory, there exists a turning point  $\ell^*$  where the slope  $\frac{dy}{dx}$  deviates away from the separatrix, and the flow sinks rapidly to one of the stable fixed points. This turning point  $\ell^*$  signals an intermediate lengthscale, below which (pre)critical fluctuations driven by excitations exist but above which fluctuations behave like those of a solid with little to no defects.

where the second equality is obtained by making use of Eq. (5.148) to remove any dependency in  $A$  and  $B$ . The solution to Eq. (5.152) is

$$\delta y(\ell) = -c_0|t| \exp\left(-2 \int_0^\ell x(\ell') d\ell'\right). \quad (5.153)$$

The formula in Eq. (5.150) can also be used to find the solution for  $x(\ell)$  by substituting Eq. (5.150) in Eq. (5.144b):

$$\frac{dx}{d\ell} \simeq 16\pi^3 Am_-^2 x^2 + \mathcal{O}(\delta y^2), \quad (5.154)$$

which leads to

$$x(\ell) = \frac{x_0}{1 - 16\pi^3 Am_-^2 x_0 \ell} = -\frac{|x_0|}{1 + 16\pi^3 Am_-^2 |x_0| \ell} \quad (5.155)$$

and  $x_0 < 0$  is some initial condition. Eq. (5.155) leads to the following closed-form solution for the perturbation in fugacity

$$\delta y(\ell) = -c_0|t| \exp\left(2 \int_0^\ell \frac{|x_0|}{1 + 16\pi^3 Am_-^2 |x_0| \ell'} d\ell'\right) = -c_0|t| (1 + 16\pi^3 Am_-^2 x_0 \ell)^{\frac{1}{8\pi^3 Am_-^2}}, \quad (5.156)$$

and thus the solution for the fugacity becomes

$$y(\ell) = \frac{|m_-||x_0|}{1 + 16\pi^3 Am_-^2 |x_0| \ell} - c_0|t| (1 + 16\pi^3 Am_-^2 |x_0| \ell)^{\frac{1}{8\pi^3 Am_-^2}}. \quad (5.157)$$

The scaling behavior from Eq. (5.157) can be deduced by noting that the RG flow follows the separatrix very closely before diverging away at  $\ell = \ell^*$ , and converging towards one of the stable fixed points; see Fig. S.19. This change in slope of the RG flow field can be defined by setting the first and second term in Eq. (5.144a) to be equal:

$$2xy = 2\pi B y^2 \rightarrow y(\ell^*) = \frac{x(\ell^*)}{B\pi} = -\frac{|x_0|}{B\pi (1 + 16\pi^3 Am_-^2 |x_0| \ell^*)} \quad (5.158)$$

at which point the  $y^2$  non-linearity is in the same order as the bilinear  $xy$  term, signaling a change in slope of any trajectory that passes through this turning point. This critical scale  $\ell^*$  corresponds to a critical lengthscale

$$\xi^* = a_{\text{dpl}} e^{\ell^*}, \quad (5.159)$$

where fluctuations from lengthscale  $a_{\text{dpl}}$  up to  $\xi^*$  are essentially critical or self-similar to the one at  $T = T_{\text{KT}}$ . The RG flow integrated up to this scale incorporates the dominant fluctuation corrections to the bare moduli, and thus approximates the full renormalized value at that temperature, i.e.,

$$\tilde{y}(\ell^*) \approx \tilde{y}_{\text{R}} \rightarrow 0, \quad \tilde{Y}(\ell^*) \approx \tilde{Y}_{\text{R}} \rightarrow 16\pi \quad \text{as } |t| \rightarrow 0, \quad (5.160)$$

or in terms of the small perturbation variables

$$x(\ell^*) \approx x_{\text{R}} \rightarrow 0 \quad \text{as } |t| \rightarrow 0, \quad (5.161)$$

where  $x_{\text{R}} = \lim_{\ell \rightarrow \infty} x(\ell)$ . Equation (5.160) also implies that fluctuations at lengthscales  $q > \xi^*$  resemble those of a solid with no defects since  $\tilde{y}(\ell) \approx 0$  for  $\ell > \ell^*$ ; an important property that will be used later in Section 5.5. Equating Eq. (5.157) with Eq. (5.158), we find

$$\frac{|x_0|}{(1 + 16\pi^3 A m_-^2 |x_0| \ell^*)} \left( \frac{1}{B\pi} + m_- \right) = c_0 |t| \left( 1 + 16\pi^3 A m_-^2 |x_0| \ell^* \right)^{\frac{1}{8\pi^3 A m_-^2}}. \quad (5.162)$$

Solving this equation for  $\ell^*$ , we obtain

$$\ell^* \approx C_1 |t|^{-\bar{\nu}_{\text{KT}}}, \quad \bar{\nu}_{\text{KT}} = \frac{1}{2} - \frac{B}{2\sqrt{B^2 + 32A\pi}} \simeq 0.372, \quad (5.163)$$

where  $\bar{\nu}_{\text{KT}}$  is a critical exponent and  $C_1 = \frac{\left( \frac{|x_0|}{B\pi x_0} - \frac{|x_0| m_-}{c_0} \right)^{\bar{\nu}_{\text{KT}}}}{16A m_-^2 \pi^3 |x_0|}$  is independent of temperature  $T$ . Equation (5.163) implies the following temperature dependence in the critical lengthscale

$$\xi^*(T) = a_{\text{dpl}} \exp \left( \frac{C_1}{|t|^{\bar{\nu}_{\text{KT}}}} \right), \quad (5.164)$$

which exhibits a singularity as  $|t| \rightarrow 0$ .

According to Eqs. (5.155) and (5.161), we also find that

$$x_{\text{R}} \approx -\frac{|x_0|}{1 + 16\pi^3 A m_-^2 |x_0| \ell^*} \approx -\frac{|x_0|}{16\pi^3 A m_-^2 |x_0| \ell^*} \approx -\bar{C} |t|^{\bar{\nu}_{\text{KT}}}, \quad (5.165)$$

where in the second equality we assume  $1 \ll 16\pi^3 A m_-^2 |x_0| \ell^*$ , and  $\bar{C} = \left( \frac{|x_0|}{B\pi x_0} - \frac{|x_0| m_-}{c_0} \right)^{\bar{\nu}_{\text{KT}}}$ . Thus, the inverse of the Young's modulus near the critical point scales as

$$\frac{1}{\tilde{Y}_{\text{R}}} \simeq \frac{1}{16\pi} (1 - \bar{C} |t|^{\bar{\nu}_{\text{KT}}}). \quad (5.166)$$

or equivalently

$$\tilde{Y}_{\text{R}} \simeq 16\pi (1 + \bar{C} |t|^{\bar{\nu}_{\text{KT}}}). \quad (5.167)$$

Similar statements can be made in regards to the other elastic moduli; the bulk and shear moduli are linearly proportional to the Young's modulus, up to a factor controlled by the renormalized Poisson's ratio  $\nu_{\text{R}}$ , and so their asymptotic behavior is given by

$$\tilde{B}_{\text{R}} \sim \tilde{G}_{\text{R}} \sim 16\pi (1 + \bar{C} |t|^{\bar{\nu}_{\text{KT}}}). \quad (5.168)$$

Table 2: List of poly-disperse models studied in this work. A model with repulsive-interaction exponent  $m$  and interactive-interaction  $n$  is named Poly- $(m, n)$ .

| Model       | $m$ | $n$ | $\varepsilon$ | $\tilde{r}_c$ |
|-------------|-----|-----|---------------|---------------|
| Poly-(12,0) | 12  | 0   | 0.2           | 1.25          |
| Poly-(12,6) | 12  | 6   | 0.2           | 2.5           |
| Poly-(18,0) | 18  | 0   | 0.0           | 1.25          |
|             | 18  | 0   | 0.2           | 1.25          |
| Poly-(10,6) | 10  | 6   | 0.1           | 2.5           |
|             | 10  | 6   | 0.2           | 2.5           |

Equations (5.163), (5.167) and (5.168) provide the most salient features of the system's asymptotic behavior near the critical point, and are the main results of this section.

At this stage, we make several remarks. First, the results we obtain so far are nearly identical to the KTHNY theory applied to 2D triangular-lattice crystals. There exists a slight difference in the value of the critical exponent  $\bar{\nu}_{\text{KT}}$ , which stems from the discrete nature of the dislocation orientation angle in the KTHNY theory. Second, the phase behavior at temperatures  $T < T_{\text{KT}}$  is governed by a line of stable fixed points; according to the general RG theory [35], the system should exhibit power-law spatial correlations in fluctuations. These power-law spatial correlations can be understood as the consequence of the two-dimensional nature of a linear elastic solid as we will show in Section 5.5.

#### 5.4 Atomistic Models of Glass Formers and RG Calculations of Elastic Moduli

The goal of the present section is to describe the procedure to obtain: (i) the onset temperature  $T_o$ , (ii) inherent-state elastic moduli, and (iii) the transition temperature  $T_{\text{KT}}$  as well as the renormalized elastic moduli from numerical integration of the RG flow equations Eqs. (5.139a) and (5.139b).

**Models:** We primarily test the theory on a class of continuous poly-disperse systems studied in [7, 39]. The general form of the pair potential in these models is given by

$$\phi(r/\sigma_{\alpha\beta}) = \begin{cases} v_0 \left[ \left( \frac{\sigma_{\alpha\beta}}{r} \right)^m - \left( \frac{\sigma_{\alpha\beta}}{r} \right)^n \right] + F(r/\sigma_{\alpha\beta}) & r/\sigma_{\alpha\beta} \leq \tilde{r}_c \\ 0 & \text{otherwise} \end{cases}, \quad (5.169)$$

$$\sigma_{\alpha\beta} = \frac{1}{2} (\sigma_\alpha + \sigma_\beta) (1 - \varepsilon |\sigma_\alpha - \sigma_\beta|), \quad (5.170)$$

where the function  $F(r) = c_0 + c_1 r^2 + c_2 r^4$  is an even polynomial that ensures continuity of the pair potential at  $r = \tilde{r}_c$  up to second-order derivative, and  $\varepsilon$  is the non-additive parameter that prevents crystallization and aggregation. The particle size distribution is defined by  $P(\sigma_d) = C/(\sigma_d)^3$  for  $\sigma_{\min} < \sigma_d < \sigma_{\max}$  and zero otherwise, where  $C$  is some normalizing constant. As listed in Table 2, we choose six poly-disperse systems by varying  $m$ ,  $n$ ,  $\varepsilon$ , and  $\tilde{r}_c$ . The rest of the model parameters are kept constant to the following values:  $v_0 = 1$ ,  $\sigma_{\min}$ ,  $\sigma_{\max}$  and  $C$  are chosen such that  $\langle \sigma_d \rangle = \int d\sigma_d P(\sigma_d) \sigma_d = 1$  and  $\sigma_{\min}/\sigma_{\max} = 0.45$ , mass is unity,  $k_B = 1$ , system size  $N = 32^2$ , and density  $\rho = 1.01$ .

**MD Simulations and Onset Temperature  $T_o$  Calculations:** For all model glass formers, we obtain relaxation-time data using molecular dynamics (MD) simulations in HOOMD-blue [40].

The MD simulation of poly-disperse glass formers was done via a custom plugin<sup>††</sup>, implemented in HOOMD-blue. First, we run 40 independent MD simulations under the NVT ensemble to equilibrate configurations and momenta. The Nosé-Hoover thermostat with timestep  $\Delta t = 0.0075$  and coupling constant  $\tau = \sqrt{\frac{Q}{gk_B T}} = 50\Delta t$ , where  $Q$  is the Nosé mass and  $g = dN$  is the number of degrees of freedom, is always used for running these simulations. Subsequent NVE production runs with time-step  $\Delta t = 0.0075$  were used to compute equilibrium relaxation time  $\tau_{\text{eq}}$  from the self-part of intermediate scattering function,

$$F_s(\mathbf{k}, t) = \frac{1}{N} \left\langle \sum_{\alpha=1}^N \exp(i\mathbf{k} \cdot [\mathbf{r}^\alpha(t) - \mathbf{r}^\alpha(0)]) \right\rangle. \quad (5.171)$$

The relaxation time  $\tau_{\text{eq}}$  is defined when the angle-averaged  $F_s(k, t) = \frac{1}{2\pi} \int_0^{2\pi} d\phi F_s(k, \phi, t)$ , where  $\mathbf{k} = k(\cos \phi, \sin \phi)$ , becomes equal to  $1/10$  for  $k = 2\pi/\langle \sigma_d \rangle$ . Note that the length of time and temperature range for both equilibration and production runs are set by the  $\tau_{\text{eq}}(T)$  data: (1) NVT equilibration is run up to  $20\tau_{\text{eq}}$  to  $25\tau_{\text{eq}}$ , (2) NVE production is run up to  $5\tau_{\text{eq}}$ , to ensure accurate time-averaged estimate of  $F_s(k, t) = 0.1$ , and (3) temperature range is set so that we have measured  $\tau_{\text{eq}}$  roughly from  $10^{-1}$  to  $10^4$  orders in magnitude relative to  $\tau_{\text{eq}}(T = T_o)$ , where  $T_o$  is the onset temperature.

The onset temperature  $T_o$  is then estimated from fitting the parabolic law,

$$\ln \left[ \frac{\tau_{\text{eq}}}{\tau_o} \right] = \begin{cases} J^2(\beta - \beta_o)^2 + (\beta - \beta_o)E_a & \beta \geq \beta_o \\ (\beta - \beta_o)E_a & \beta < \beta_o \end{cases}, \quad (5.172)$$

to the equilibrium relaxation time  $\tau_{\text{eq}}(T)$  data, where  $\beta_o = 1/k_B T_o$ ,  $E_a$  is the high-temperature activation energy,  $J$  is an effective energy scale, and  $\tau_o$  is the relaxation time at  $T = T_o$ . First, we fit the high-temperature data with the Arrhenius term, fixing the fitted Arrhenius parameters, and then we fit the low-temperature data with the parabolic law in Eq. (5.172). The high-temperature portion of the data is determined statistically, i.e., it is the number of high-temperature data points needed to maximize the  $R^2$  value of the low-temperature fitting.

**Inherent-State Elastic Moduli Calculation:** To determine the initial conditions, Eq. (5.143), of the RG flow equations in Eqs. (5.139a) and (5.139b), we require the calculation of the inherent-state elastic moduli at different temperatures. To this end, we first obtain equilibrated configurations  $\{\mathbf{r}_\alpha\}$  using SWAP Monte Carlo [39] at different temperatures  $T$  for all models of Table 2. From these configurations, the corresponding inherent-state configurations  $\{\mathbf{R}_\alpha\}$  are obtained via local-energy minimization, where the FIRE algorithm [41] is used with the maximum timestep at every  $i$ -th iteration set between  $\Delta t_i \in [0.05, 0.075]$ . An energy minimum is reached when  $\sum_{\alpha=1}^N |\mathbf{F}_\alpha|/N \leq 10^{-6}$  and  $|\Delta U|/N \leq 10^{-7}$ . From the inherent-state configurations, we compute the shear ( $G^{\text{IS}}$ ) and Young's ( $Y^{\text{IS}}$ ) moduli, respectively, through the stiffness tensor  $C_{ijkl}^{\text{IS}}$  [7, 42].

The computation of  $C_{ijkl}^{\text{IS}}$  requires the evaluation of the Born part  $C_{ijkl}^B$ , which involves pair-wise sums, and the non-affine part  $C_{ijkl}^{\text{NA}}$  that requires the pseudo-inverse  $\mathbf{H}^+$  of the Hessian  $\mathbf{H} = \frac{\partial^2 U}{\partial \mathbf{r} \partial \mathbf{r}}$  evaluated at the inherent-state configurations, where  $\mathbf{r}$  is the  $N$ -particles position vector. These calculations are performed by an in-house code<sup>††</sup> that utilizes SLEPc [43] for eigenvalue/vector calculations. Note that prior to ensemble averaging, the time-series of  $G^{\text{IS}}$  and  $Y^{\text{IS}}$  are de-correlated through a sub-sampling scheme in [44], which is already implemented in the Python package `pymbar`.

<sup>††</sup><https://github.com/mandadapu-group/polydisperse-md>

<sup>††</sup><https://github.com/mandadapu-group/pyglasstools>

Following this scheme, 8000 to 10000 uncorrelated samples are available for averaging at every temperature. The results of these calculations for the polydisperse glass formers can be found in Fig. S.11 of [7].

**Transition Temperature  $T_{\text{KT}}$  and Renormalized Elastic Moduli:** We test our theory by evaluating the transition temperature  $T_{\text{KT}}$  for which binding-unbinding transition of elastic dipolar excitations occurs and compare its value with the extracted onset temperature  $T_o$ . The analysis of the RG equations in Section 5.3 allows us to define  $T_{\text{KT}}$  as the temperature for which the initial conditions of Eqs. (5.139a) and (5.139b) flow to the stationary point  $(\tilde{y}^*, \tilde{Y}^*) = (0, 16\pi)$ . Schematically, this point corresponds to the temperature for which the initial conditions intersect the separatrix (green dashed line), as shown in Fig. S.18 for the Poly-(12,0) model glass former.

Practically, we identify  $T_{\text{KT}}$  by performing a temperature sweep across all values of the inherent-state elastic moduli for all glass-former models considered in the present study. In particular, after choosing a temperature, we evaluate the initial conditions of Eq. (5.143), and subsequently integrate numerically Eqs. (5.139a) and (5.139b) using implicit Euler with  $\Delta\ell = 0.02$ . We iterate this procedure until we identify the temperature for which the stationary point lies between  $(0, 16\pi - \delta\tilde{Y})$  and  $(0, 16\pi)$ , with  $\delta\tilde{Y} = 10^{-4}$ . The results of these calculations can be found in Table 1 of the main text, where reasonable agreement is found across all polydisperse glass formers.

In addition to the transition temperature, we are interested in the renormalized elastic moduli due to the existence of bound dipolar elastic excitations in the supercooled regime. Through the temperature sweep for determining  $T_{\text{KT}}$ , we are able to obtain the renormalized elastic constants  $Y^{\text{R}}$ ,  $G^{\text{R}}$  and  $\nu^{\text{R}}$ . The results for all models are shown in Figs. S.20–S.22, where for all glass-former models the elastic moduli  $G^{\text{R}}$  and  $Y^{\text{R}}$  converge to a finite value as  $T \rightarrow T_{\text{KT}}$  from below, and abruptly drops to zero at the melting transition.

## 5.5 Mean-Squared Displacement and Density–Density Correlations

The analysis of the RG equations shows that the system macroscopically behaves as an elastic solid ( $\tilde{Y}_{\text{R}} \neq 0$ ) with no defects ( $\tilde{y} = 0$ ) at  $T < T_{\text{KT}}$ . We may use this fact to model the total strain fluctuations  $\epsilon_{ij}$  via an effective Gaussian field theory of elastic fluctuations, where the partition function is given by

$$\bar{\mathcal{Z}}_{\text{eff}} = \int \mathcal{D}\mathbf{u} \, e^{-\beta\mathcal{H}_{\text{eff}}}, \quad \mathcal{H}_{\text{eff}} = \frac{1}{2} \int d^2\mathbf{x} \, \epsilon_{ij} C_{ijkl}^{\text{R}} \epsilon_{kl}. \quad (5.173)$$

This effective field theory is valid for a specific range of lengthscales set by  $\xi^*(T)$  found in the RG analysis, i.e., it is valid for displacement fluctuation modes with wavenumber  $|\mathbf{k}| \in [0, 2\pi/\xi^*]$ . Equation (5.173) is nearly identical to the partition function Eq. (4.1) for the ‘bare’ harmonic fluctuations with the chief difference being the elastic moduli, which correspond to their renormalized values in this effective field theory.

The Gaussian nature of the strain fluctuations has important consequences on the relaxation behavior of a supercooled liquid. To see this, we first note that renormalization plays a diminishing role as  $T \rightarrow 0$  since dipole pairs become more bounded and dilute. This can be seen, for instance, in the RG calculations shown in Fig. S.23, where the renormalized elastic moduli converge the bare inherent-state values the moment that  $T < T_p$ , where  $T_p$  is the temperature where the shear modulus begins to plateau at high temperatures [7]. At this deeply supercooled state, the critical lengthscale  $\xi^* \sim \mathcal{O}(a_{\text{dpl}})$  is very small and coincides with the lengthscale  $\mathcal{O}(\sigma_d) \sim \mathcal{O}(a_{\text{dpl}})$  in which we measure relaxation where  $\sigma_d$  is the particle diameter. Since the current theory models

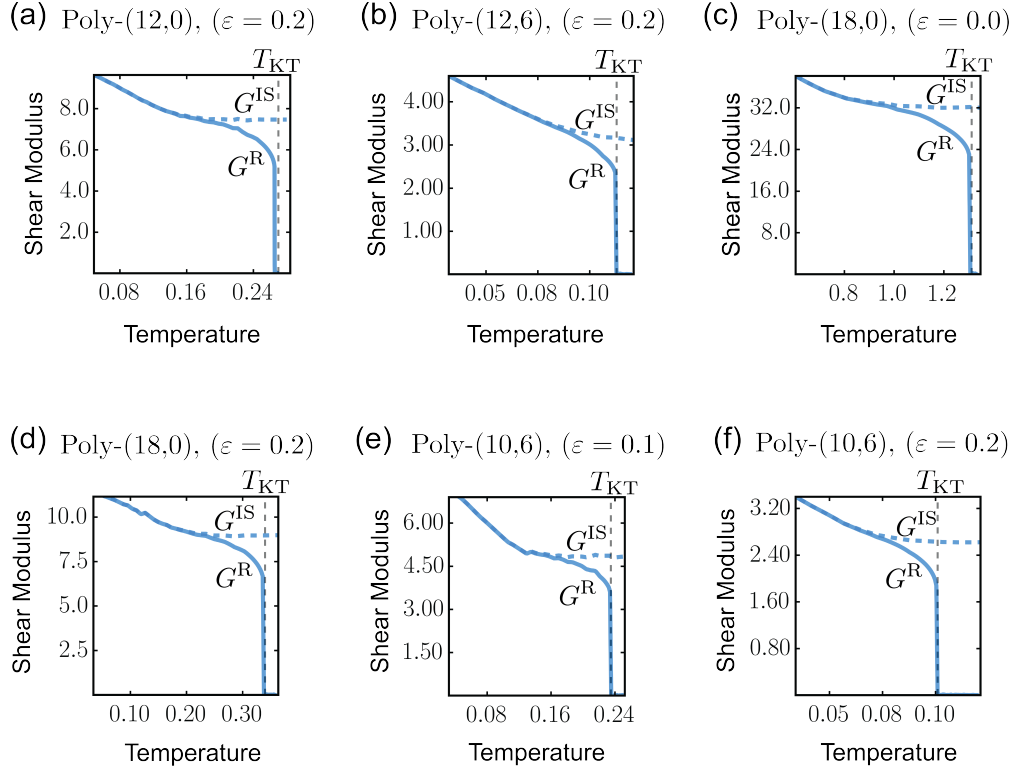

Figure S.20: The bare inherent-state shear modulus in comparison to the renormalized shear modulus for six model atomistic glass formers. Just below the onset temperature, excitations play an important role in renormalizing the bare shear modulus.

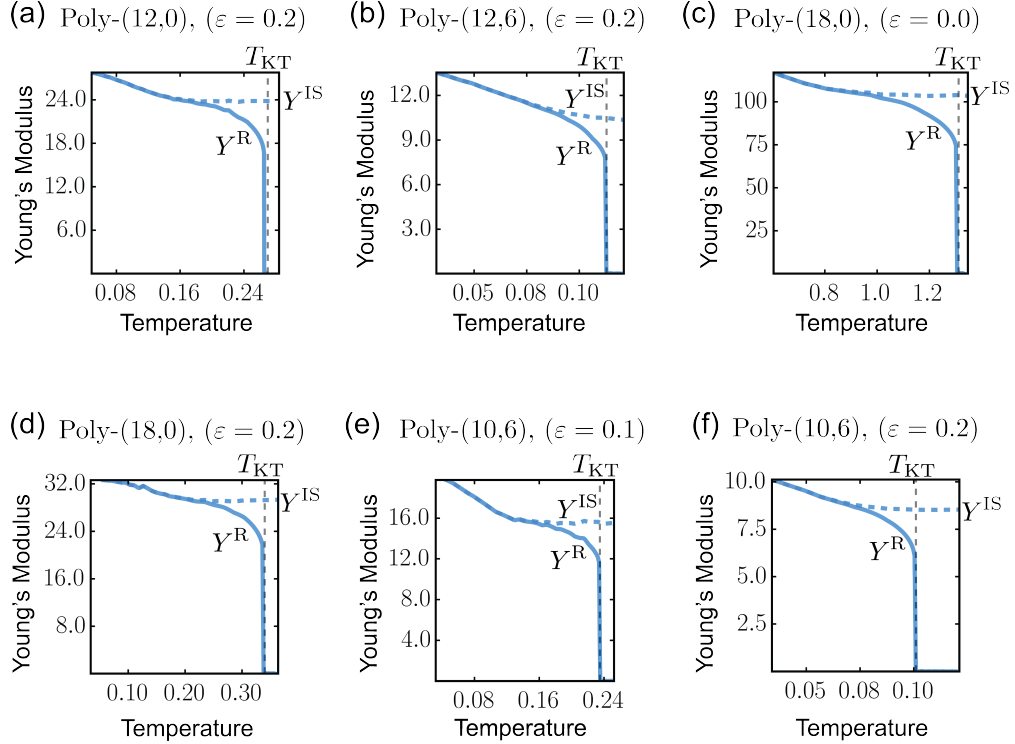

Figure S.21: The bare inherent-state Young's modulus in comparison to the renormalized Young's modulus for six model atomistic glass formers. Just below the onset temperature, excitations play an important role in renormalizing the bare Young's modulus.

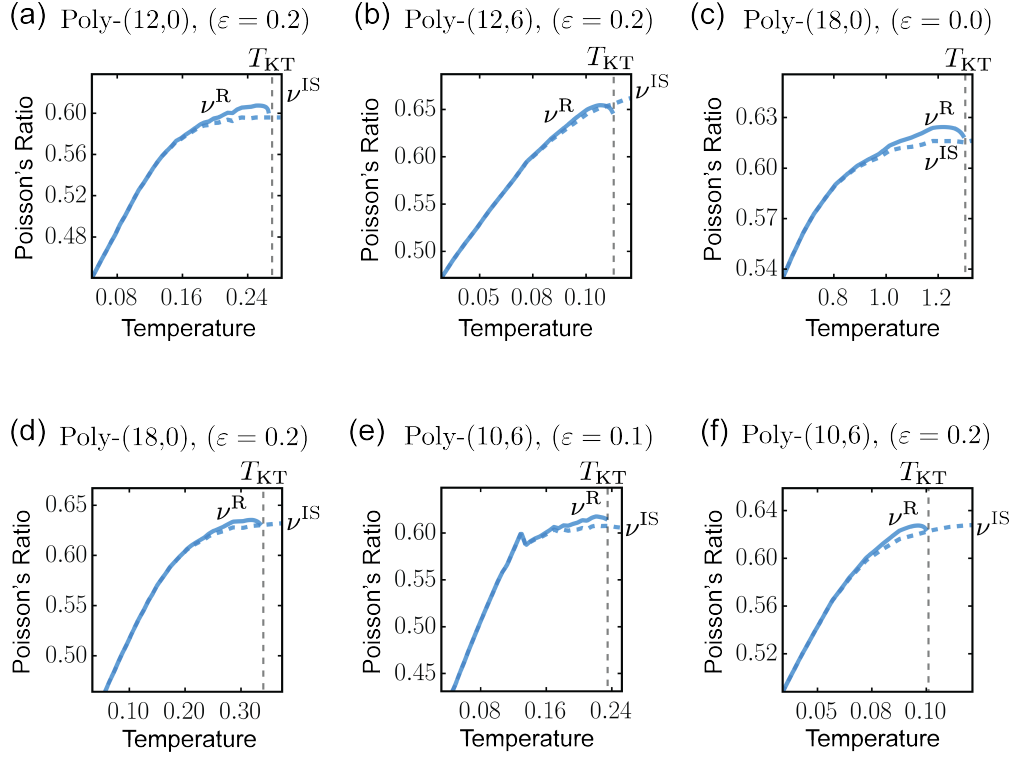

Figure S.22: The bare inherent-state Poisson's ratio in comparison to the renormalized Poisson's ratio for six model atomistic glass formers. In all cases, the renormalized value is close to the inherent state one.

fluctuations that are dynamically probed at timescales  $t \sim \langle \tau_{\text{jump}} \rangle \ll \tau_{\text{eq}}$ , we expect that the elastic and Gaussian correlations are measurable in the displacement and density correlation functions for relaxation at those intermediate timescales. Such functions include the mean-squared displacement (MSD)  $\langle |\mathbf{u}^\alpha(t)|^2 \rangle$ , and the self-part of the intermediate scattering function  $F_s(\mathbf{k}, t)$ .

In this section we investigate the consequences of both the elastic and two-dimensional nature of these fluctuations on the MSD and density-density correlations. We start with the effective Hamiltonian in Eq. (5.173) and apply the stiffness tensor for an isotropic solid (Eq. (2.14)) to obtain

$$\mathcal{H}_{\text{eff}} = \int d^2\mathbf{x} G^{\text{R}} \left( \epsilon_{ij} \epsilon_{ij} + \frac{\nu^{\text{R}}}{1 - \nu^{\text{R}}} \epsilon_{kk} \epsilon_{nn} \right). \quad (5.174)$$

To study correlations, it is convenient to switch to Fourier space and express  $\epsilon_{ij} = \frac{1}{2} (u_{i,j} + u_{j,i})$ , in terms of its Fourier transform  $\epsilon_{ij}(\mathbf{k}) = \frac{i}{2} (k_i u_j(\mathbf{k}) + k_j u_i(\mathbf{k}))$ . This turns Eq. (5.174) into

$$\mathcal{H}_{\text{eff}} = \int \frac{d^2\mathbf{k}}{(2\pi)^2} G^{\text{R}} \left( \epsilon_{ij}(\mathbf{k}) \epsilon_{ij}(-\mathbf{k}) + \frac{\nu^{\text{R}}}{1 - \nu^{\text{R}}} \epsilon_{kk}(\mathbf{k}) \epsilon_{nn}(-\mathbf{k}) \right) \quad (5.175)$$

$$= \int \frac{d^2\mathbf{k}}{(2\pi)^2} G^{\text{R}} \left[ \frac{1}{4} (k_i u_j(\mathbf{k}) + k_j u_i(\mathbf{k})) (k_i u_j(-\mathbf{k}) + k_j u_i(\mathbf{k})) + \frac{\nu^{\text{R}}}{1 - \nu^{\text{R}}} k_i u_i(\mathbf{k}) k_j u_j(-\mathbf{k}) \right] \quad (5.176)$$

$$= \frac{1}{2} \int \frac{d^2\mathbf{k}}{(2\pi)^2} G^{\text{R}} \left[ k^2 \delta_{ij} + \left( \frac{1 + \nu^{\text{R}}}{1 - \nu^{\text{R}}} \right) k_i k_j \right] u_i(\mathbf{k}) u_j(-\mathbf{k}) \quad (5.177)$$

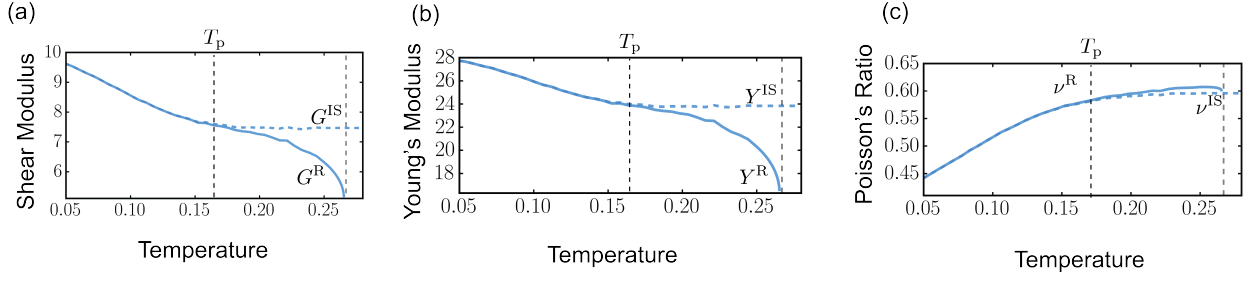

Figure S.23: Comparison of inherent-state and renormalized elastic moduli, the convergence of the renormalized values to their bare values as  $T \rightarrow T_p$ . (a) Shear modulus (b) Young's modulus, (c) Poisson's ratio. All data corresponds to the renormalized shear modulus for the Poly-(12,0) model glass former.

$$\equiv \frac{1}{2} \int \frac{d^2 \mathbf{k}}{(2\pi)^2} u_i(\mathbf{k}) M_{ij}(\mathbf{k}) u_j(-\mathbf{k}), \quad (5.178)$$

where  $M_{ij}(\mathbf{k})$  is a matrix kernel that controls the inverse of the covariance function in displacements

$$M_{ij}(\mathbf{k}) = G^R \left[ k^2 \delta_{ij} + \left( \frac{1 + \nu^R}{1 - \nu^R} \right) k_i k_j \right]. \quad (5.179)$$

Equation (5.178) leads to interaction between displacements in  $\mathbf{k}$ -space that are Gaussian in nature, and thus allows us to conclude that

$$\langle u_i(\mathbf{k}) u_j(\mathbf{k}') \rangle = (2\pi)^2 \delta(\mathbf{k} + \mathbf{k}') k_B T M_{ij}^{-1}(\mathbf{k}). \quad (5.180)$$

where the inverse  $M_{ij}^{-1}$  is defined as

$$M_{ij}^{-1}(\mathbf{k}) M_{jk}(\mathbf{k}) = \delta_{ik}. \quad (5.181)$$

Suppose that the inverse follows the same form as  $M_{ij}(\mathbf{k})$ , namely  $M_{ij}^{-1} = A(\mathbf{k}) \delta_{ij} + B(\mathbf{k}) k_i k_j$ , where  $A(\mathbf{k})$  and  $B(\mathbf{k})$  are functions to be determined. Substituting this ansatz into Eq. (5.181) yields an equation,

$$(G^R k^2 A(\mathbf{k})) \delta_{ik} + \left( G^R \left( \frac{1 + \nu^R}{1 - \nu^R} \right) A(\mathbf{k}) + G^R k^2 B(\mathbf{k}) + \left( \frac{1 + \nu^R}{1 - \nu^R} \right) k^2 B(\mathbf{k}) \right) k_i k_k = \delta_{ik}, \quad (5.182)$$

which is satisfied when

$$G^R \left( \frac{1 + \nu^R}{1 - \nu^R} \right) A(\mathbf{k}) = 1, \quad G^R \left( \frac{1 + \nu^R}{1 - \nu^R} \right) A(\mathbf{k}) + G^R k^2 B(\mathbf{k}) + \left( \frac{1 + \nu^R}{1 - \nu^R} \right) k^2 B(\mathbf{k}) = 0. \quad (5.183)$$

Solving for  $A(\mathbf{k})$  and  $B(\mathbf{k})$  we find that

$$A(\mathbf{k}) = \frac{1}{G^R k^2}, \quad B(\mathbf{k}) = -\frac{1 + \nu^R}{2 G^R} \frac{1}{k^4}, \quad (5.184)$$

leading to

$$M_{ij}^{-1}(\mathbf{k}) = \frac{1}{G^R k^2} \left( \delta_{ij} - \frac{1 + \nu^R}{2} \frac{k_i k_j}{k^2} \right) \quad (5.185)$$

and using Eq. (5.180), we obtain the final form of the displacement correlation function

$$\langle u_i(\mathbf{k}) u_j(\mathbf{k}') \rangle = \frac{(2\pi)^2 k_B T}{G^R k^2} \delta(\mathbf{k} + \mathbf{k}') \left( \delta_{ij} - \frac{1 + \nu^R}{2} \frac{k_i k_j}{k^2} \right). \quad (5.186)$$

The displacement correlation function in Eq. (5.186) forms the basis behind all possible correlations we want to understand in a supercooled liquid at timescales  $t \sim \langle \tau_{\text{jump}} \rangle \ll \tau_{\text{eq}}$ . The use of renormalized elastic moduli, e.g.  $G^{\text{R}}$  and  $\nu^{\text{R}}$ , implies that the correlations we compute already accounts for the rare localized excitation events that are present within those timescales, simplifying the calculation to an application of Gaussian statistics. For instance, consider the MSD as given by

$$\langle |\mathbf{u}(t)|^2 \rangle = \frac{1}{N} \sum_{\alpha=1}^N \langle |\mathbf{u}^{\alpha}(t)|^2 \rangle \quad (5.187)$$

At  $t \simeq \tau_{\text{jump}}$ , we expect that the MSD can also be computed from the spatial average of displacement field fluctuation,

$$\langle |\mathbf{u}(\langle \tau_{\text{jump}} \rangle)|^2 \rangle \approx \frac{1}{A_0} \int d^2 \mathbf{x} \langle |\mathbf{u}(\mathbf{x})|^2 \rangle. \quad (5.188)$$

The mean-squared displacement in the integral of Eq. (5.188) is obtained by taking the inverse Fourier transform of Eq. (5.186). In particular,

$$\begin{aligned} \langle |\mathbf{u}(\mathbf{x})|^2 \rangle &= \int \frac{d^2 \mathbf{k}}{(2\pi)^2} \frac{d^2 \mathbf{k}'}{(2\pi)^2} \langle u_i(\mathbf{k}) u_i(\mathbf{k}') \rangle e^{i(\mathbf{k}+\mathbf{k}') \cdot \mathbf{x}} \\ &= \int \frac{d^2 \mathbf{k}}{(2\pi)^2} \frac{d^2 \mathbf{k}'}{(2\pi)^2} (2\pi)^2 \delta(\mathbf{k} + \mathbf{k}') k_{\text{B}} T M_{ii}^{-1}(\mathbf{k}) e^{i(\mathbf{k}+\mathbf{k}') \cdot \mathbf{x}} \\ &= \int \frac{d^2 \mathbf{k}}{(2\pi)^2} k_{\text{B}} T M_{ii}^{-1}(\mathbf{k}), \end{aligned} \quad (5.189)$$

and from Eq. (5.185), we obtain

$$\langle |\mathbf{u}(\langle \tau_{\text{jump}} \rangle)|^2 \rangle \approx \int \frac{d^2 \mathbf{k}}{(2\pi)^2} k_{\text{B}} T M_{ii}^{-1}(\mathbf{k}) = \int \frac{d^2 \mathbf{k}}{(2\pi)^2} \frac{k_{\text{B}} T}{G^{\text{R}} k^2} \left( \delta_{ii} - \frac{1 + \nu^{\text{R}}}{2} \frac{k_i k_i}{k^2} \right) \quad (5.190)$$

$$= k_{\text{B}} T \frac{3 - \nu^{\text{R}}}{2 G^{\text{R}}} \int \frac{d^2 \mathbf{k}}{(2\pi)^2} \frac{1}{k^2}, \quad (5.191)$$

where use is made of the trace of Eq. (5.185) to obtain the second equality. Switching to polar coordinates in Fourier space, we have

$$\langle |\mathbf{u}(\langle \tau_{\text{jump}} \rangle)|^2 \rangle \approx k_{\text{B}} T \frac{3 - \nu^{\text{R}}}{2 G^{\text{R}} (2\pi)^2} \int_{2\pi/\xi^*}^{2\pi/R} dk \int_0^{2\pi} d\phi \frac{1}{k} = k_{\text{B}} T \frac{3 - \nu^{\text{R}}}{4\pi G^{\text{R}}} \ln \frac{R}{\xi^*}. \quad (5.192)$$

Using the definition for the Young's modulus,  $Y = 2G(1 + \nu)$ , we obtain

$$\langle |\mathbf{u}(\langle \tau_{\text{jump}} \rangle)|^2 \rangle \approx k_{\text{B}} T \frac{(3 - \nu^{\text{R}})(1 + \nu^{\text{R}})}{2\pi Y^{\text{R}}} \ln \frac{R}{\xi^*}. \quad (5.193)$$

At sufficiently low temperatures,  $\xi^* \sim \mathcal{O}(a_{\text{dpl}})$  and the renormalized elastic moduli converge to their bare values. Thus, most of the temperature dependence comes from the prefactor of the logarithm, and the dominant scaling behavior is  $\langle |\mathbf{u}(\langle \tau_{\text{jump}} \rangle)|^2 \rangle \sim \ln R$ . The logarithmic increase of MSD at the intermediate timescales also implies that relaxation becomes faster as the system gets larger. This observation was recently confirmed in computer simulations, where the elastic fluctuations were also called Mermin-Wagner fluctuations [12–16]. We adapted the MSD from Ref. [14] and demonstrate its logarithmic scaling in Fig. S.24(a). See also Fig. 4(d) of the main text for a demonstration of the logarithmic scaling for a 2D Kob-Andersen model [45, 46].

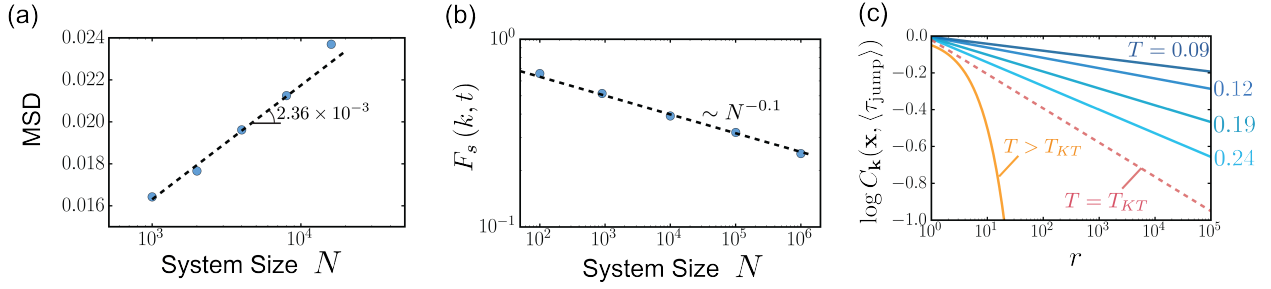

Figure S.24: Summary of displacement and density correlations at low temperatures and intermediate timescales  $t \simeq \tau_{\text{jump}}$  according to our theory: (a) logarithmic scaling of mean-squared displacement, (b) power-law scaling of  $F_s(k, t)$ , and (c) power-law spatial correlations in the order parameter. Note that the data of the first two were adapted from Ref. [12] and [14], respectively.

Our conclusion on the MSD also translates to the self-part of the intermediate scattering function  $F_s(\mathbf{k}, t)$ , which is defined as

$$F_s(\mathbf{k}, t) = \left\langle \frac{1}{N} \sum_{\alpha=1}^N e^{i\mathbf{k} \cdot \mathbf{u}^\alpha(t)} \right\rangle. \quad (5.194)$$

At the intermediate timescale  $t \simeq \tau_{\text{jump}}$ , the displacement at every point in space, and thus of every particle, is Gaussian for wavenumbers  $k \in [0, 2\pi/\xi^*]$  according to the effective field theory. Since  $F_s(\mathbf{k}, t)$  is a characteristic or cumulant-generating function for the particle displacement fluctuations [47], we can use the characteristic function for a Gaussian distribution to write Eq. (5.194) as

$$F_s(\mathbf{k}, \langle \tau_{\text{jump}} \rangle) \approx e^{-\frac{k^2}{2d} \langle |\mathbf{u}^\alpha(\langle \tau_{\text{jump}} \rangle)|^2 \rangle}, \quad (5.195)$$

where  $d = 2$  for two dimensions. Substituting Eq. (5.193) then yields

$$F_s(k, \langle \tau_{\text{jump}} \rangle) \approx \exp \left( -k_B T \frac{k^2 (3 - \nu^R)(1 + \nu^R)}{8\pi Y^R} \ln \frac{R}{\xi^*} \right) = \left( \frac{R}{\xi^*} \right)^{-\frac{\sigma(k, T)}{2}}, \quad (5.196)$$

where  $\sigma(k, T)$  is a power-law exponent

$$\sigma(k, T) = k_B T \frac{k^2 (3 - \nu^R)(1 + \nu^R)}{4\pi Y^R}. \quad (5.197)$$

At very low temperatures,  $\xi^* \sim \mathcal{O}(a_{\text{dpl}}) \sim \mathcal{O}(\sigma_d)$ , where  $\sigma_d$  is the particle diameter, which implies that the lengthscales in which we measure relaxation coincides with the lengthscales for elastic Gaussian fluctuations. This results in the decrease of  $F_s(k, \tau_{\text{jump}})$  as the system gets larger; a phenomenon that has been observed in recent computer simulations [12]. We further adapted the data in Ref. [12], choosing  $t = 100$  as the intermediate timescale, and demonstrate that the power-law scaling exists in Fig. S.24(b). See also Fig. 4(e) of the main text where we also show the power-law scaling for the same 2D Kob-Andersen model used in the MSD scaling of Fig. 4(d). There, the data is also taken at the same temperature, and thus we are able to validate that the exponents derived from either MSD or  $F_s(k, t)$  are consistent with each other.

Correlations in elastic fluctuations can also be studied spatially. To see this, we compute a displacement field  $\mathbf{u}(\mathbf{x}, t)$  from the particle displacements  $\mathbf{u}^\alpha(t) = \mathbf{r}^\alpha(t) - \mathbf{R}_0^\alpha$  using the initial inherent state  $\{\mathbf{R}_0^\alpha\}$  as a reference configuration. This yields,

$$\mathbf{u}(\mathbf{x}, t) = \sum_{\alpha=1}^N \mathbf{u}^\alpha(t) \hat{N}_\alpha(\mathbf{x}), \quad (5.198)$$

where  $\hat{N}_\alpha(\mathbf{x})$  is an interpolating function such that  $\hat{N}_\alpha(\mathbf{R}_0^\beta) = \delta_{\alpha\beta}$  [7]. Using the displacement field, we define an order parameter field

$$\rho_{\mathbf{k}}(\mathbf{x}) = e^{i\mathbf{k} \cdot \mathbf{u}(\mathbf{x}, t)}, \quad (5.199)$$

where the value of  $\mathbf{k} \in [0, 2\pi/\xi^*]$ . The spatial correlations we want to study corresponds to the following correlation function evaluated at  $t \simeq \langle \tau_{\text{jump}} \rangle$ :

$$C_{\mathbf{k}}(\mathbf{x}, \langle \tau_{\text{jump}} \rangle) = \langle \rho_{\mathbf{k}}(\mathbf{x}, \langle \tau_{\text{jump}} \rangle) \rho_{-\mathbf{k}}(\mathbf{0}, 0) \rangle = \left\langle e^{i\mathbf{k} \cdot (\mathbf{u}(\mathbf{x}, \langle \tau_{\text{jump}} \rangle) - \mathbf{u}(\mathbf{0}, 0))} \right\rangle. \quad (5.200)$$

At these timescales, the displacement field, and thereby the correlation function, is also governed by the elastic Gaussian field theory. Furthermore, Eq. (5.200) defines a characteristic function like  $F_s(k, t)$ , and thus we can write the correlation function as

$$C_{\mathbf{k}}(\mathbf{x}, \langle \tau_{\text{jump}} \rangle) = \exp \left( -\frac{\mathbf{k} \otimes \mathbf{k}}{2} : \langle (\mathbf{u}(\mathbf{x}) - \mathbf{u}(\mathbf{0})) \otimes (\mathbf{u}(\mathbf{x}) - \mathbf{u}(\mathbf{0})) \rangle \right) \quad (5.201)$$

$$= \exp \left( -\frac{k_i k_j}{2} \int \frac{d\mathbf{k}'}{(2\pi)^2} \frac{d\mathbf{k}''}{(2\pi)^2} \left( e^{i\mathbf{k}' \cdot \mathbf{x}} - 1 \right) \left( e^{i\mathbf{k}'' \cdot \mathbf{x}} - 1 \right) \langle u_i(\mathbf{k}') u_j(\mathbf{k}'') \rangle \right) \quad (5.202)$$

$$= \exp \left( - \int \frac{d\mathbf{k}'}{(2\pi)^2} (1 - \cos(\mathbf{k}' \cdot \mathbf{x})) \frac{k_B T (1 + \nu^R)}{2Y^R k'^2} \left( k^2 - \frac{1 + \nu^R}{2} \frac{(\mathbf{k} \cdot \mathbf{k}')^2}{k'^2} \right) \right). \quad (5.203)$$

To evaluate the last equality, we may use the approximation  $(\mathbf{k} \cdot \mathbf{k}')^2 \simeq \frac{k^2 k'^2}{2}$  to simplify the angular average [48], giving us

$$C_{\mathbf{k}}(\mathbf{x}, \langle \tau_{\text{jump}} \rangle) \simeq \exp \left( -k_B T \frac{k^2 (3 - \nu^R) (1 + \nu^R)}{4\pi Y^R} \ln \left( \frac{|\mathbf{x}|}{R} \right) \right) = \left( \frac{|\mathbf{x}|}{R} \right)^{-\sigma(k, T)}. \quad (5.204)$$

Equation (5.204) thus implies for any temperatures lower than  $T_{\text{KT}}$ , the system exhibits power-law spatial correlations, as anticipated in the end of Section 5.3. These power-law correlations should persist all the way to  $T \rightarrow T_{\text{KT}}$ , but above these temperatures, one expects an exponential decay in correlations, as shown in Fig. S.24(c) for the Poly-(12,0) model glass former.

## References

- [1] Widmer-Cooper, A., Harrowell, P. & Fynewever, H. How reproducible are dynamic heterogeneities in a supercooled liquid? *Phys. Rev. Lett.* **93**, 135701 (2004).
- [2] Chandler, D. & Garrahan, J. P. Dynamics on the way to forming glass: Bubbles in space-time. *Annu. Rev. Phys. Chem.* **61**, 191–217 (2010).
- [3] Moshe, M., Sharon, E. & Kupferman, R. Elastic interactions between two-dimensional geometric defects. *Phys. Rev. E* **92**, 062403 (2015).
- [4] Moshe, M., Levin, I., Aharoni, H., Kupferman, R. & Sharon, E. Geometry and mechanics of two-dimensional defects in amorphous materials. *Proc. Natl. Acad. Sci. U.S.A.* **112**, 10873–10878 (2015).
- [5] Kosterlitz, J. M. & Thouless, D. J. Long range order and metastability in two dimensional solids and superfluids. (application of dislocation theory). *J. Phys. C: Solid State Phys.* **5**, L124 (1972).
- [6] Kosterlitz, J. M. & Thouless, D. J. Ordering, metastability and phase transitions in two-dimensional systems. *J. Phys. C: Solid State Phys.* **6**, 1181 (1973).
- [7] Hasyim, M. R. & Mandadapu, K. K. A theory of localized excitations in supercooled liquids. *J. Chem. Phys.* **155**, 044504 (2021).
- [8] Halperin, B. & Nelson, D. R. Theory of two-dimensional melting. *Phys. Rev. Lett.* **41**, 121 (1978).
- [9] Nelson, D. R. Study of melting in two dimensions. *Phys. Rev. B* **18**, 2318 (1978).
- [10] Nelson, D. R. & Halperin, B. Dislocation-mediated melting in two dimensions. *Phys. Rev. B* **19**, 2457 (1979).
- [11] Young, A. Melting and the vector Coulomb gas in two dimensions. *Phys. Rev. B* **19**, 1855 (1979).
- [12] Flenner, E. & Szamel, G. Fundamental differences between glassy dynamics in two and three dimensions. *Nat. Comm.* **6**, 1–6 (2015).
- [13] Shiba, H., Yamada, Y., Kawasaki, T. & Kim, K. Unveiling dimensionality dependence of glassy dynamics: 2d infinite fluctuation eclipses inherent structural relaxation. *Phys. Rev. Lett.* **117**, 245701 (2016).
- [14] Illing, B. *et al.* Mermin–Wagner fluctuations in 2d amorphous solids. *Proc. Natl. Acad. Sci. U.S.A.* **114**, 1856–1861 (2017).
- [15] Vivek, S., Kelleher, C. P., Chaikin, P. M. & Weeks, E. R. Long-wavelength fluctuations and the glass transition in two dimensions and three dimensions. *Proc. Natl. Acad. Sci. U.S.A.* **114**, 1850–1855 (2017).
- [16] Tarjus, G. Glass transitions may be similar in two and three dimensions, after all. *Proc. Natl. Acad. Sci. U.S.A.* **114**, 2440–2442 (2017).

- [17] Chandler, D. Statistical mechanics of isomerization dynamics in liquids and the transition state approximation. *J. Chem. Phys.* **68**, 2959–2970 (1978).
- [18] Peters, B. *Reaction Rate Theory and Rare Events* (Elsevier, 2017).
- [19] Karmakar, S., Lerner, E. & Procaccia, I. Athermal nonlinear elastic constants of amorphous solids. *Phys. Rev. E* **82**, 026105 (2010).
- [20] Lutsko, J. Generalized expressions for the calculation of elastic constants by computer simulation. *J. App. Phys.* **65**, 2991–2997 (1989).
- [21] Stillinger, F. H. & Weber, T. A. Hidden structure in liquids. *Phys. Rev. A* **25**, 978 (1982).
- [22] Chandler, D. *Introduction to Modern Statistical Mechanics* (Oxford University Press, 1987).
- [23] Hansen, J.-P. & McDonald, I. R. *Theory of Simple Liquids* (Academic Press, 2005).
- [24] Keys, A. S., Hedges, L. O., Garrahan, J. P., Glotzer, S. C. & Chandler, D. Excitations are localized and relaxation is hierarchical in glass-forming liquids. *Phys. Rev. X* **1**, 021013 (2011).
- [25] Garrahan, J. P. & Chandler, D. Coarse-grained microscopic model of glass formers. *Proc. Natl. Acad. Sci. U.S.A.* **100**, 9710–4 (2003).
- [26] Ritort, F. & Sollich, P. Glassy dynamics of kinetically constrained models. *Adv. Phys.* **52**, 219–342 (2003).
- [27] Sollich, P. & Evans, M. R. Glassy time-scale divergence and anomalous coarsening in a kinetically constrained spin chain. *Phys. Rev. Lett.* **83**, 3238–3241 (1999).
- [28] Sollich, P. & Evans, M. R. Glassy dynamics in the asymmetrically constrained kinetic Ising chain. *Phys. Rev. E* **68**, 031504 (2003).
- [29] Johnson, A. M. Dislocations Disclinations and Displacement Discontinuity Boundary Elements for Isotropic, Anisotropic, Nonlinear Solids and Fluids. <https://engineering.purdue.edu/~ce597m> (2005).
- [30] Kroner, E. & Anthony, K. Dislocations and disclinations in material structures: The basic topological concepts. *Annu. Rev. Mater. Sci.* **5**, 43–72 (1975).
- [31] Chaikin, P. M., Lubensky, T. C. & Witten, T. A. *Principles of Condensed Matter Physics*, vol. 10 (Cambridge University Press, 1995).
- [32] Balluffi, R. W. *Introduction to Elasticity Theory for Crystal Defects* (Cambridge University Press, 2012).
- [33] Papadopoulos, P. ME 280A: Introduction to the Finite Element Method. <https://csm1.berkeley.edu/Notes/ME280A.pdf> (2015).
- [34] Seung, H. S. & Nelson, D. R. Defects in flexible membranes with crystalline order. *Phys. Rev. A* **38**, 1005 (1988).
- [35] Goldenfeld, N. *Lectures on Phase Transitions and the Renormalization Group* (CRC Press, 2018).

- [36] Amit, D. J. & Martin-Mayor, V. *Field Theory, the Renormalization Group, and Critical Phenomena: Graphs to Computers* (World Scientific, 2005).
- [37] Zwanzig, R. W. High-temperature equation of state by a perturbation method. I. Nonpolar gases. *J. Chem. Phys.* **22**, 1420–1426 (1954).
- [38] Kleinert, H. *Multivalued Fields in Condensed Matter, Electromagnetism, And Gravitation* (World Scientific, 2008).
- [39] Ninarello, A., Berthier, L. & Coslovich, D. Models and algorithms for the next generation of glass transition studies. *Phys. Rev. X* **7**, 021039 (2017).
- [40] Anderson, J. A., Glaser, J. & Glotzer, S. C. HOOMD-blue: A Python package for high-performance molecular dynamics and hard particle monte carlo simulations. *Comput. Mater. Sci* **173**, 109363 (2020).
- [41] Bitzek, E., Koskinen, P., Gähler, F., Moseler, M. & Gumbusch, P. Structural relaxation made simple. *Phys. Rev. Lett.* **97**, 170201 (2006).
- [42] Lutsko, J. Stress and elastic constants in anisotropic solids: Molecular dynamics techniques. *J. App. Phys.* **64**, 1152–1154 (1988).
- [43] Hernandez, V., Roman, J. E. & Vidal, V. SLEPc: A scalable and flexible toolkit for the solution of eigenvalue problems. *ACM Trans. Math. Softw.* **31**, 351–362 (2005).
- [44] Chodera, J. D., Swope, W. C., Pitera, J. W., Seok, C. & Dill, K. A. Use of the weighted histogram analysis method for the analysis of simulated and parallel tempering simulations. *J. Chem. Theory Comput.* **3**, 26–41 (2007).
- [45] Kob, W. & Andersen, H. C. Testing mode-coupling theory for a supercooled binary Lennard-Jones mixture I: The van Hove correlation function. *Phys. Rev. E* **51**, 4626 (1995).
- [46] Shiba, H., Kawasaki, T. & Kim, K. Local density fluctuation governs the divergence of viscosity underlying elastic and hydrodynamic anomalies in a 2d glass-forming liquid. *Phys. Rev. Lett.* **123**, 265501 (2019).
- [47] Boon, J. P. & Yip, S. *Molecular Hydrodynamics*, chap. 4, 171–178 (Courier Corporation, 1991).
- [48] Kardar, M. *Statistical Physics of Fields* (Cambridge University Press, 2007).
